# Supplementary material for: The SAMI Galaxy Survey: rules of behaviour for spin-ellipticity radial tracks in galaxies
Source: arXiv:1910.01358 ancillary file (2019-10-04)

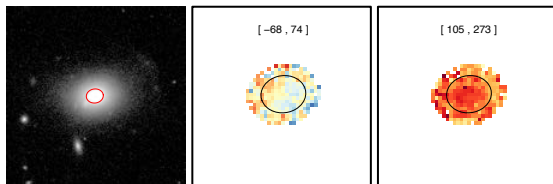

SAMI7289 (KiDS): \*E

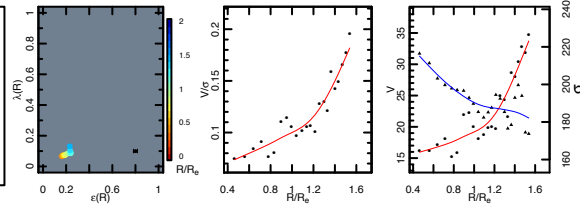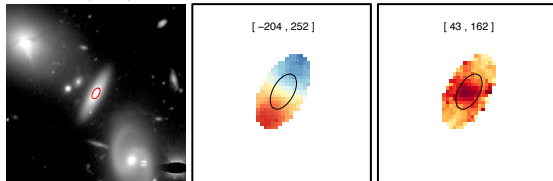

SAMI7841 (HSC): \*S0

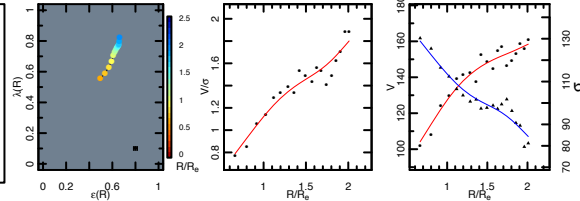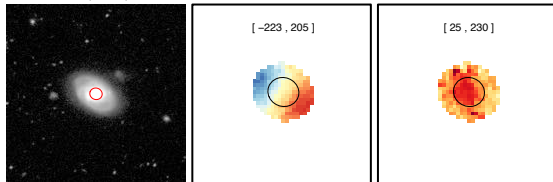

SAMI7946 (HSC): eSp

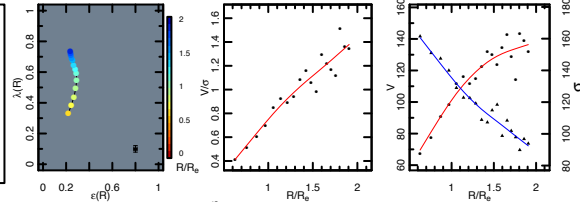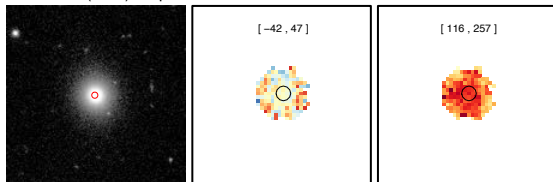

SAMI8865 (KiDS): E

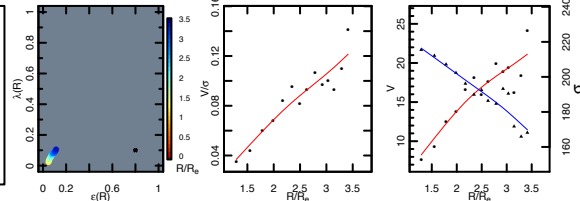

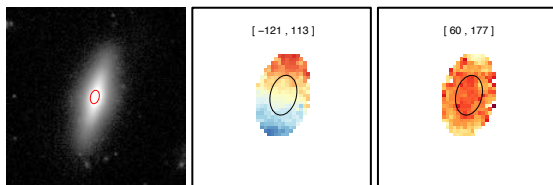

SAMI9062 (KiDS): S0

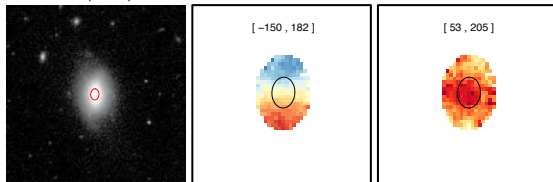

SAMI14552 (KiDS): S0

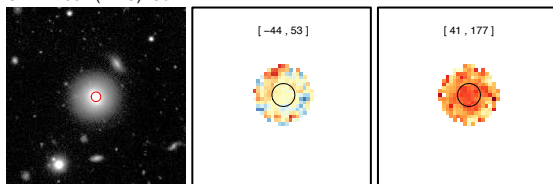

SAMI16022 (HSC): \*E

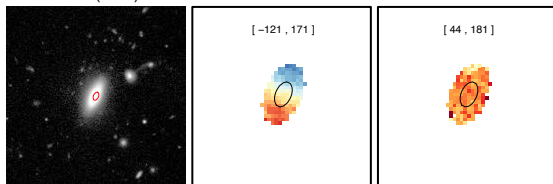

SAMI16026 (HSC): eSp/ISp

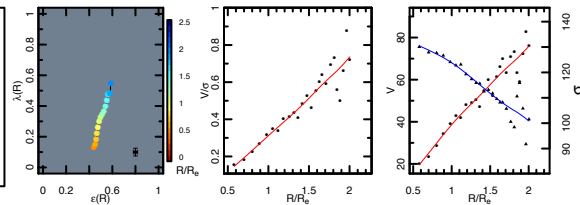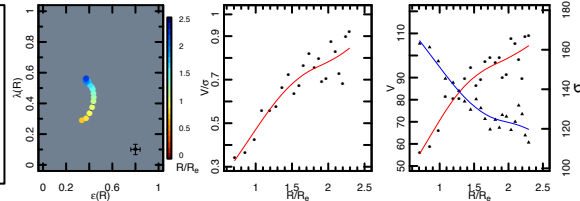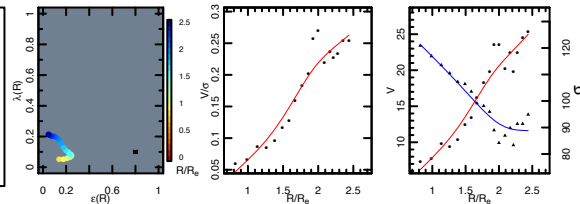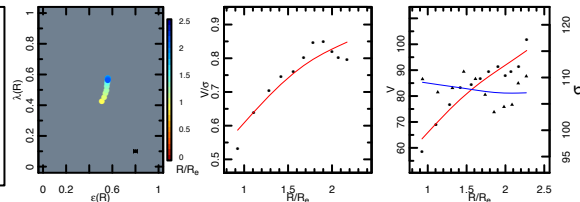

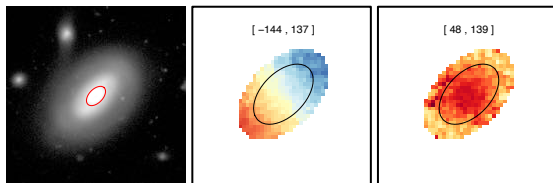

SAMI16317 (HSC): S0

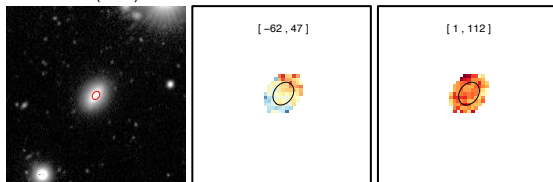

SAMI16429 (HSC): ?

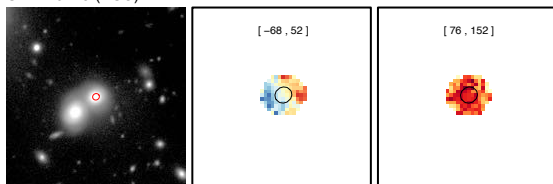

SAMI16525 (HSC): E

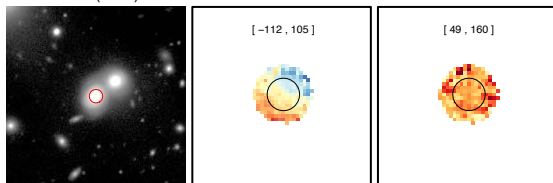

SAMI16526 (HSC): E

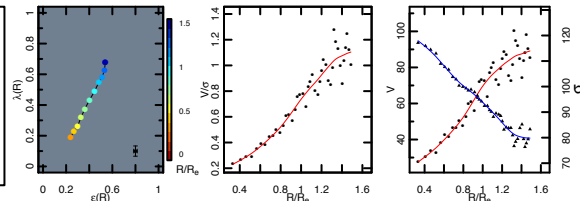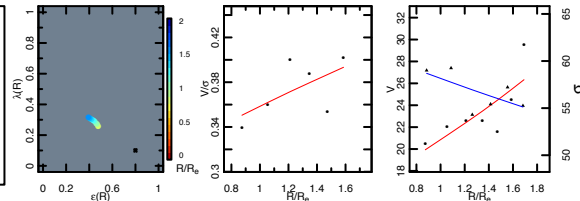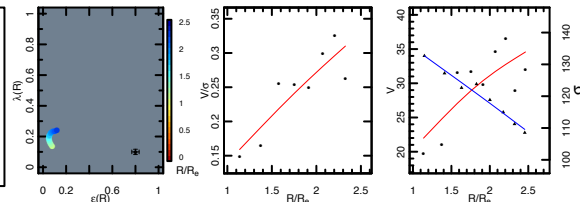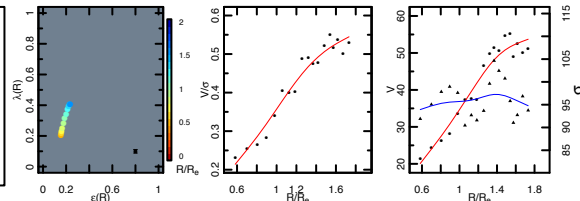

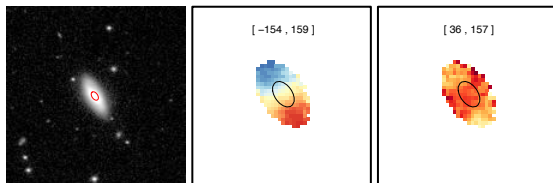

SAMI16926 (KiDS): S0

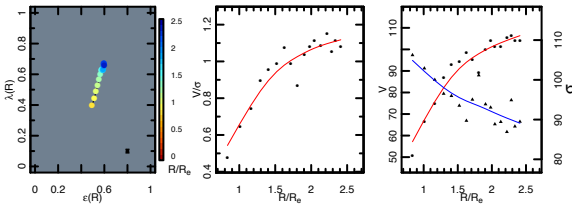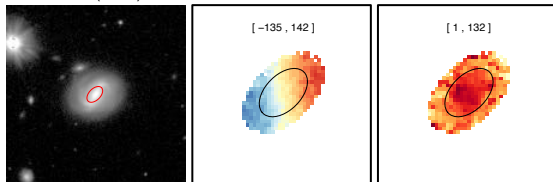

SAMI17314 (KiDS): \*eSB

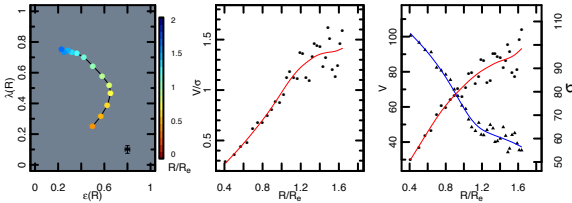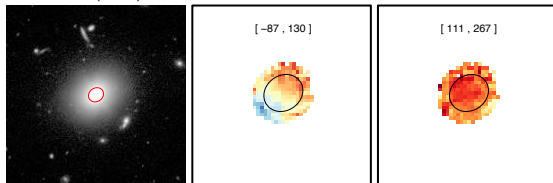

SAMI22582 (HSC): \*E

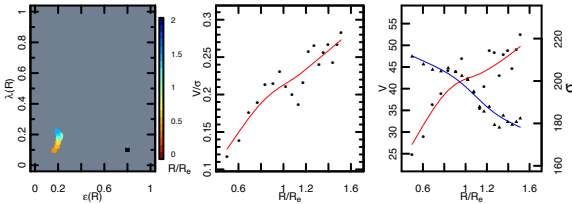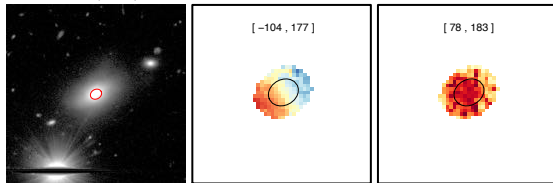

SAMI23070 (HSC): S0

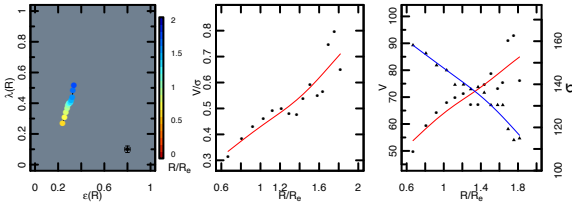

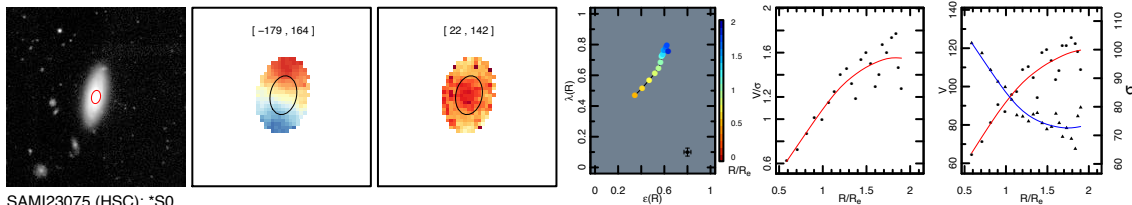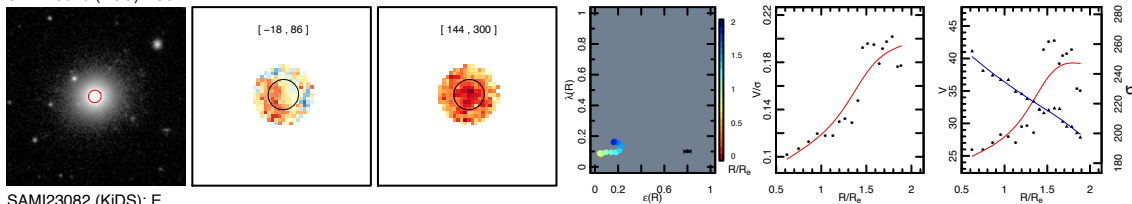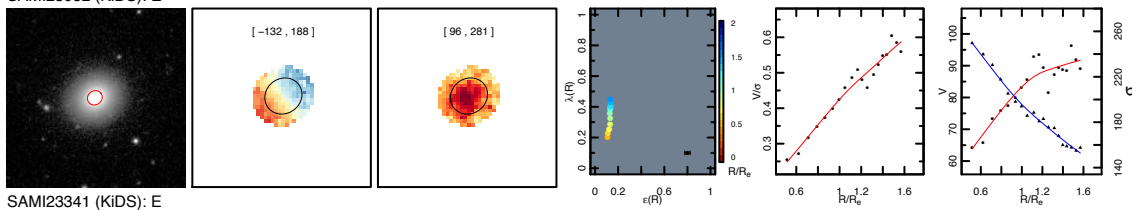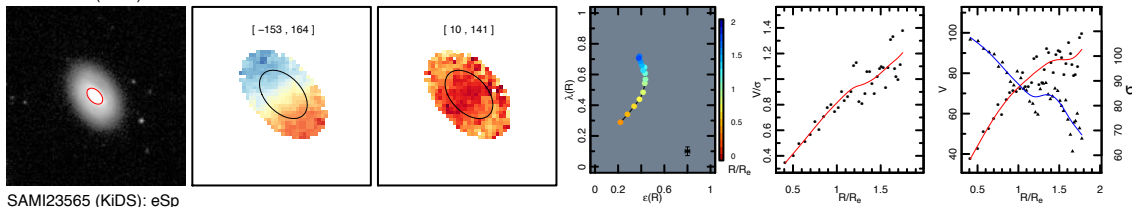

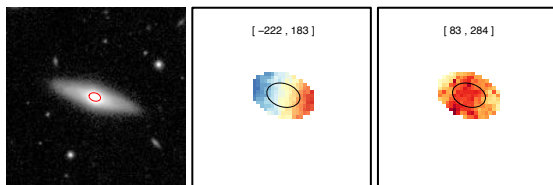

SAMI23619 (KiDS): \*S0

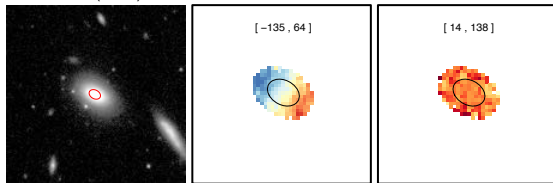

SAMI28738 (KiDS): lSp

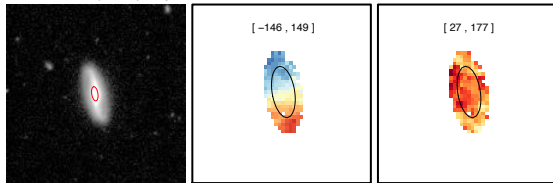

SAMI30786 (KiDS): eSp

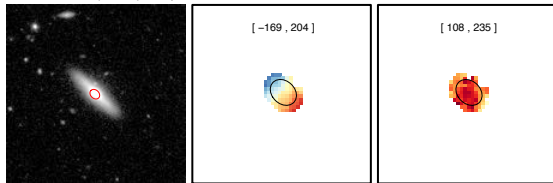

SAMI31912 (KiDS): \*S0

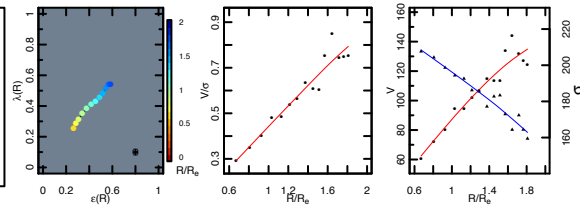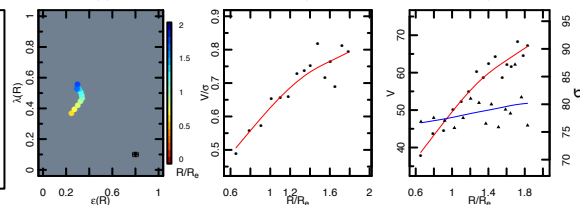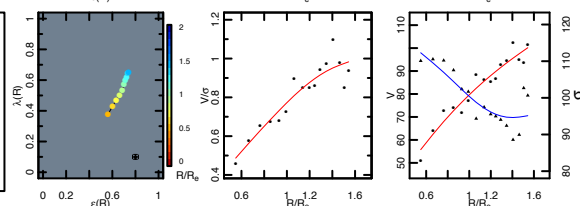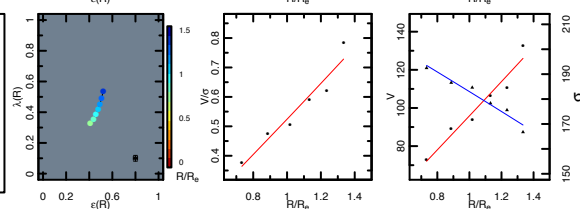

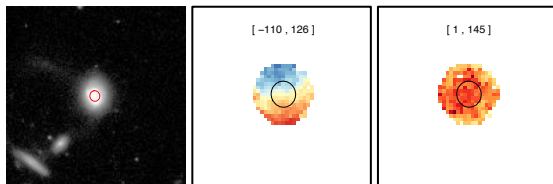

SAMI39145 (KiDS): \*ISp

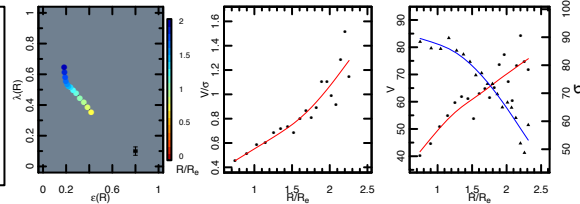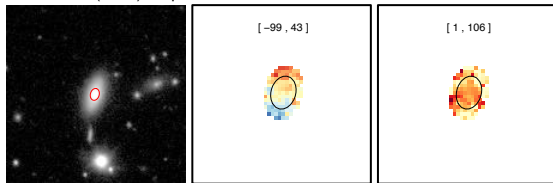

SAMI39365 (KiDS): eSp

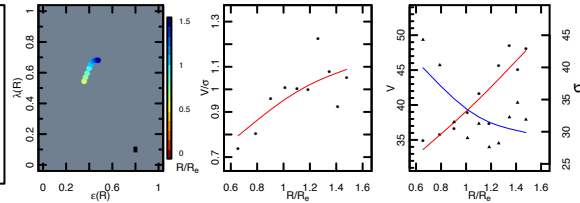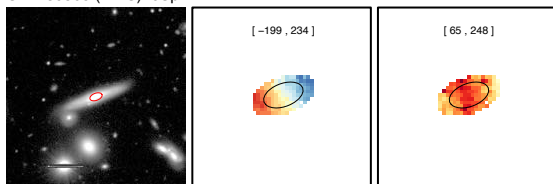

SAMI39709 (HSC): \*SO

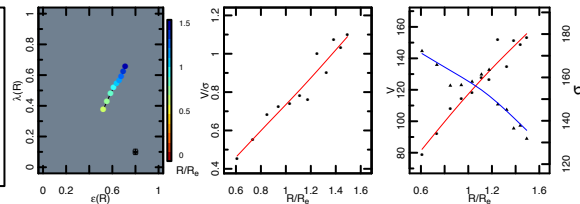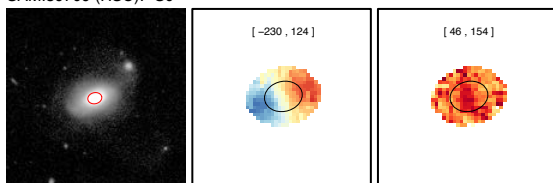

SAMI40164 (KiDS): \*Merger

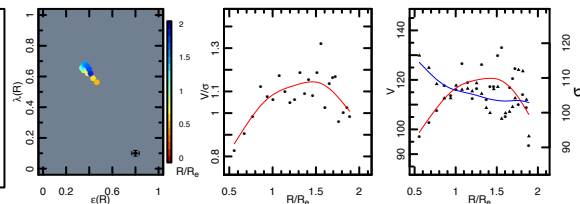

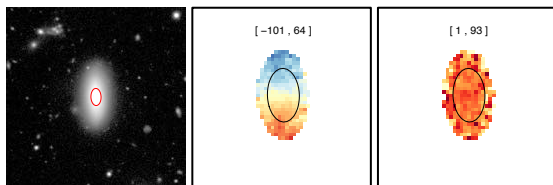

SAMI40197 (HSC): S0/eSp

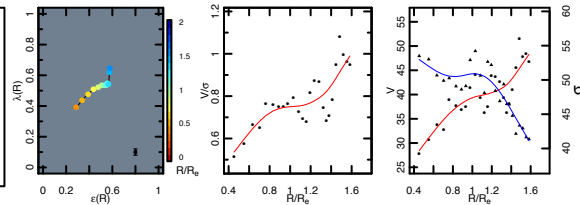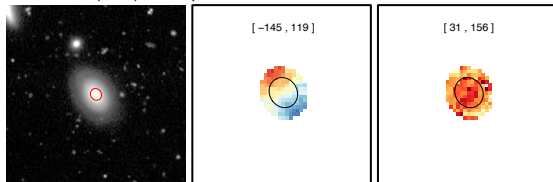

SAMI40491 (HSC): \*S0

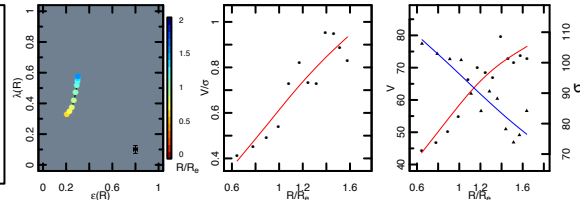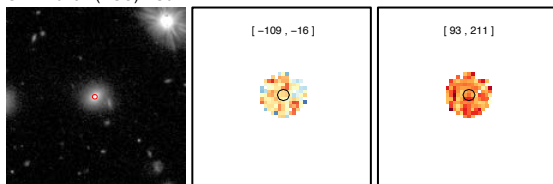

SAMI41180 (KiDS): E

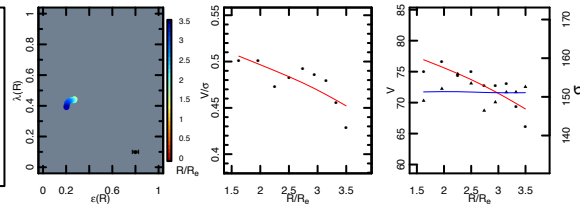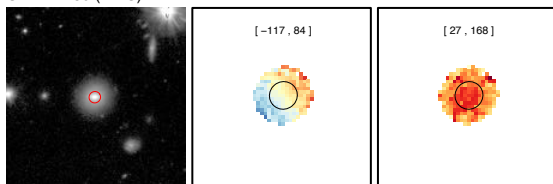

SAMI41274 (KiDS): E/S0

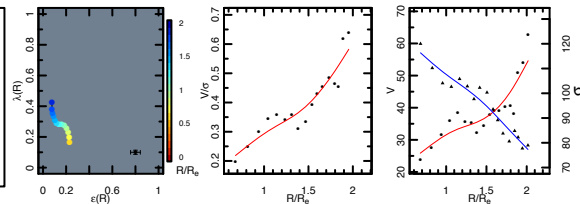



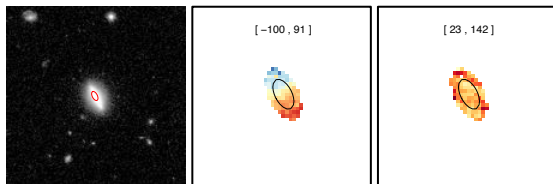

SAMI41302 (KiDS): S0/eSp

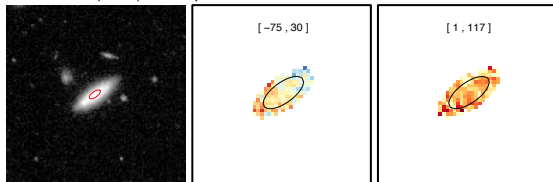

SAMI41354 (KiDS): lSp

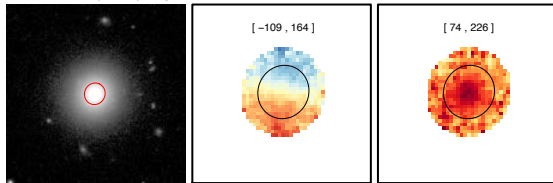

SAMI47254 (KiDS): E

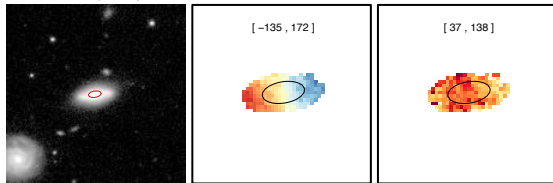

SAMI47258 (KiDS): \*eSp

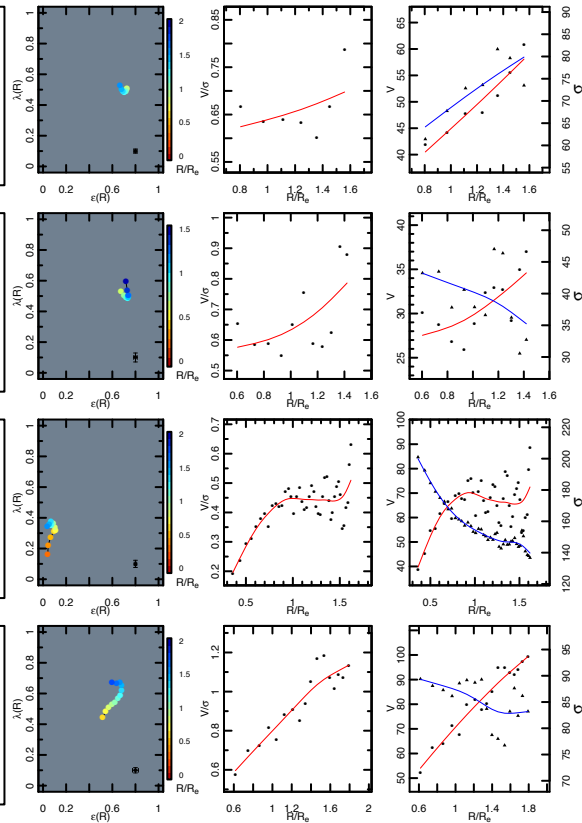

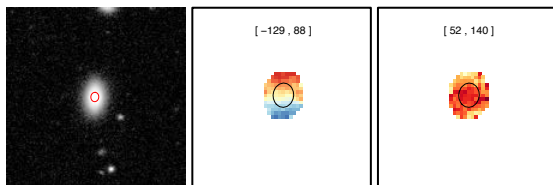

SAMI47293 (KiDS): S0

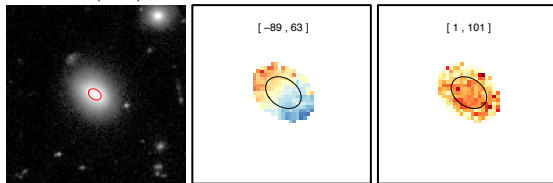

SAMI47493 (KiDS): ISp

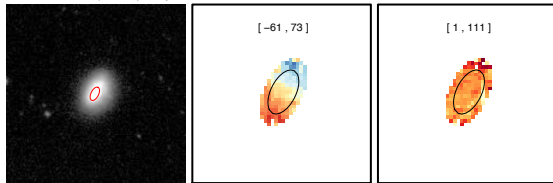

SAMI47500 (KiDS): ISp

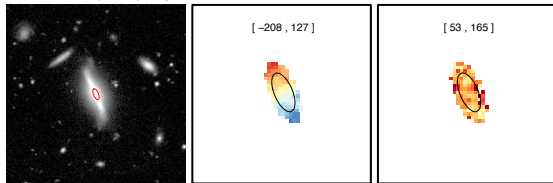

SAMI48016 (HSC): \*eSp

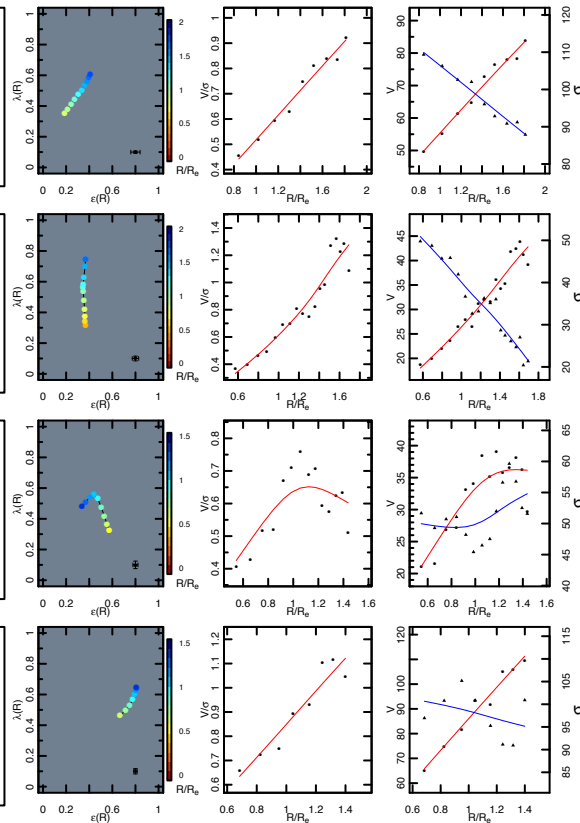

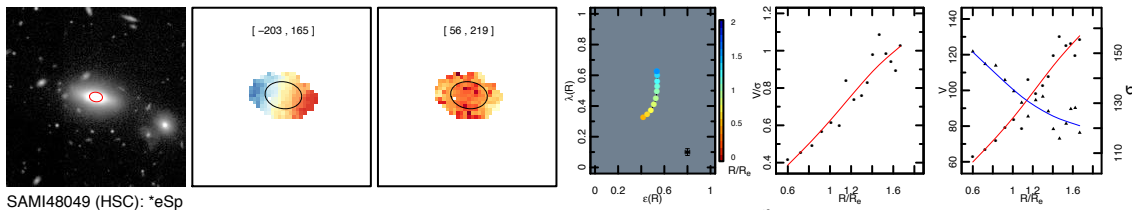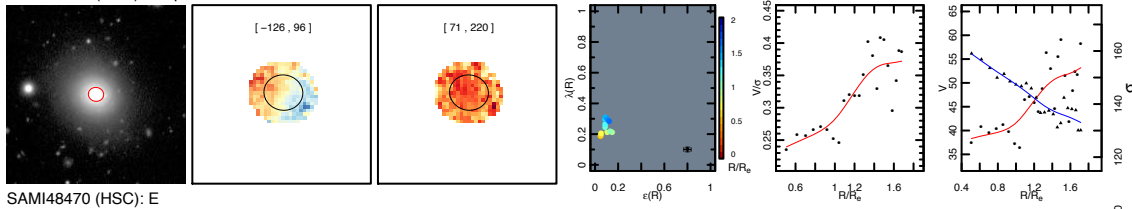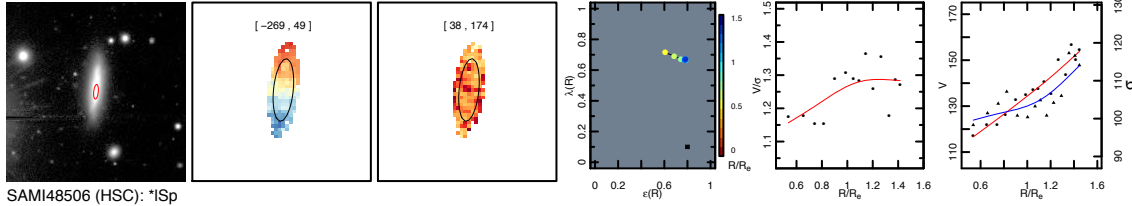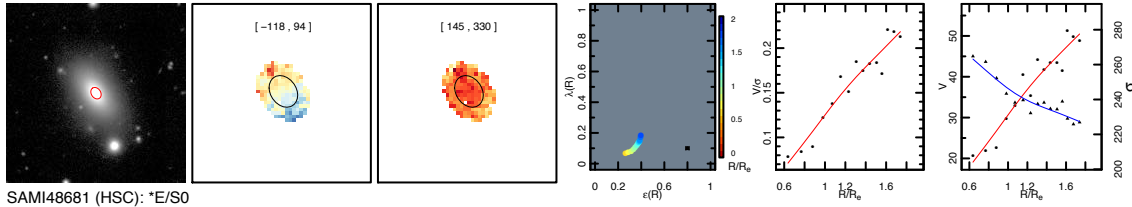

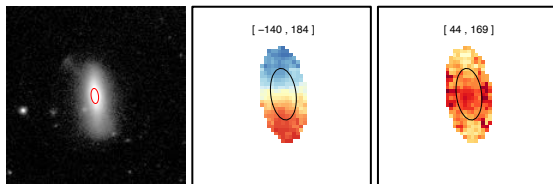

SAMI49734 (KiDS): S0

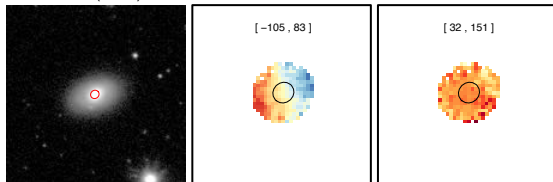

SAMI49784 (KiDS): S0

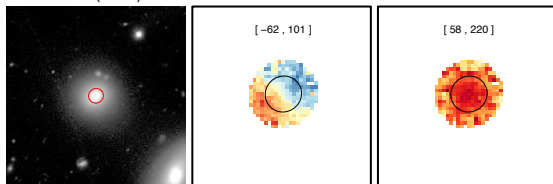

SAMI54202 (HSC): E

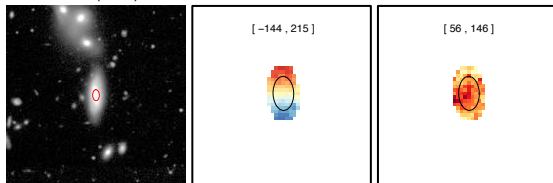

SAMI54957 (HSC): eSp

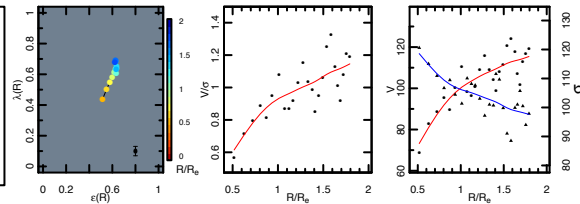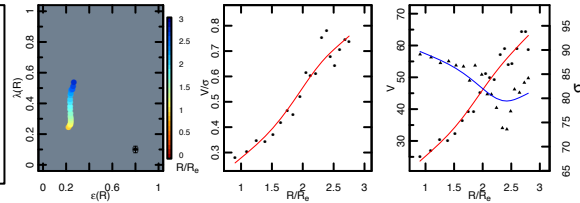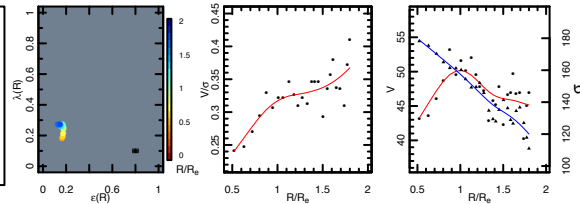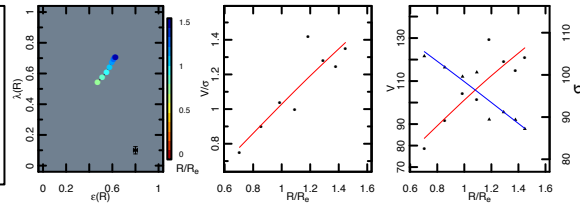

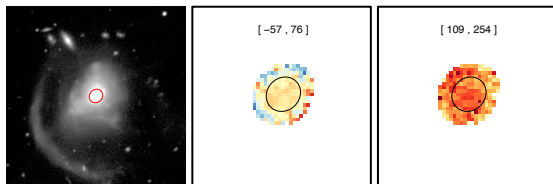

SAMI55245 (HSC): \*Merger

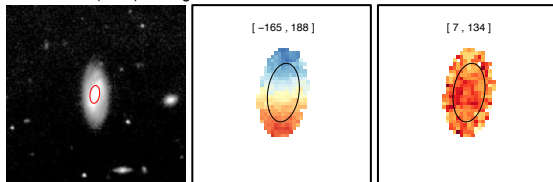

SAMI55537 (KiDS): \*ISp

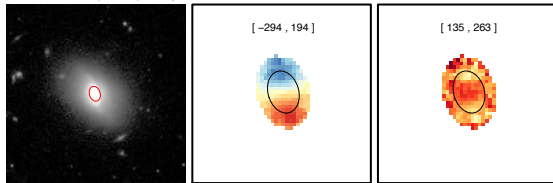

SAMI56140 (KiDS): \*Embedded Disc

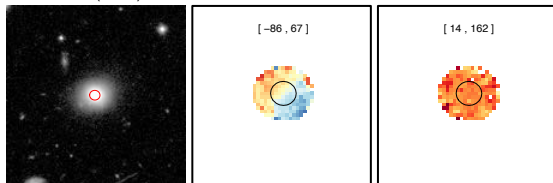

SAMI56181 (KiDS): E

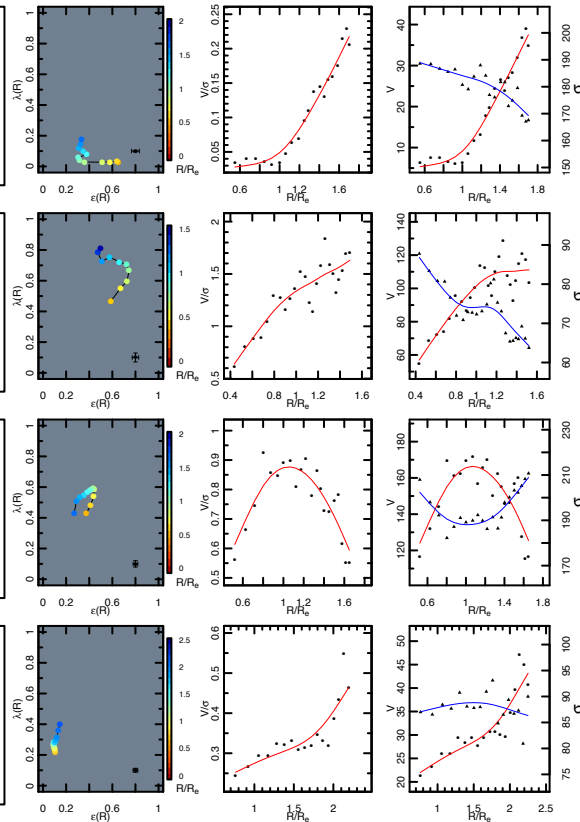

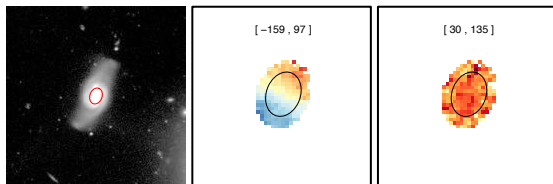

SAMI63276 (HSC): \*eSB

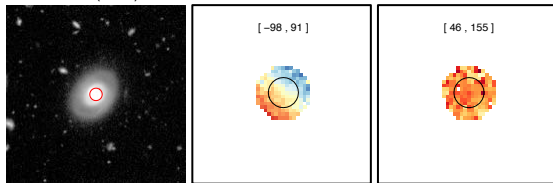

SAMI63780 (HSC): S0/eSp

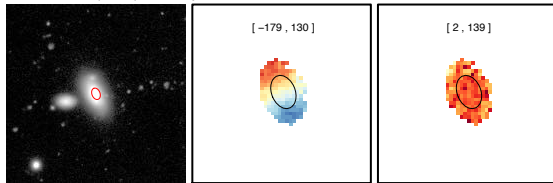

SAMI64087 (HSC): \*ISp

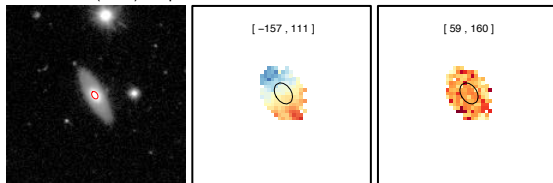

SAMI65384 (KiDS): eSp

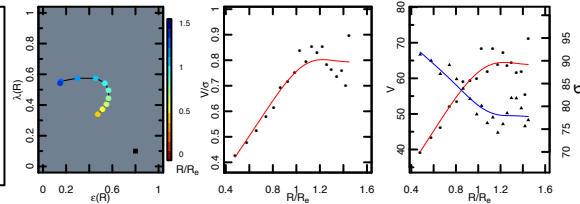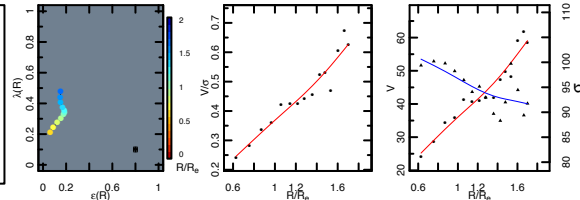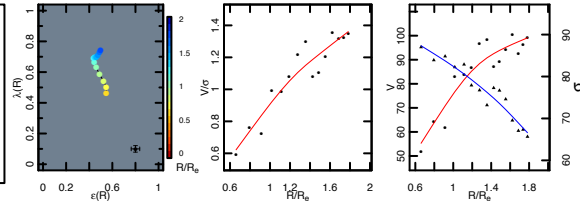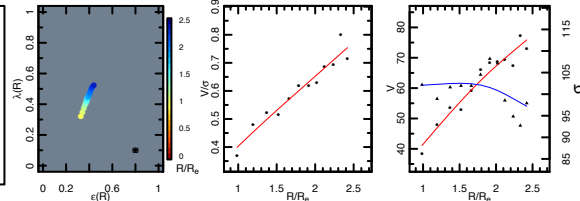

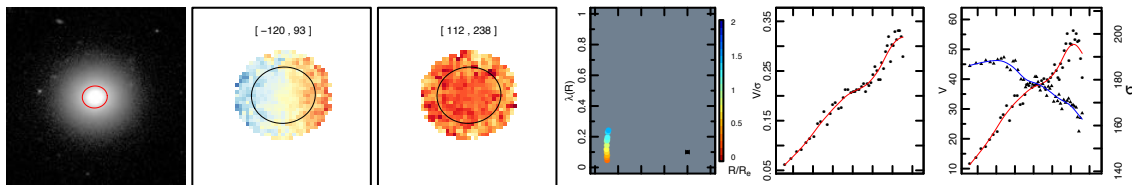

SAMI65408 (KiDS): E

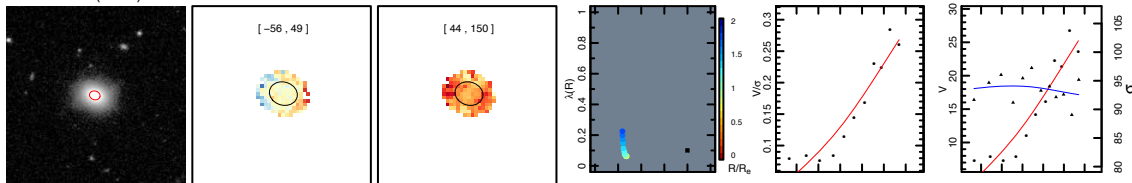

SAMI65410 (KiDS): \*E

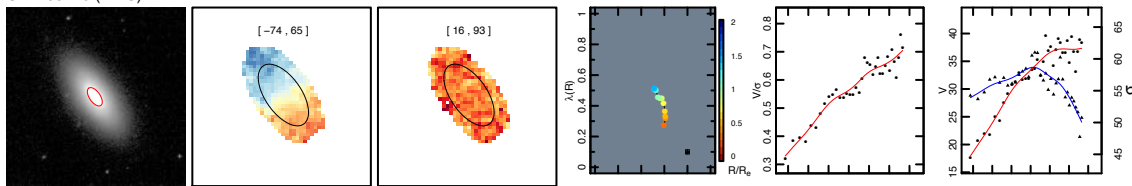

SAMI69740 (KiDS): ?

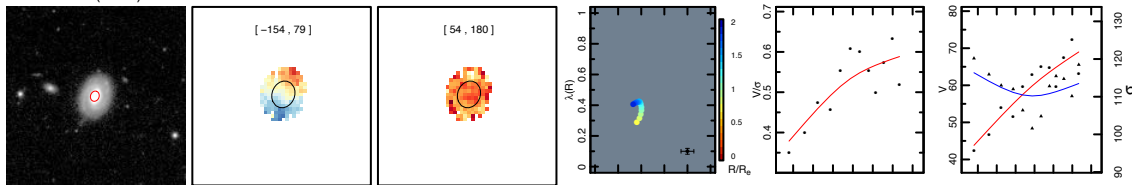

SAMI69752 (KiDS): eSp

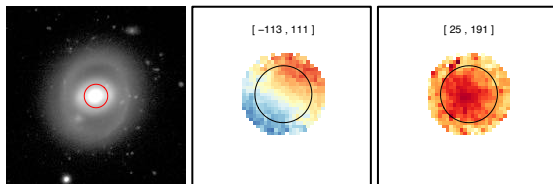

SAMI69986 (HSC): \*NA

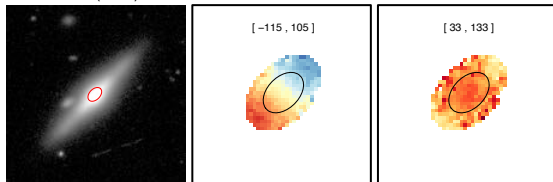

SAMI70532 (KiDS): \*S0

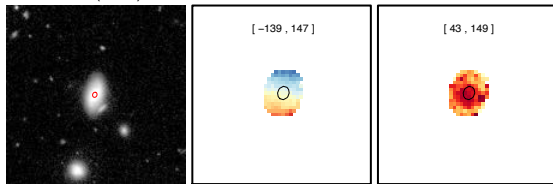

SAMI77227 (KiDS): eSp

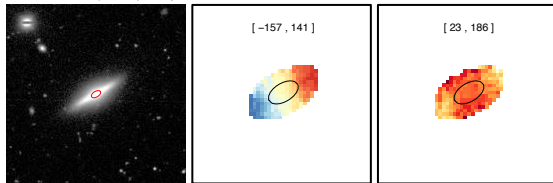

SAMI77710 (HSC): \*eSp

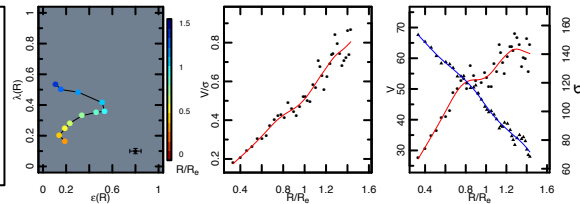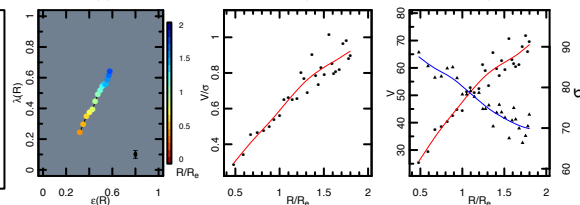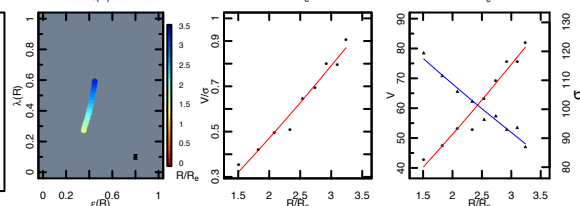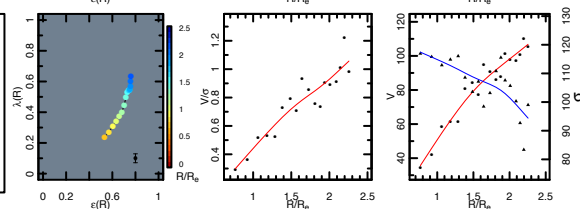



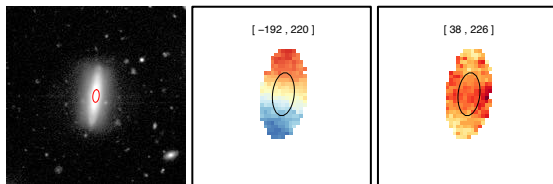

SAMI78355 (HSC): \*eSp

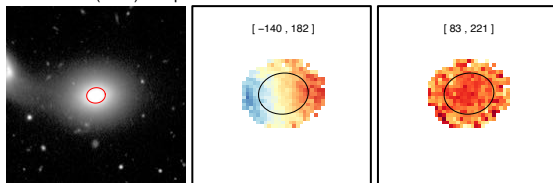

SAMI78530 (HSC): \*S0

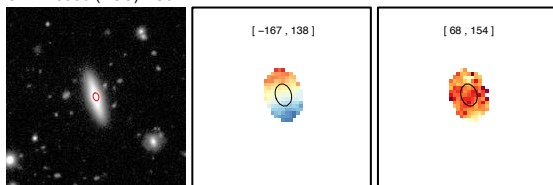

SAMI78634 (HSC): S0

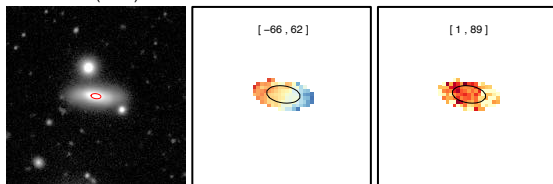

SAMI78791 (HSC): ISp

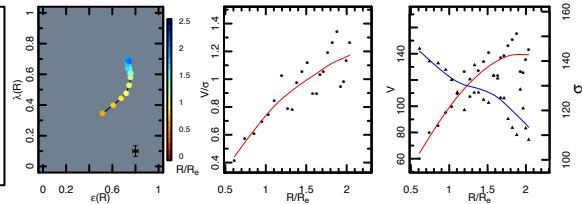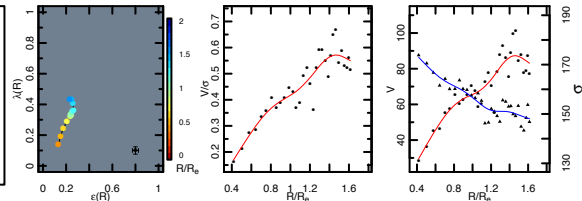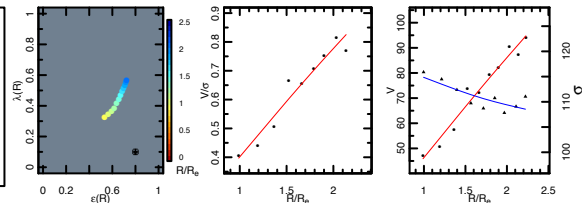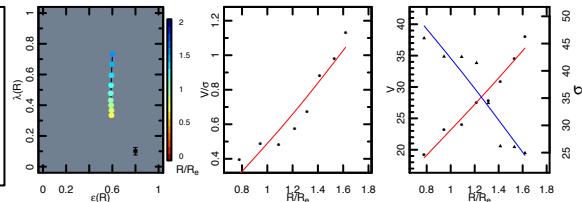

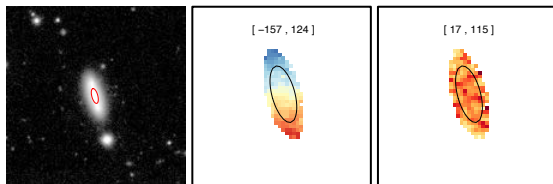

SAMI79693 (KiDS): \*eSp

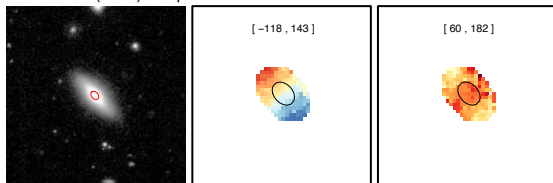

SAMI79711 (KiDS): S0

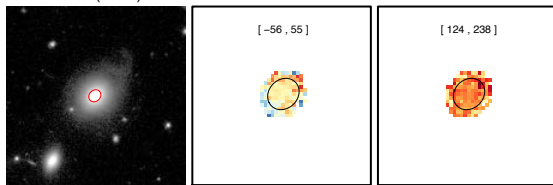

SAMI79750 (KiDS): E

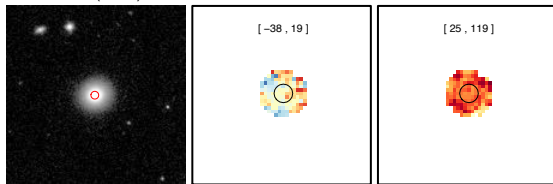

SAMI79810 (KiDS): E

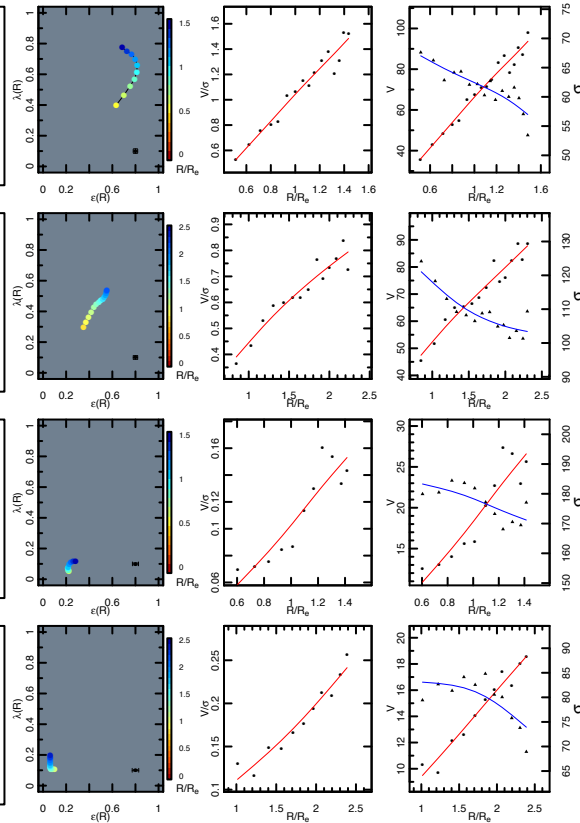

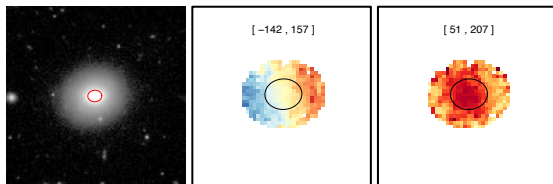

SAMI79866 (KiDS): E

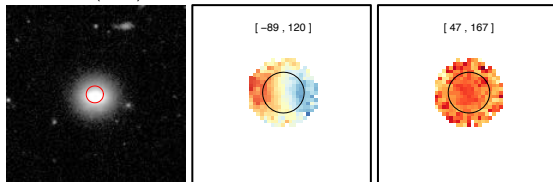

SAMI84106 (KiDS): \*E

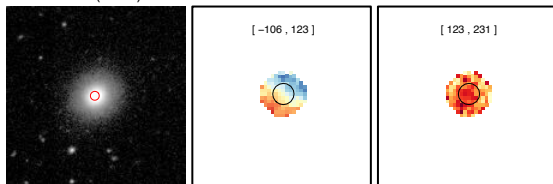

SAMI84209 (KiDS): E

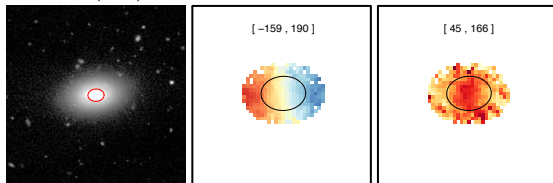

SAMI84680 (HSC): S0

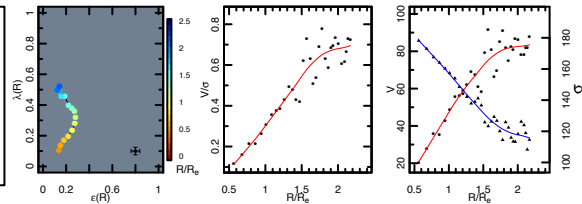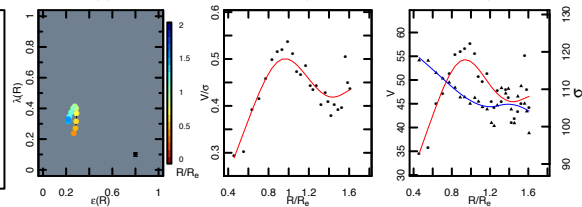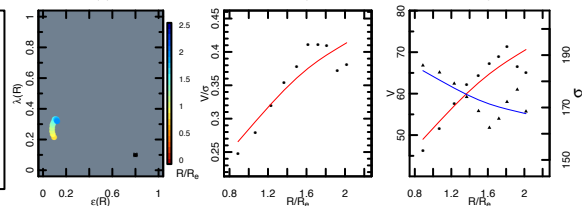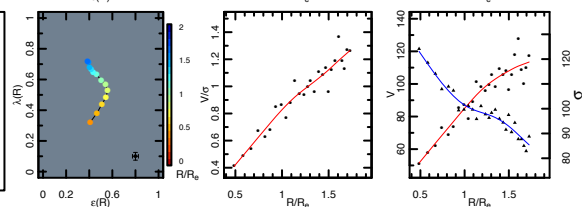

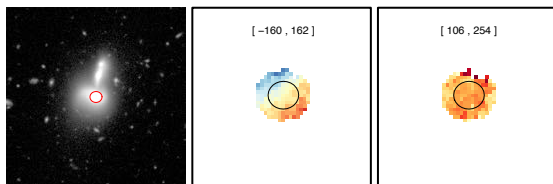

SAMI85239 (HSC): S0/eSp

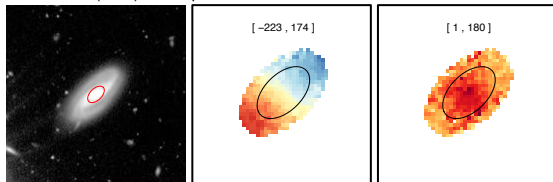

SAMI85280 (HSC): eSp

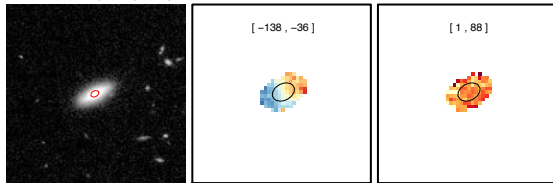

SAMI85507 (KiDS): \*2-sigma?

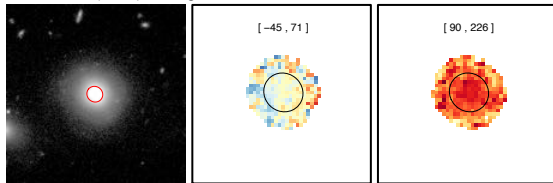

SAMI85667 (KiDS): E

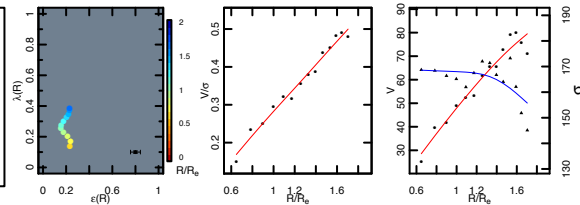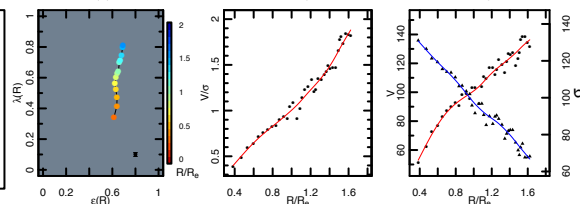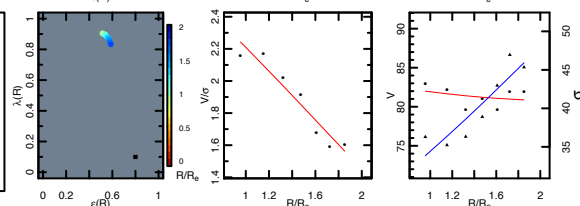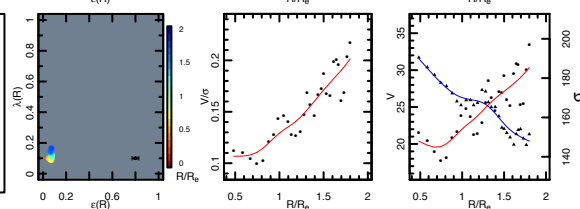

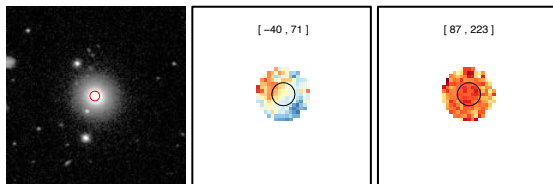

SAMI91545 (KiDS): E

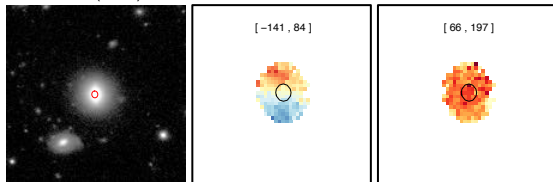

SAMI91568 (KiDS): E/SO

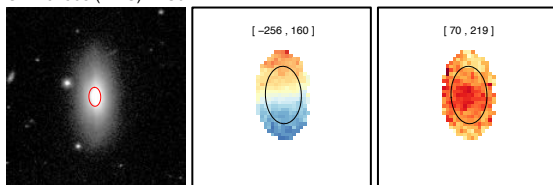

SAMI91686 (KiDS): S0

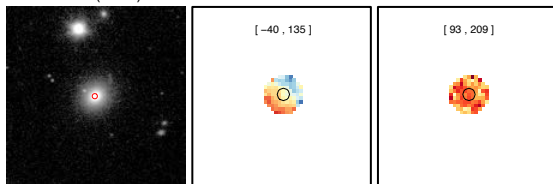

SAMI91689 (KiDS): E

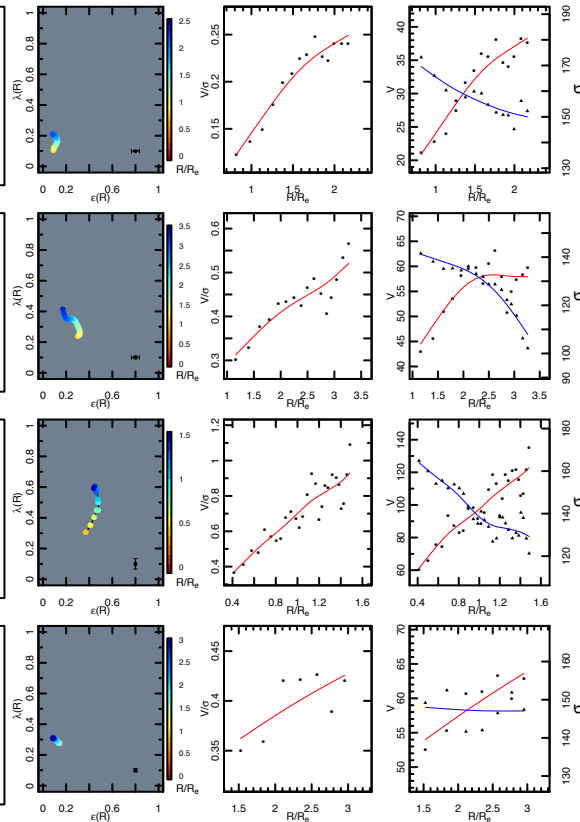

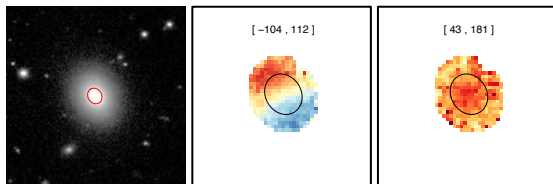

SAMI91697 (KiDS): \*Embedded Disc?

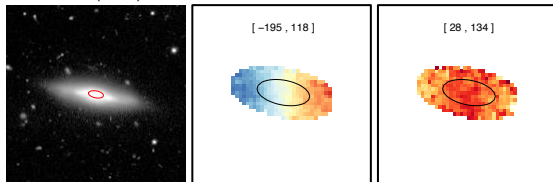

SAMI91926 (HSC): \*eSp

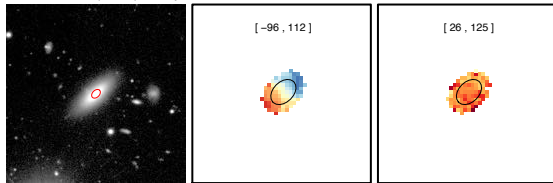

SAMI91959 (HSC): S0/eSp

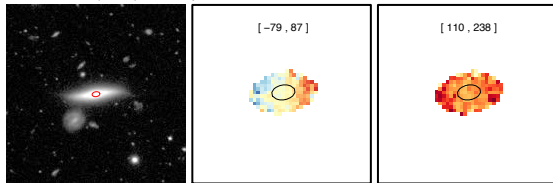

SAMI91996 (HSC): S0/eSp

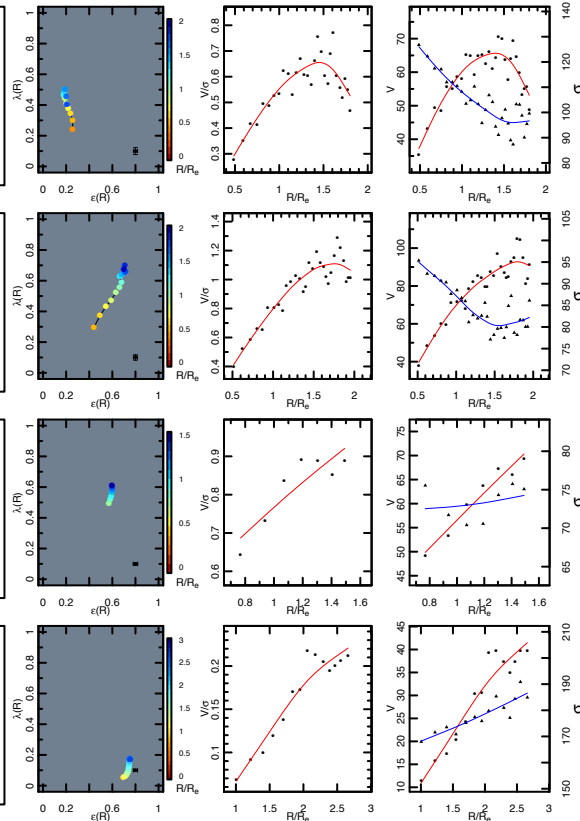

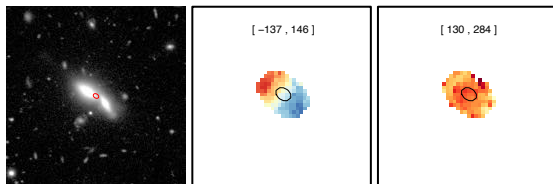

SAMI91999 (HSC): ?

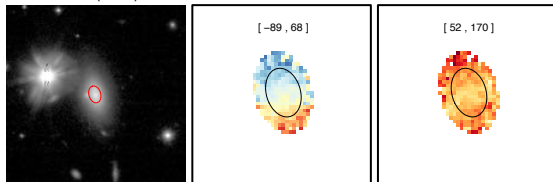

SAMI92770 (KiDS): ?

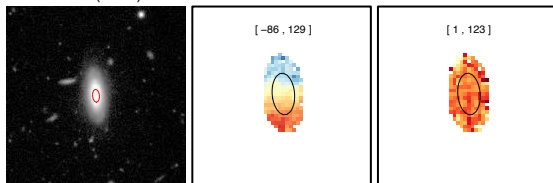

SAMI92944 (HSC): ISp

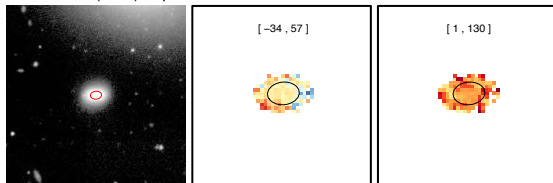

SAMI93020 (HSC): S0/eSp

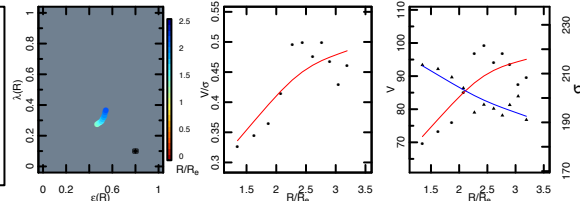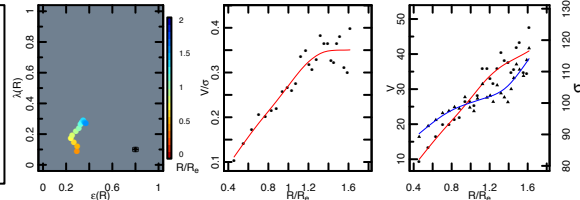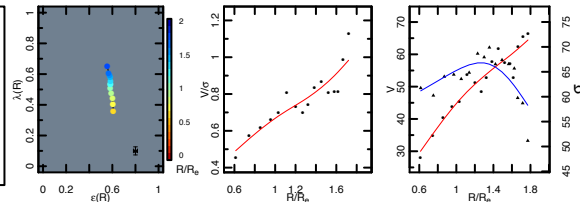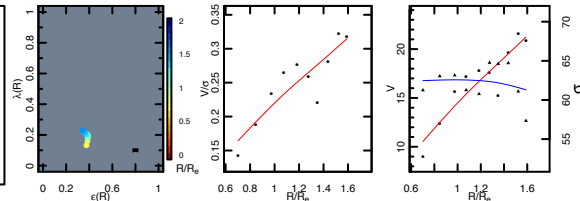

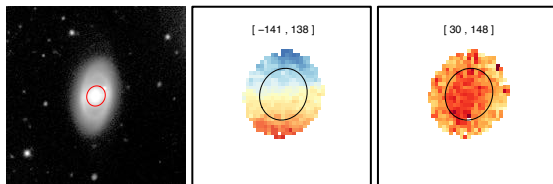

SAMI93023 (HSC): eSp

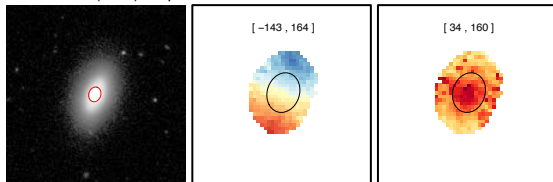

SAMI98097 (KiDS): S0

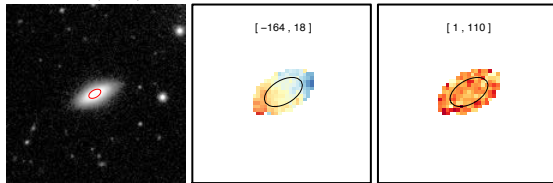

SAMI99430 (KiDS): \*2-sigma?

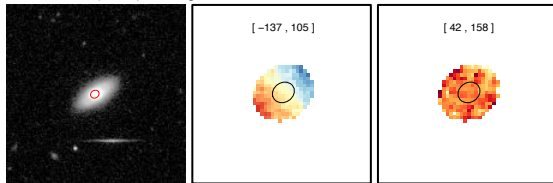

SAMI99742 (KiDS): \*S0

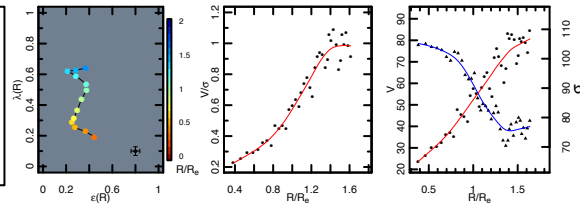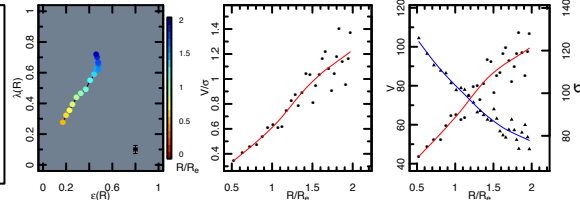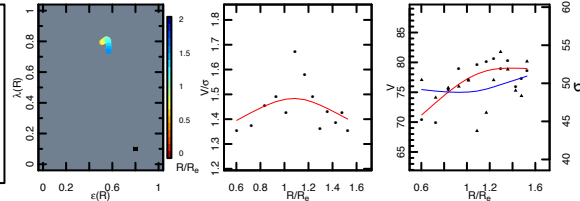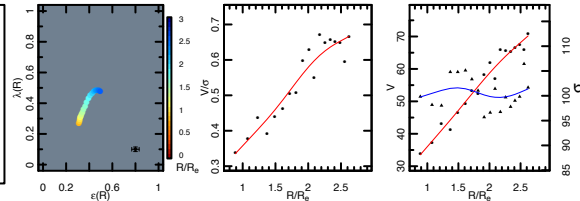



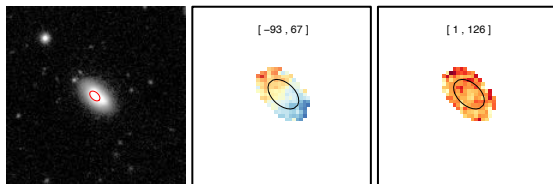

SAMI100162 (KiDS): ISp

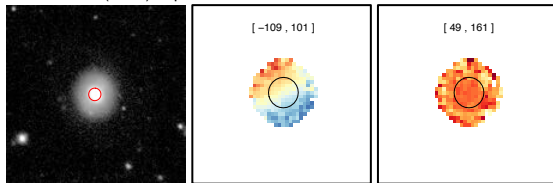

SAMI105420 (KiDS): eSp

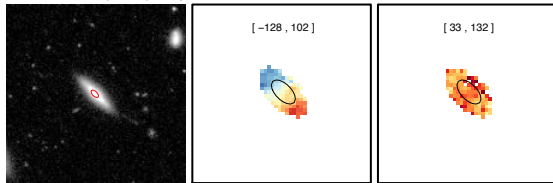

SAMI105447 (KiDS): \*S0

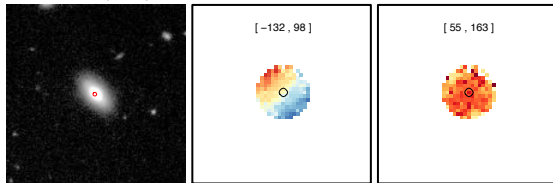

SAMI105519 (KiDS): S0

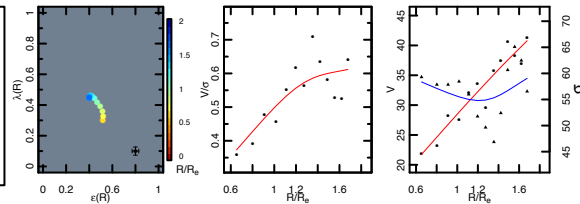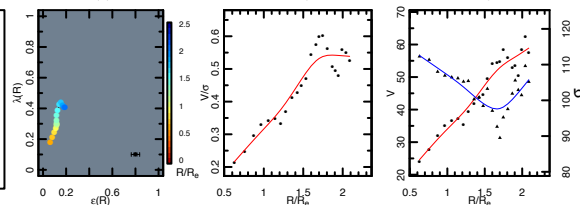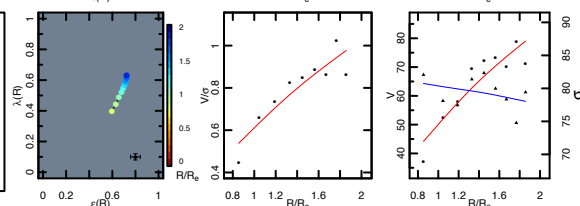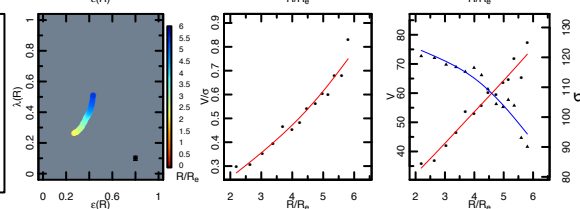

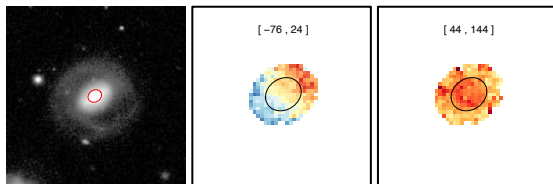

SAMI105738 (KiDS): \*eSB

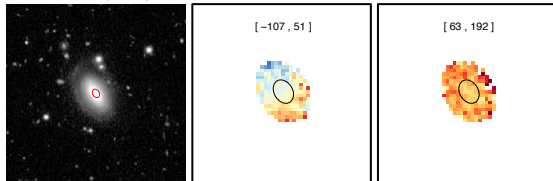

SAMI106047 (HSC): S0/eSp

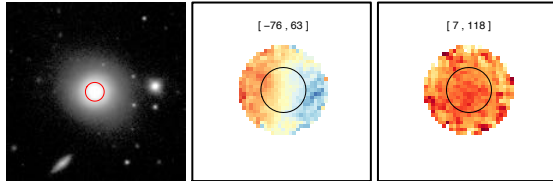

SAMI106549 (KiDS): \*E

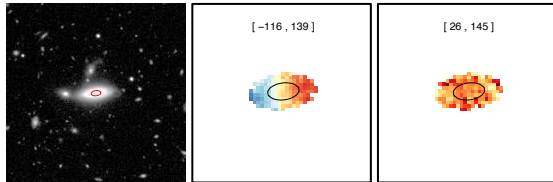

SAMI106634 (HSC): \*eSp

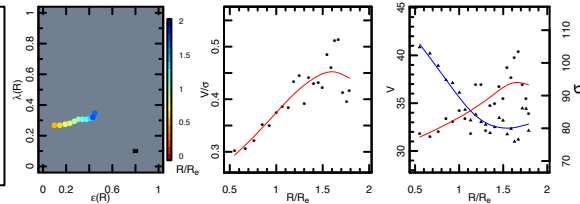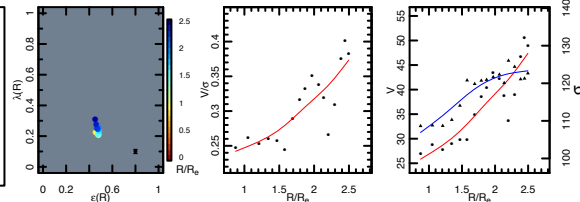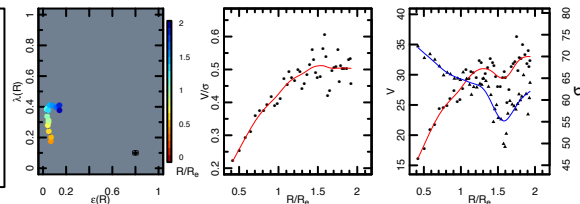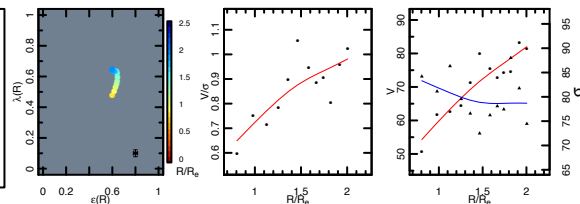

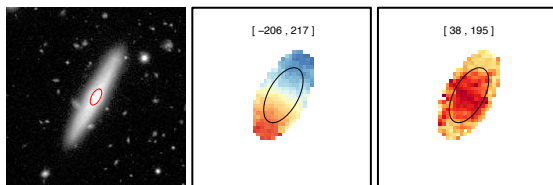

SAMI106810 (HSC): SO/eSp

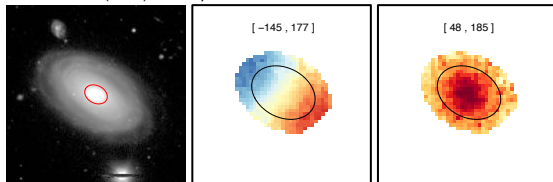

SAMI106839 (HSC): \*eSp

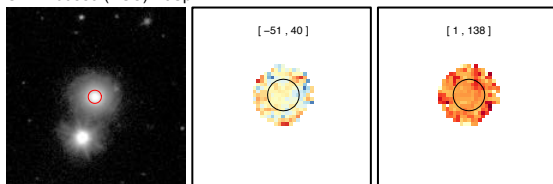

SAMI107454 (KiDS): \*E

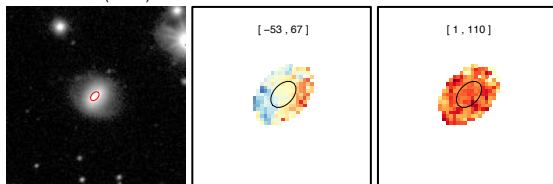

SAMI107503 (KiDS): \*ISp

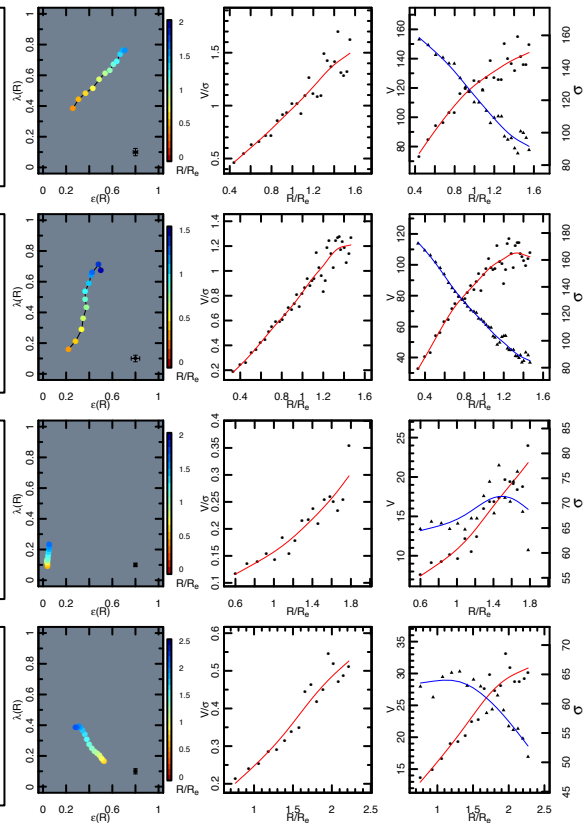

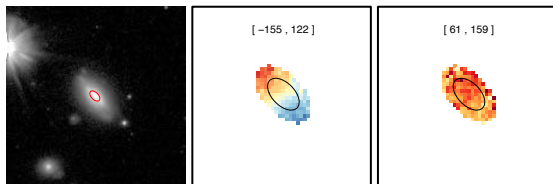

SAMI107824 (KiDS): eSp

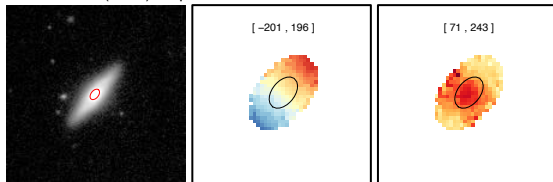

SAMI136232 (KiDS): \*S0

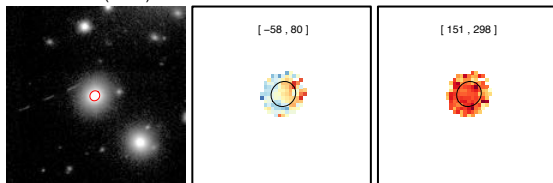

SAMI136605 (KiDS): E

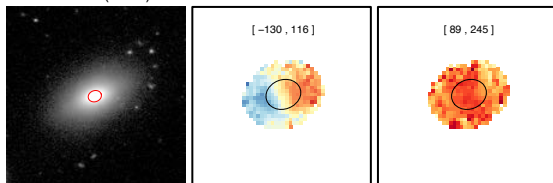

SAMI136616 (KiDS): S0

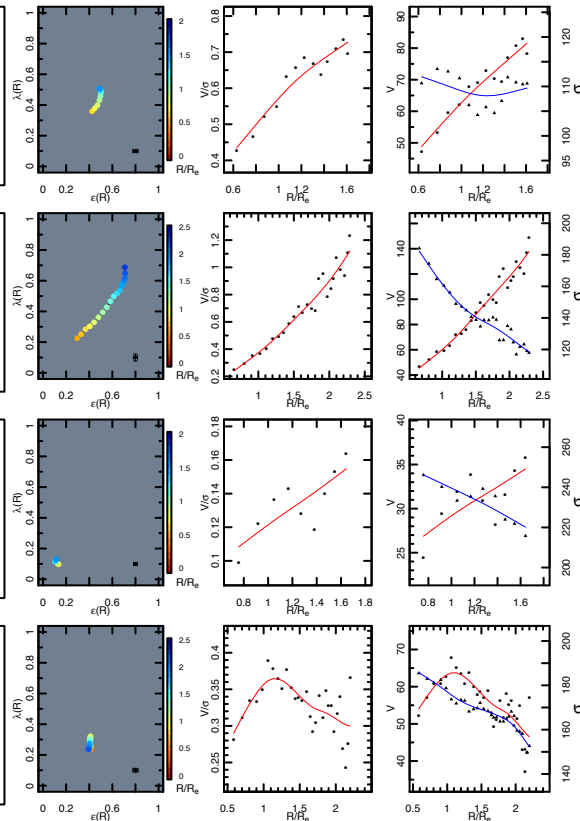

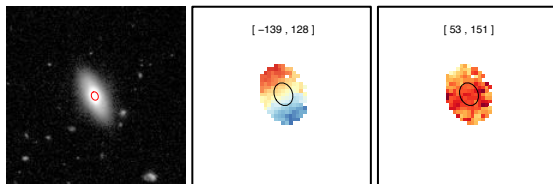

SAMI136624 (KiDS): S0

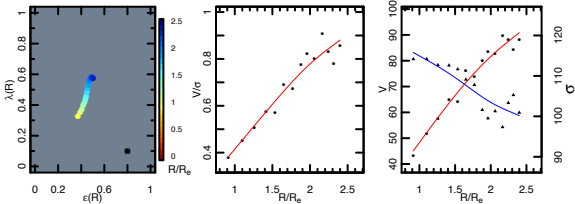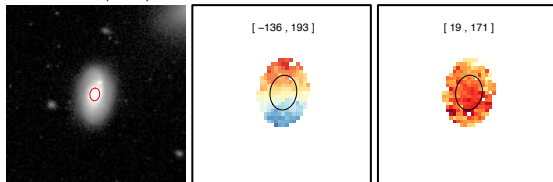

SAMI136688 (KiDS): eSp

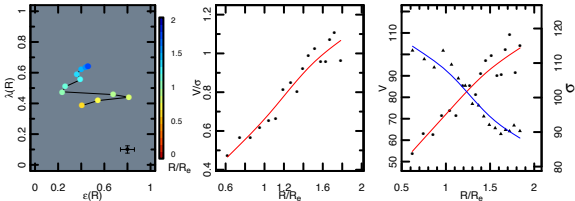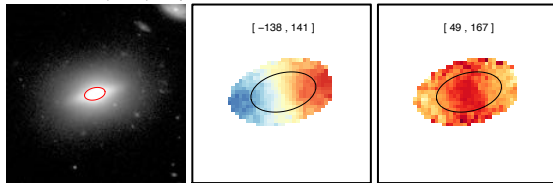

SAMI136841 (KiDS): \*Embedded Disc

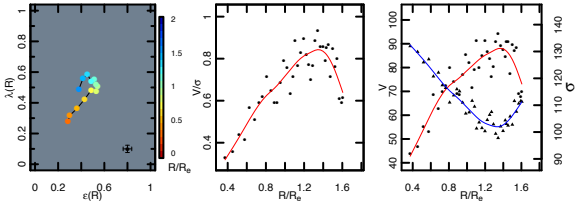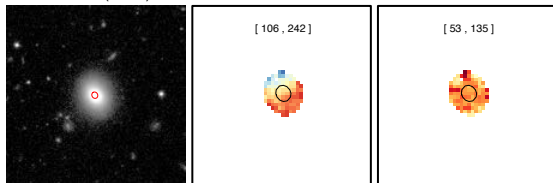

SAMI136871 (KiDS): \*E

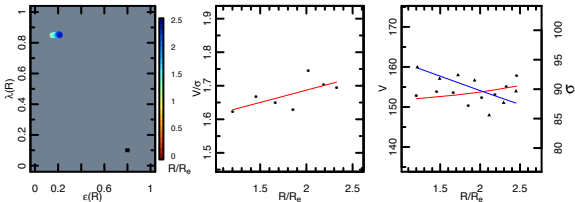

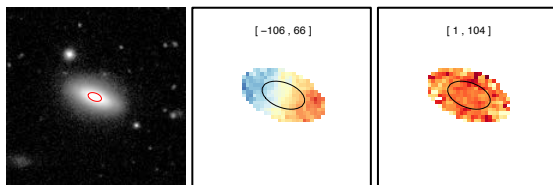

SAMI136880 (KiDS): S0/eSp

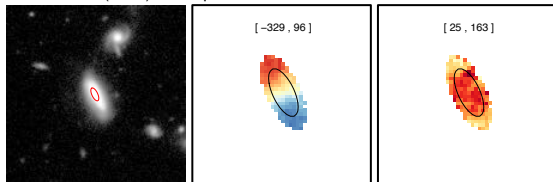

SAMI137809 (KiDS): eSp

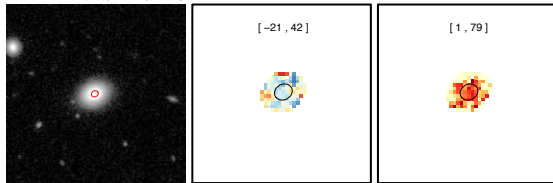

SAMI137841 (KiDS): S0

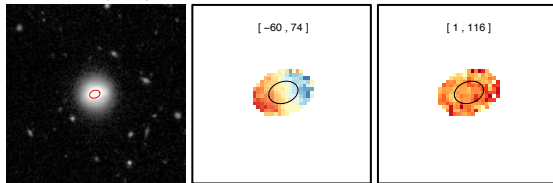

SAMI138381 (KiDS): ISp

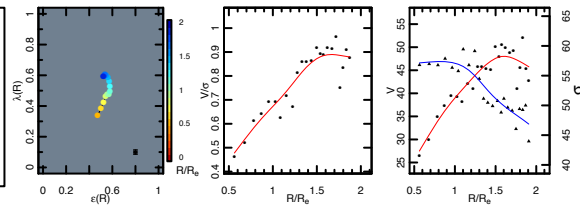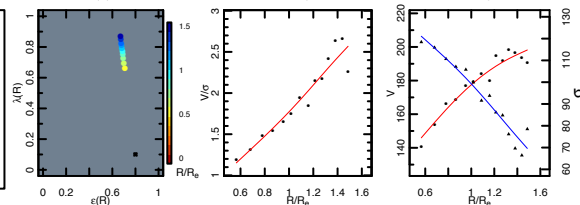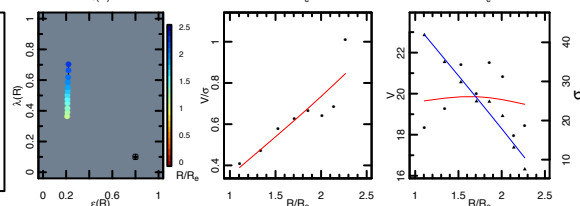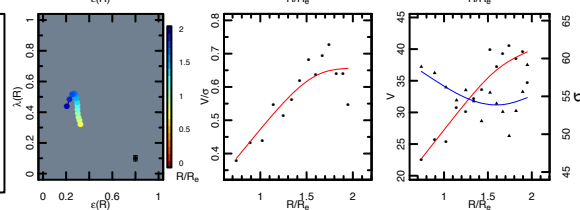

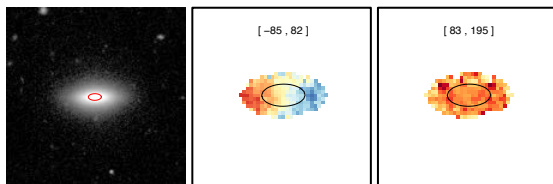

SAMI143227 (KiDS): S0/eSp

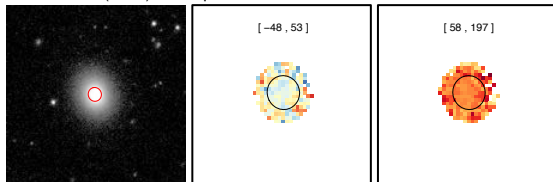

SAMI143291 (KiDS): E

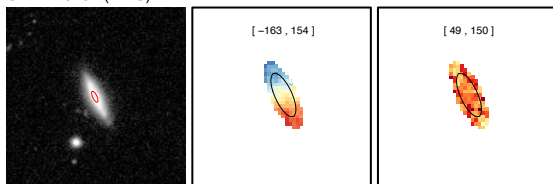

SAMI143605 (KiDS): \*eSp

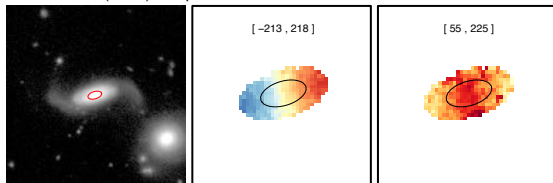

SAMI143736 (KiDS): \*eSp

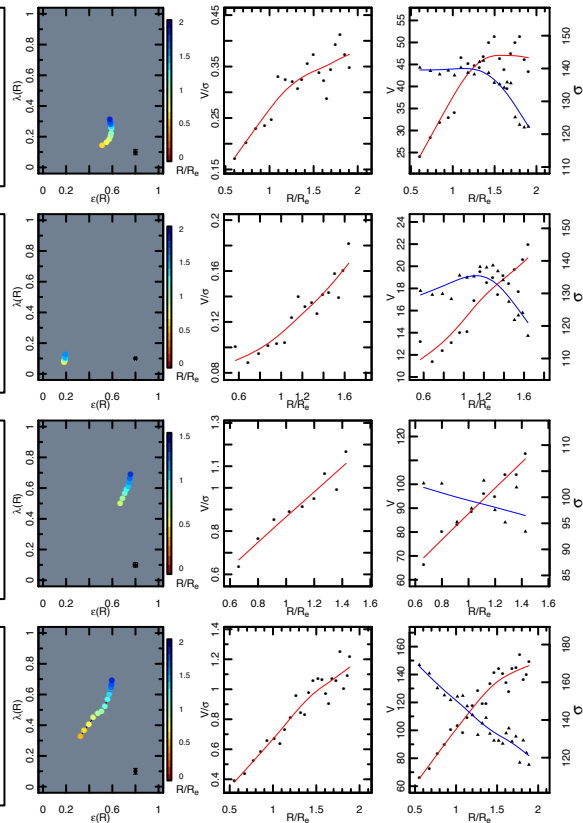

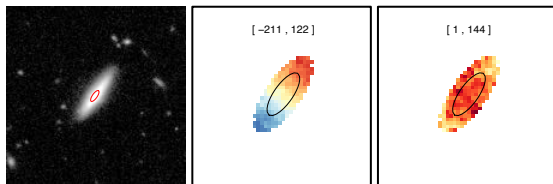

SAMI143746 (KiDS): \*S0

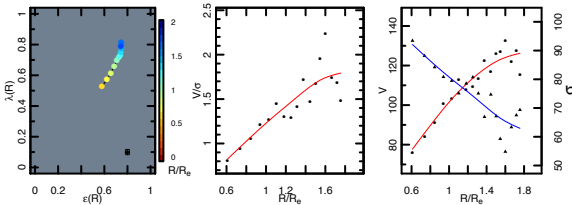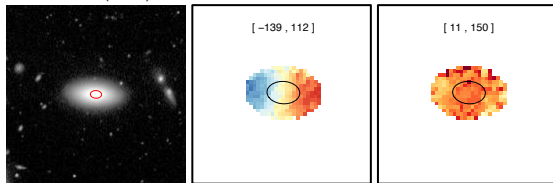

SAMI143918 (HSC): S0

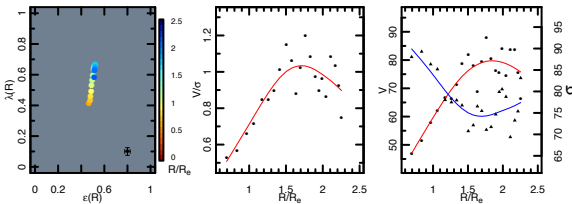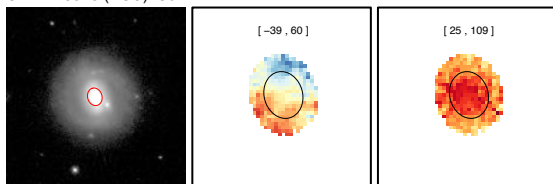

SAMI144051 (KiDS): \*eSB

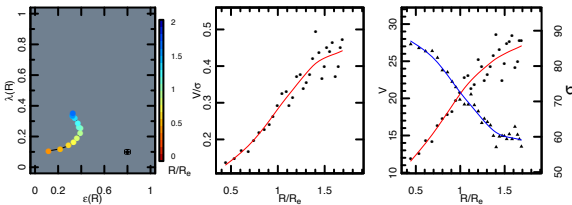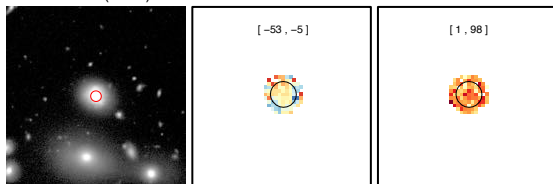

SAMI144197 (HSC): iSp

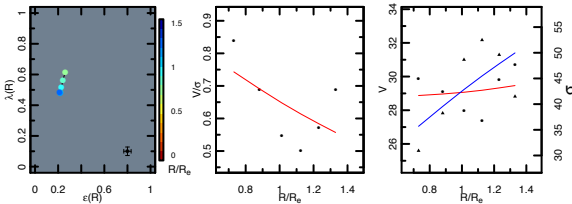



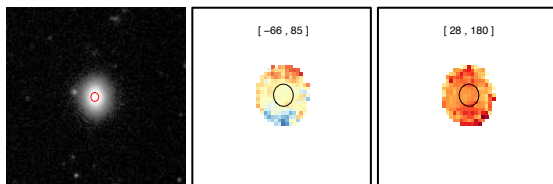

SAMI144320 (KiDS): ?

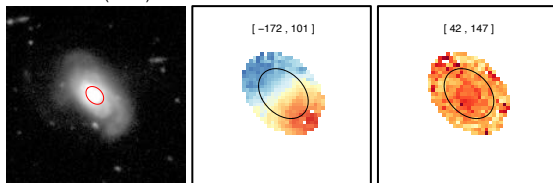

SAMI144402 (KiDS): \*Merger

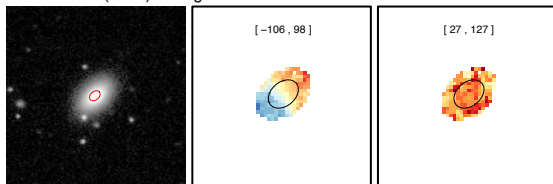

SAMI144498 (KiDS): S0

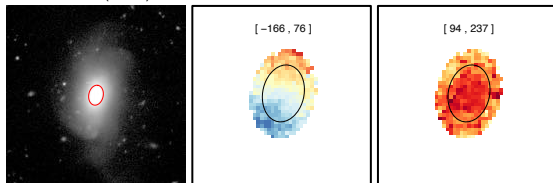

SAMI144640 (HSC): \*Merger

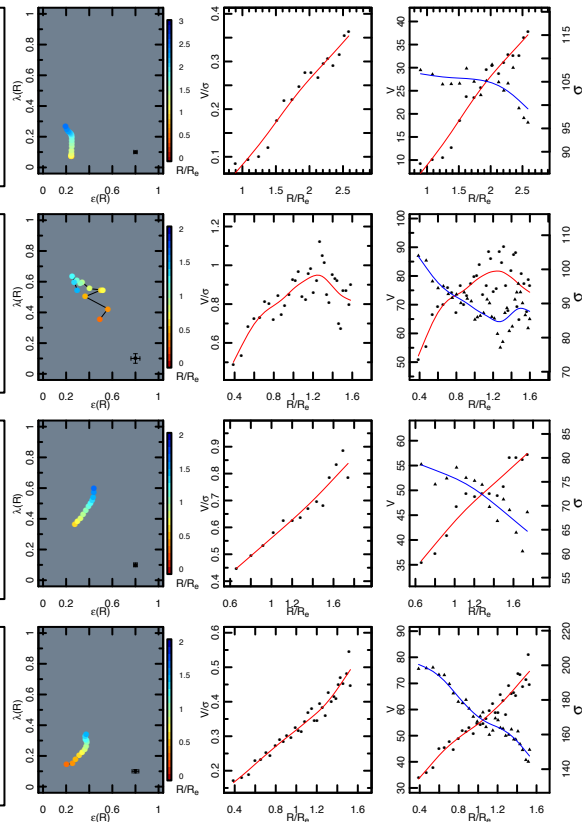

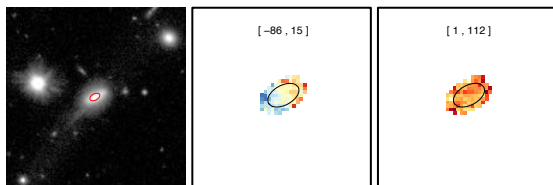

SAMI145073 (KiDS): ISp

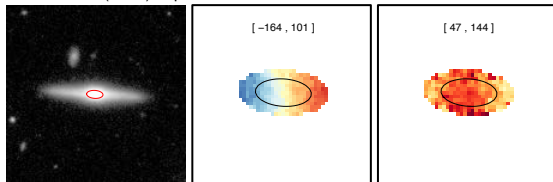

SAMI145729 (KiDS): \*eSp

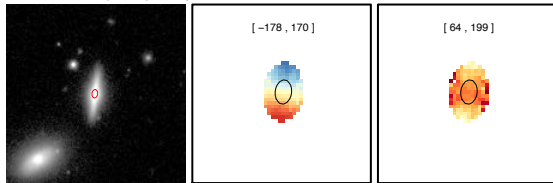

SAMI177010 (KiDS): \*S0

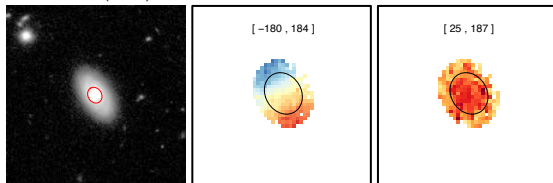

SAMI177143 (KiDS): eSp

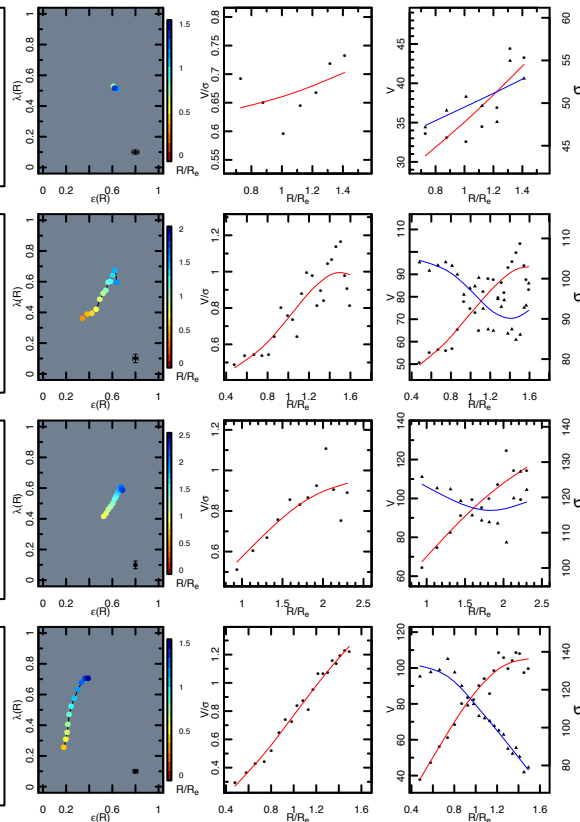

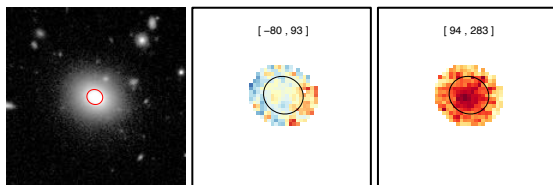

SAMI177969 (KiDS): E

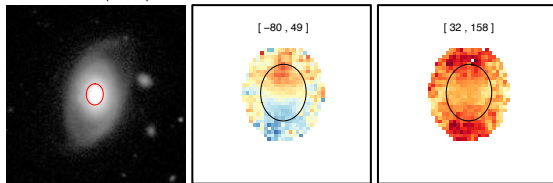

SAMI178197 (KiDS): \*Merger, 2-sigma

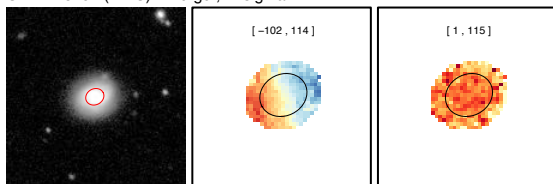

SAMI179584 (KiDS): \*ISp

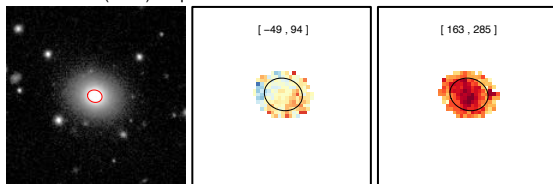

SAMI184046 (KiDS): E

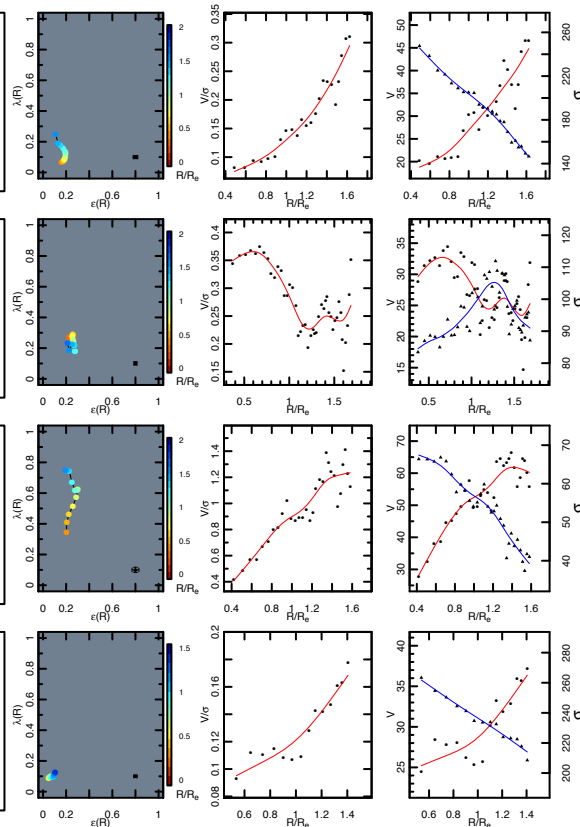

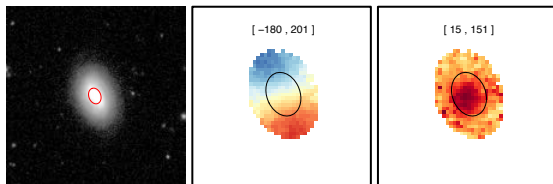

SAMI184122 (KiDS): eSp

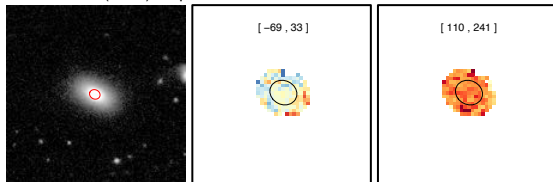

SAMI184202 (KiDS): \*E

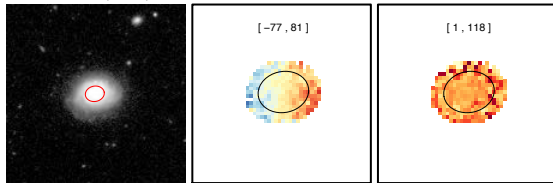

SAMI184415 (KiDS): ISp

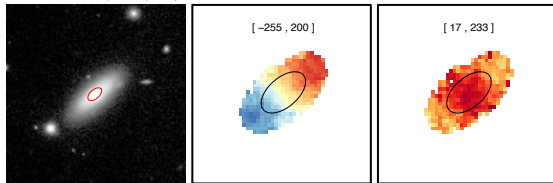

SAMI184689 (KiDS): \*SO

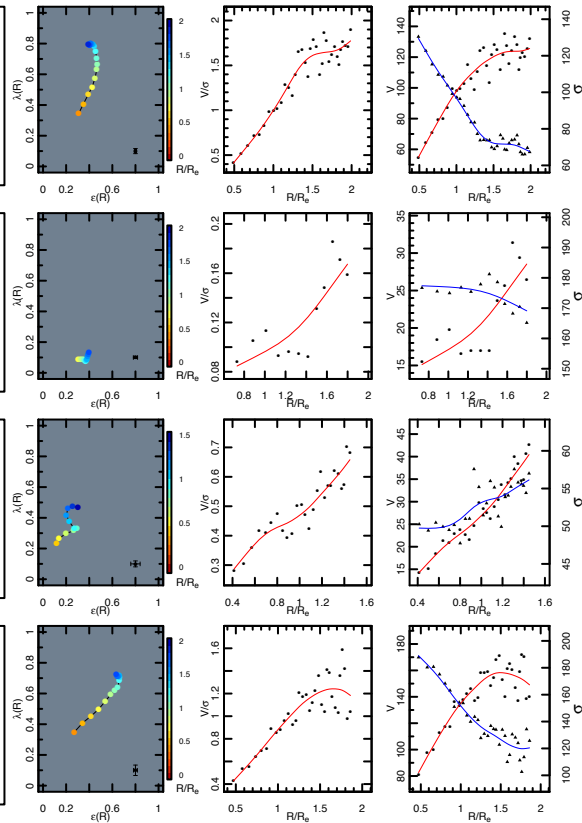

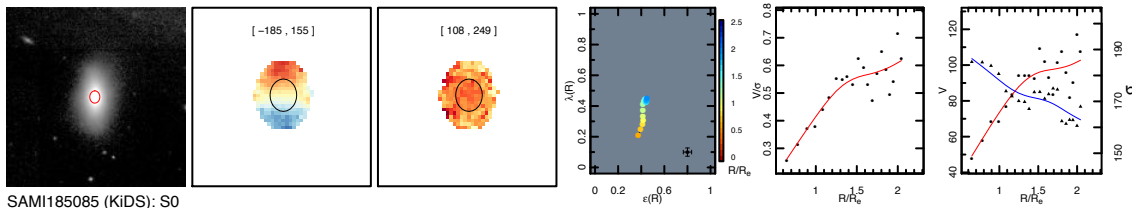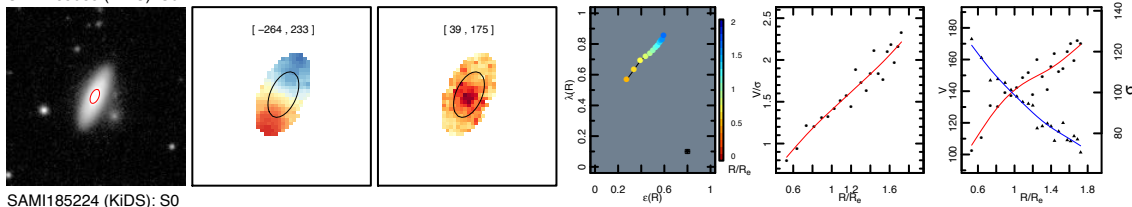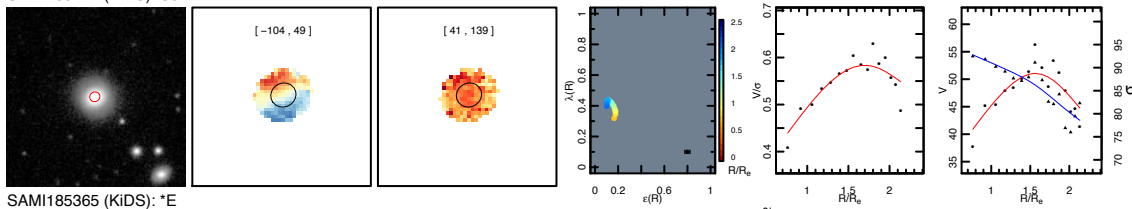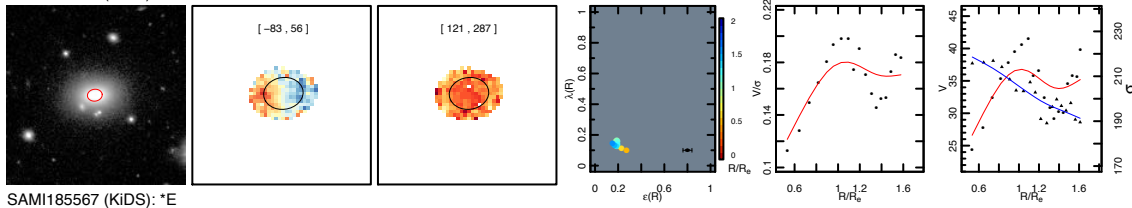

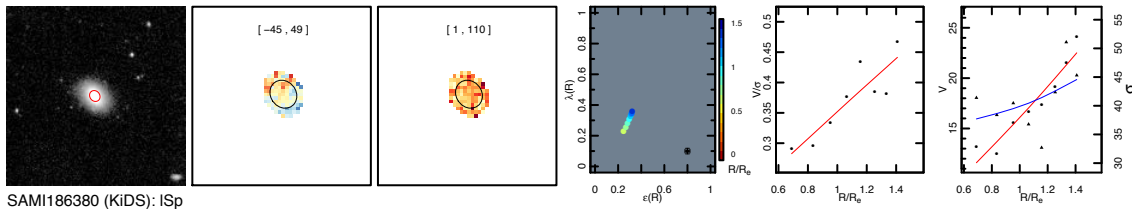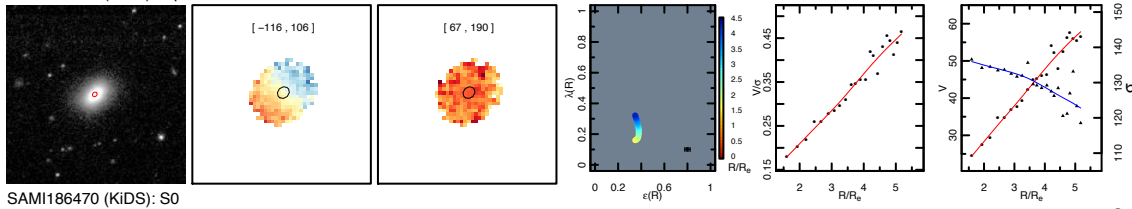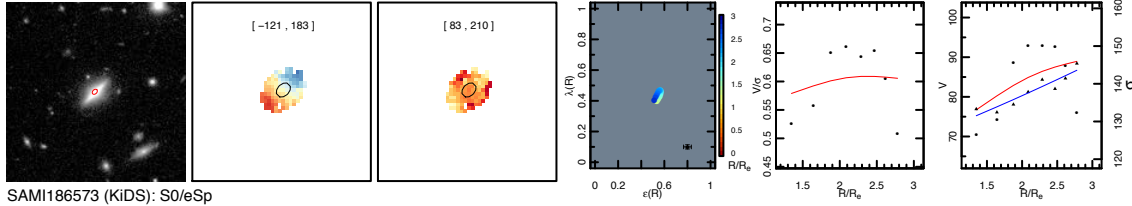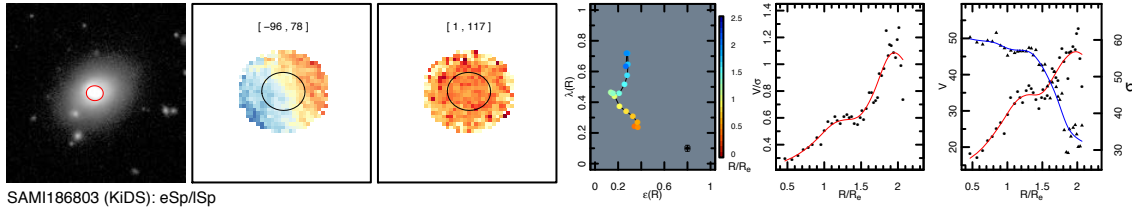

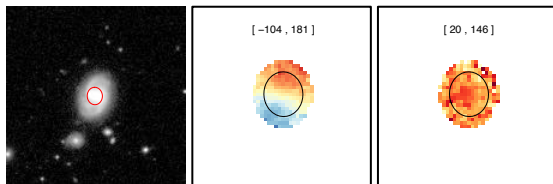

SAMI197866 (KiDS): eSp

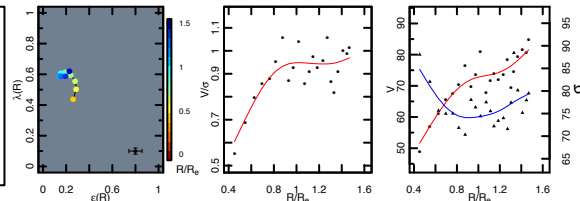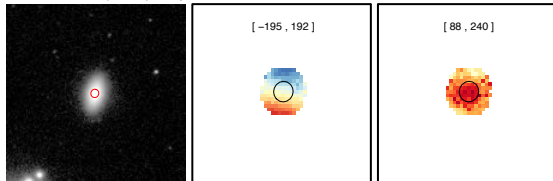

SAMI198343 (KiDS): S0

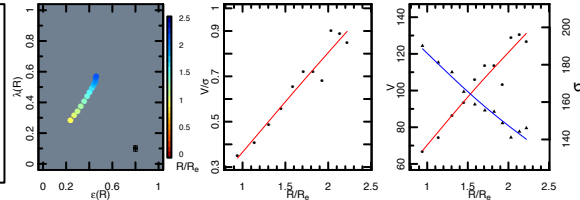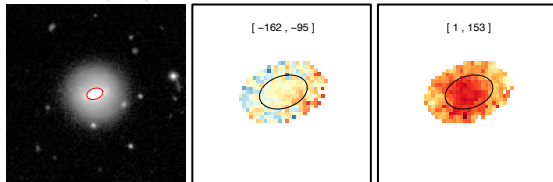

SAMI202360 (KiDS): eSp

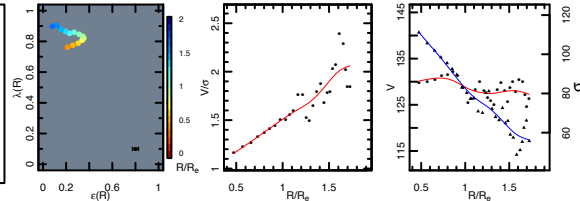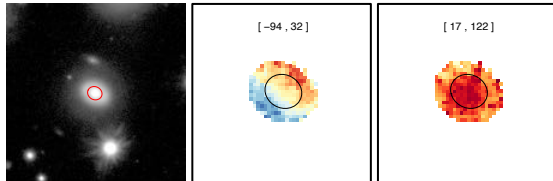

SAMI202398 (KiDS): \*Prolate Rotator

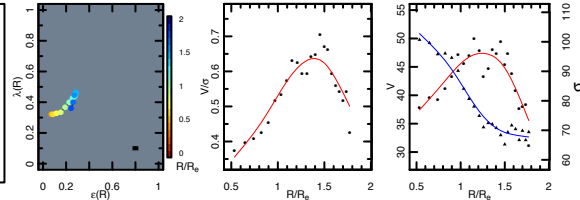

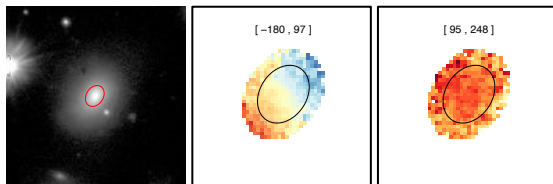

SAMI202399 (KiDS): S0

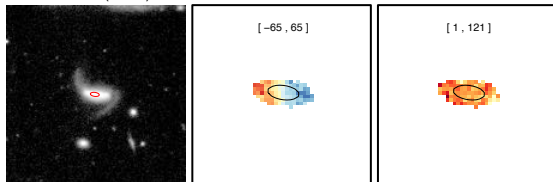

SAMI202636 (KiDS): ISp

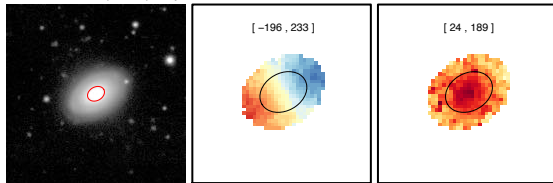

SAMI203114 (HSC): eSp

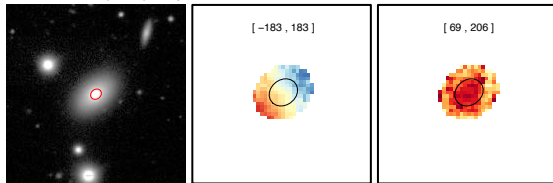

SAMI203140 (HSC): S0

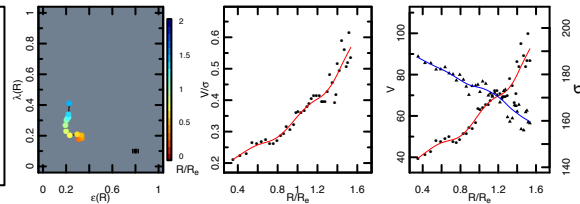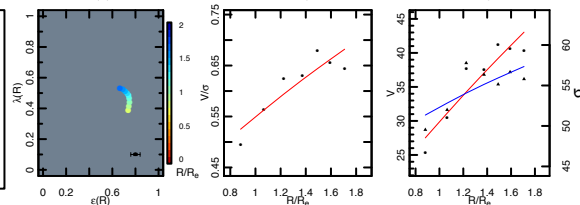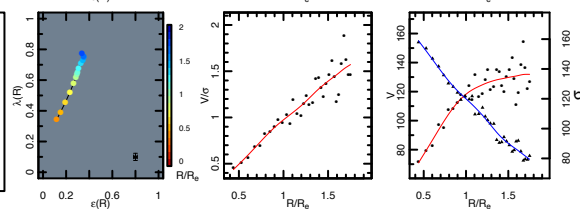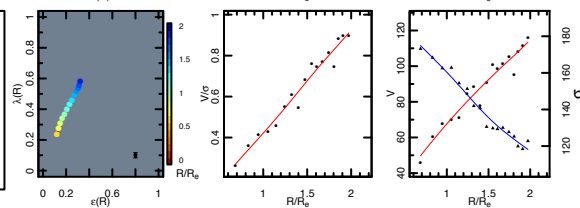



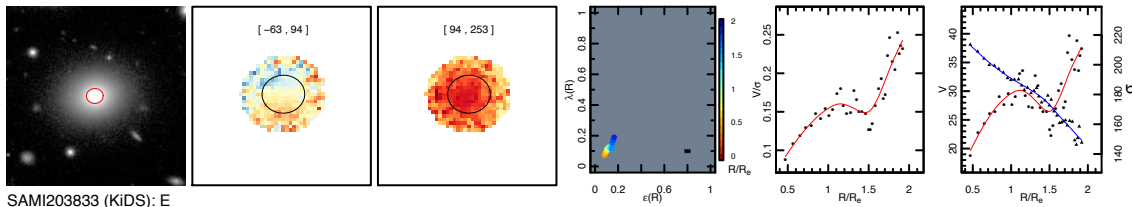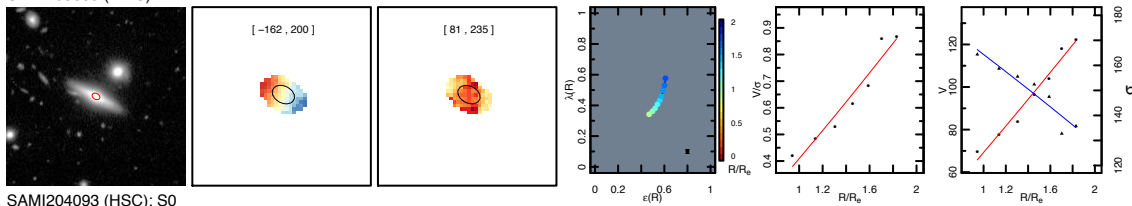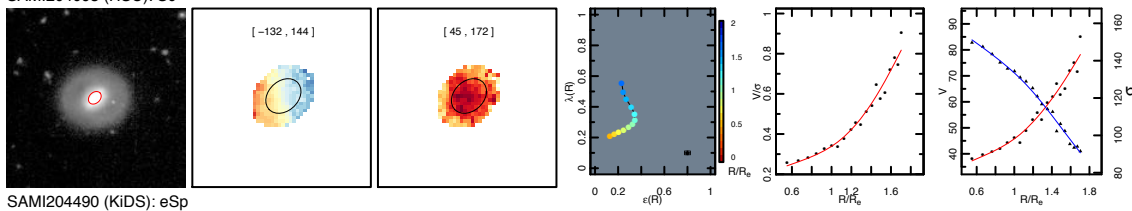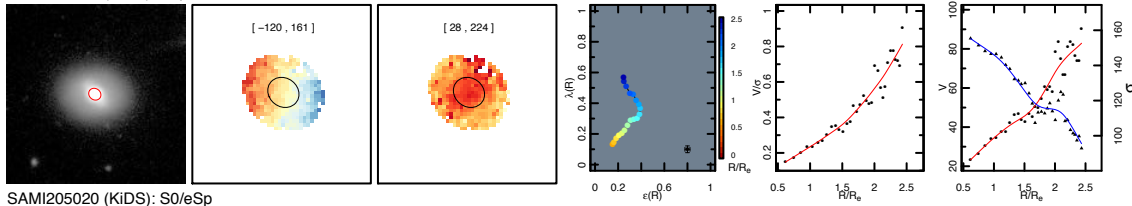

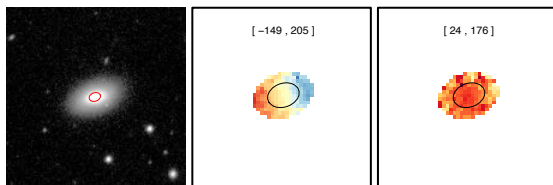

SAMI205089 (KiDS): S0

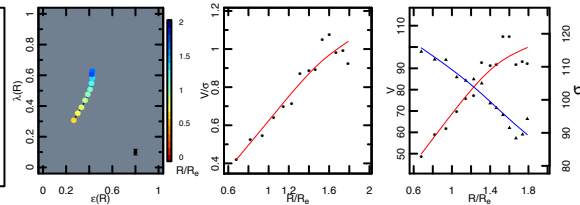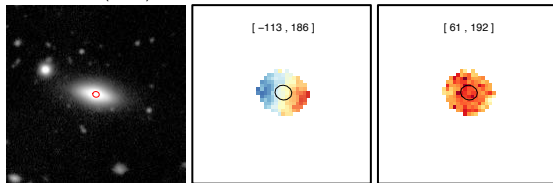

SAMI208876 (HSC): S0

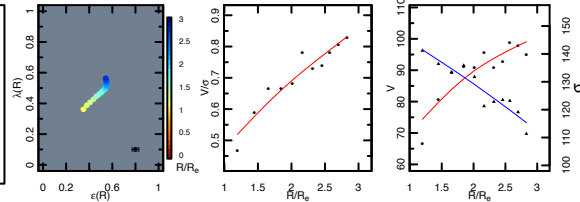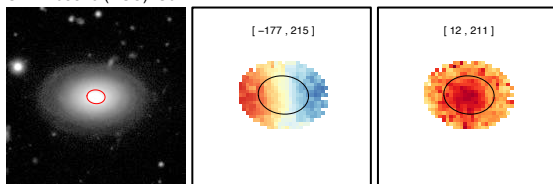

SAMI209185 (HSC): \*S0/eSp

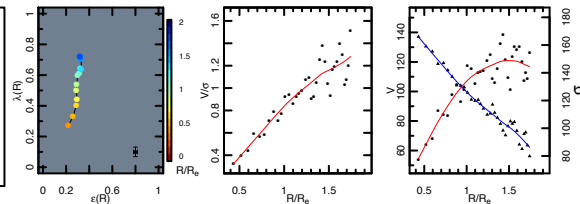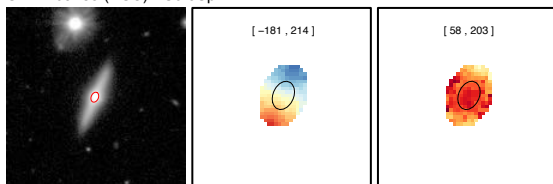

SAMI210228 (KiDS): \*S0

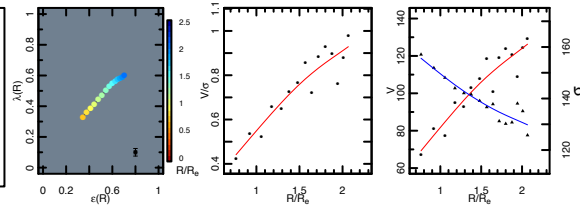

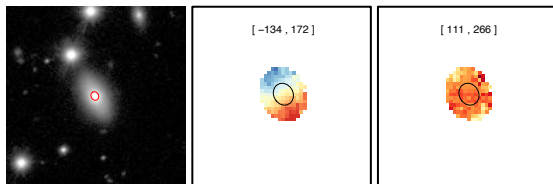

SAMI210375 (KiDS): S0

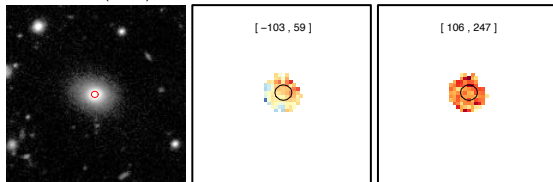

SAMI210467 (KiDS): E

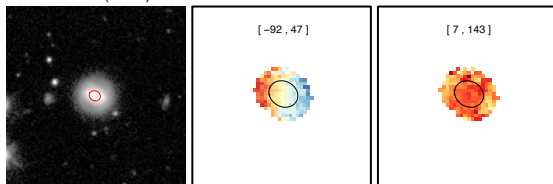

SAMI210611 (KiDS): eSp

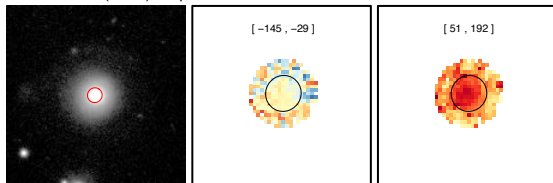

SAMI214211 (KiDS): \*E

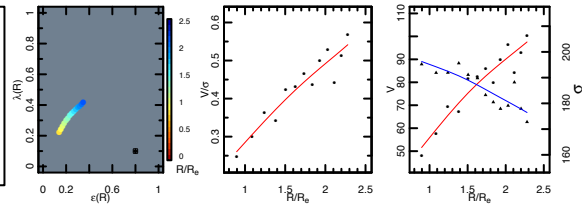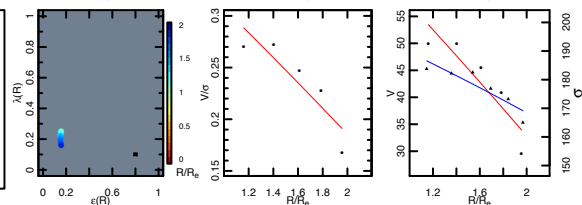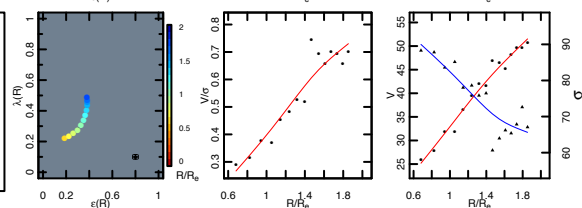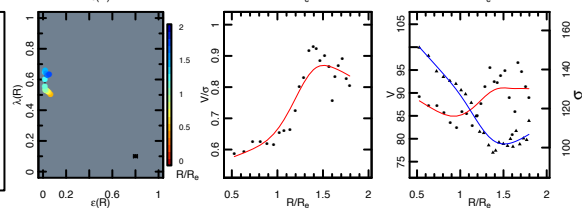

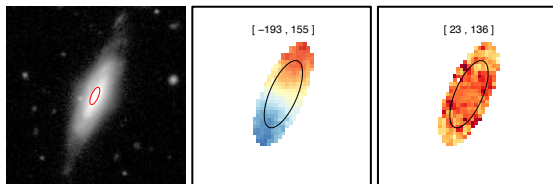

SAMI215292 (KiDS): ISp

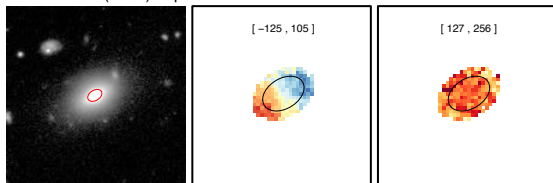

SAMI216396 (KiDS): S0

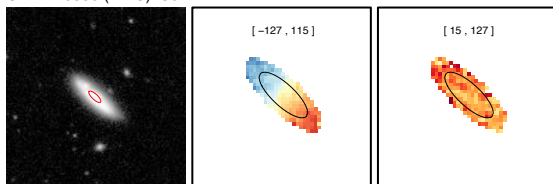

SAMI218681 (KiDS): ISp

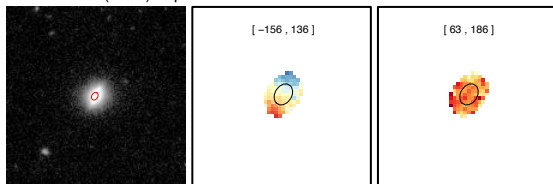

SAMI219992 (KiDS): S0

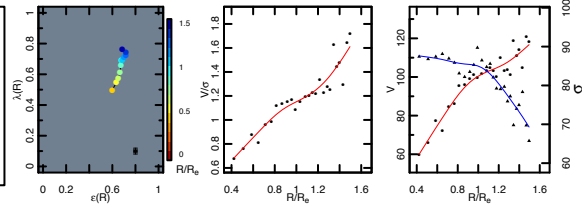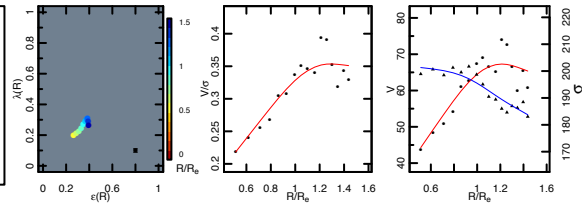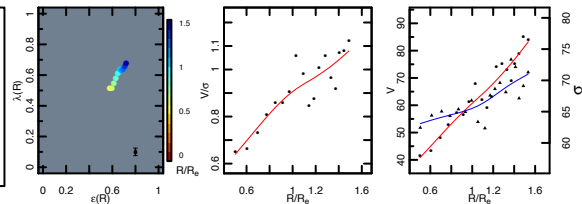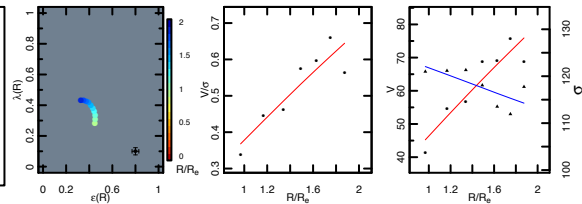

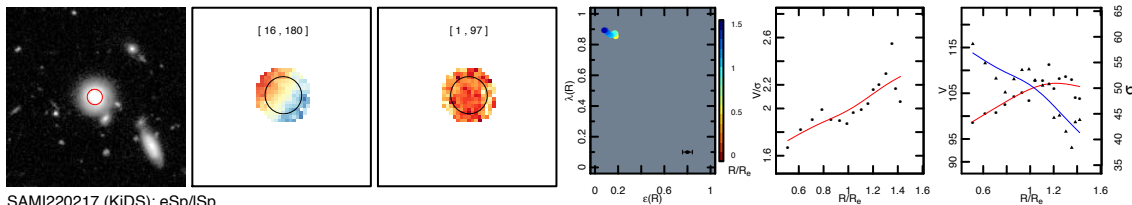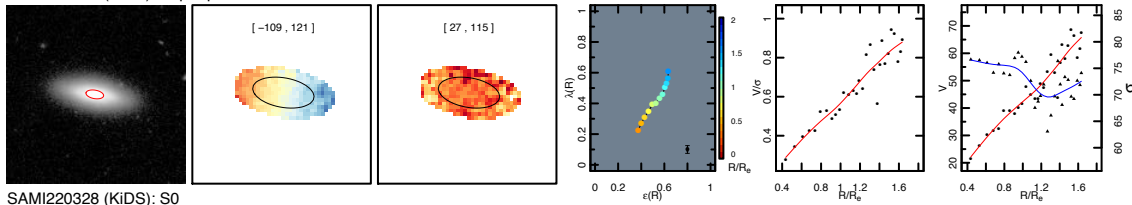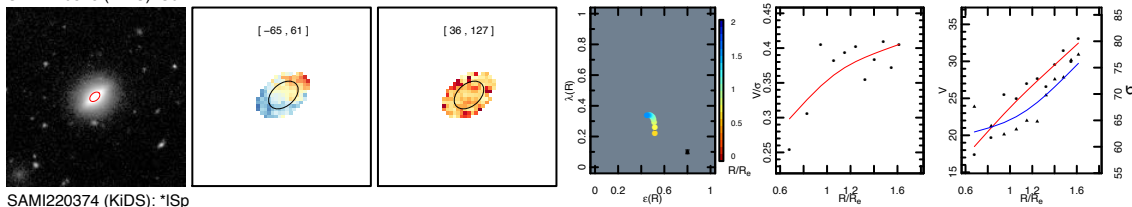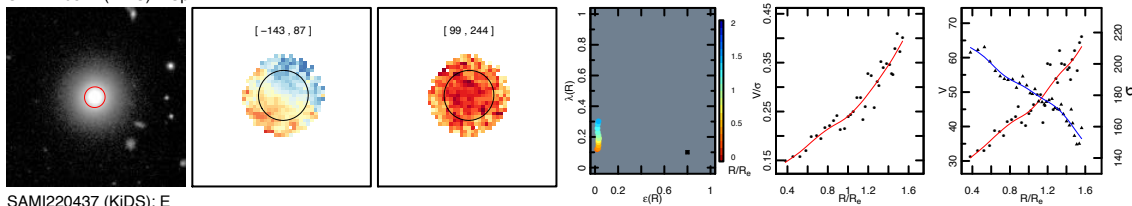

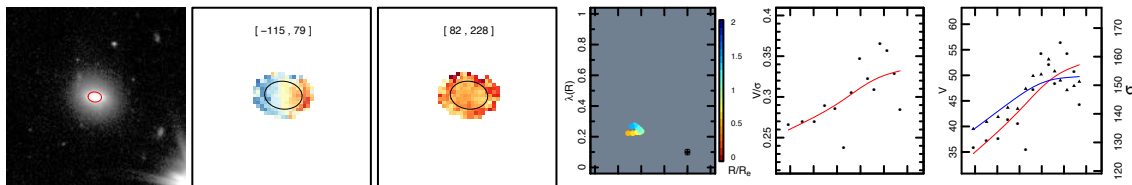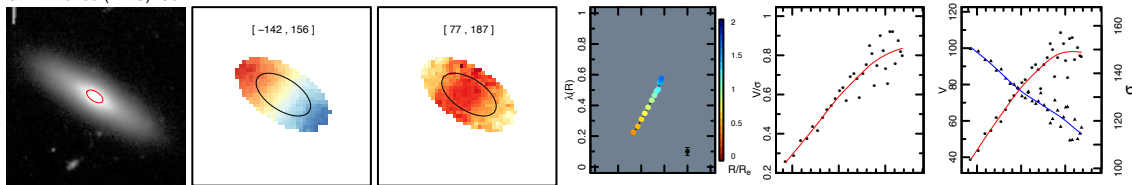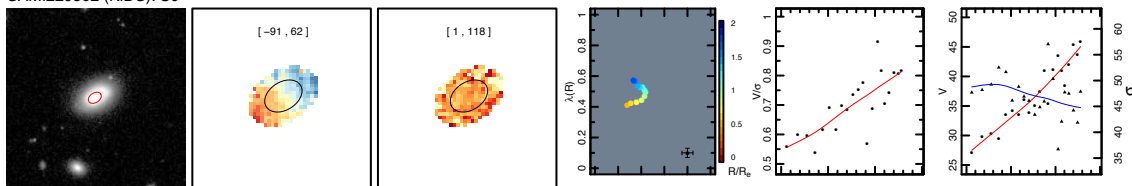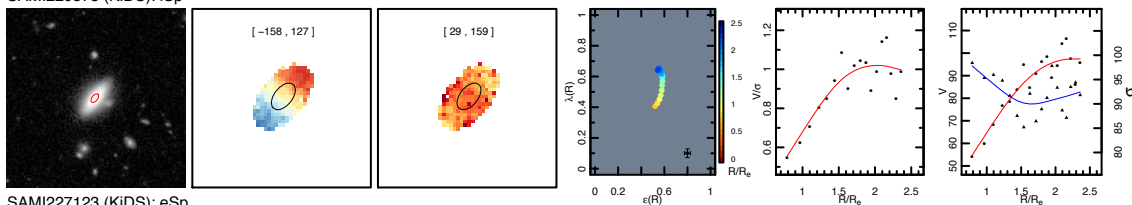

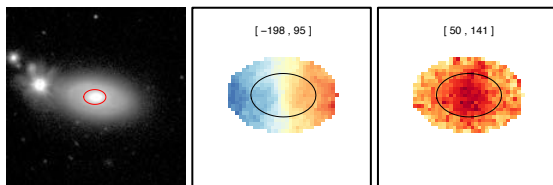

SAMI227264 (KiDS): S0/eSp

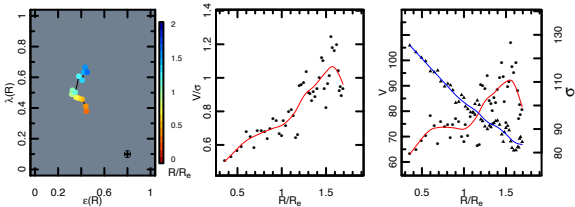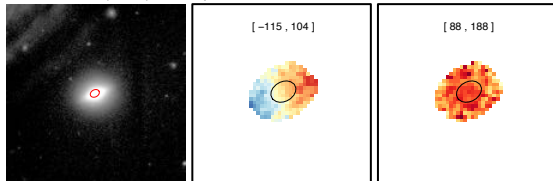

SAMI227278 (KiDS): S0

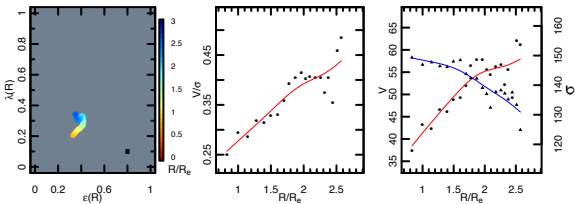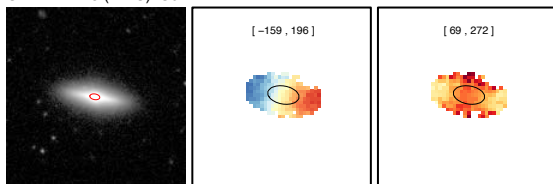

SAMI227905 (KiDS): S0

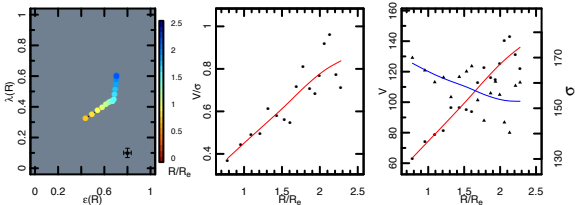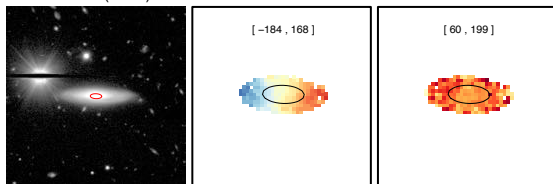

SAMI228066 (HSC): \*S0

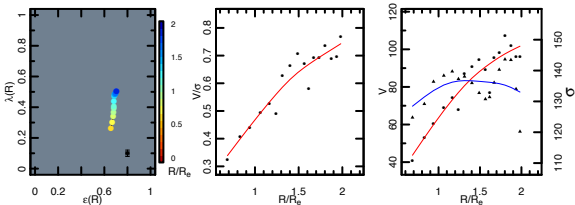

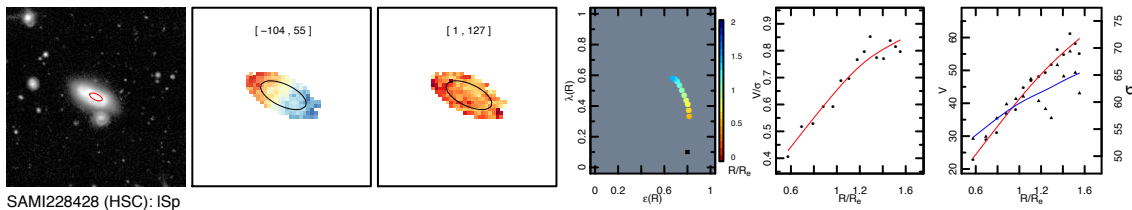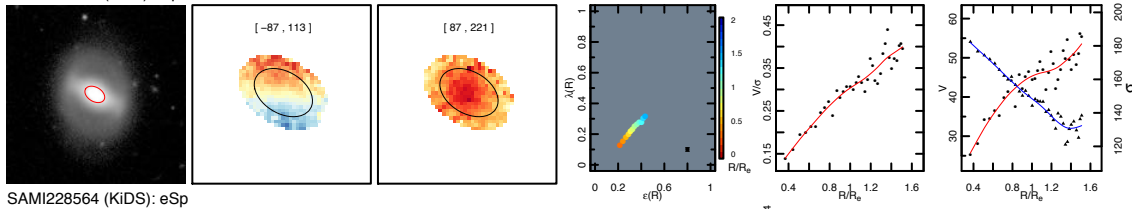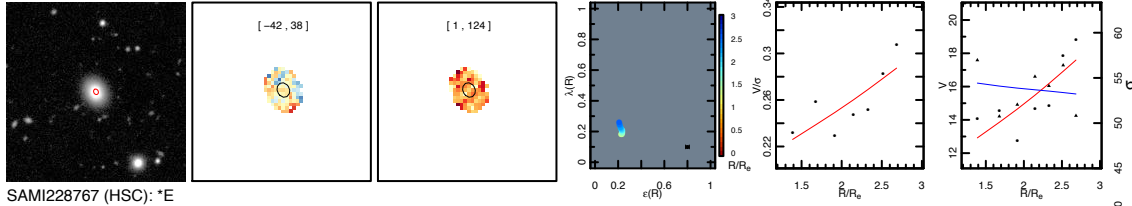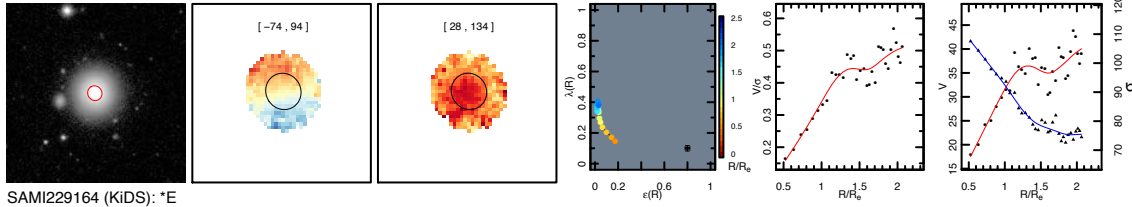



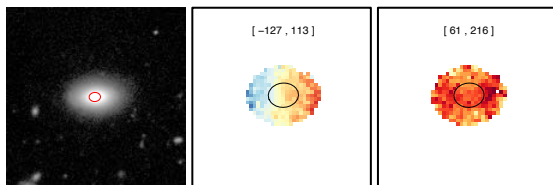

SAMI230421 (KiDS): S0

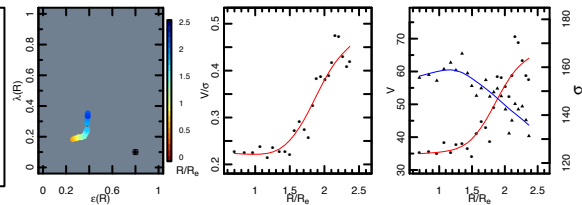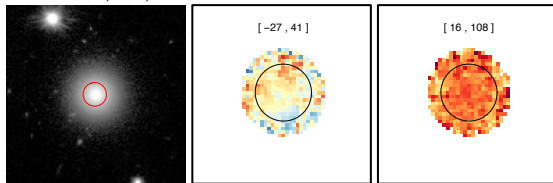

SAMI230683 (KiDS): E

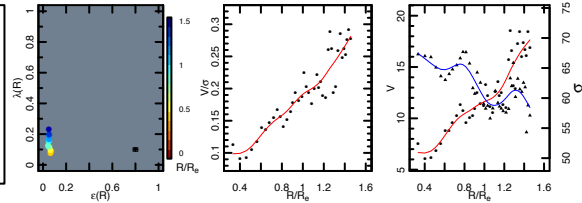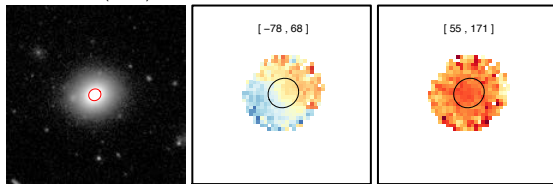

SAMI230786 (KiDS): E

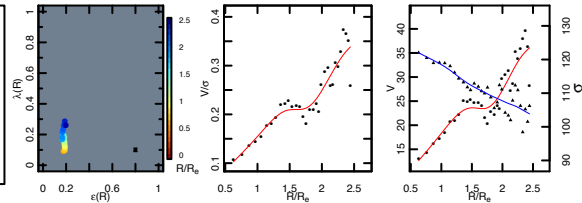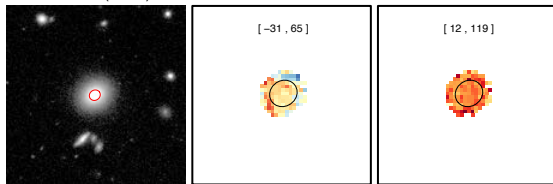

SAMI230787 (KiDS): E

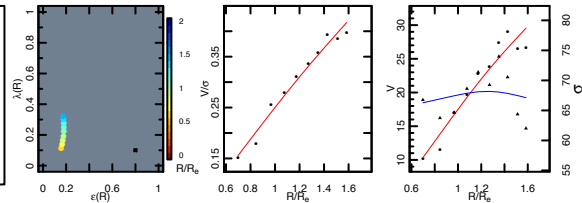

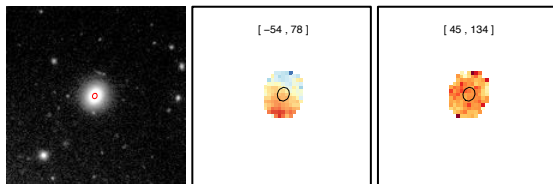

SAMI230789 (KiDS): \*E

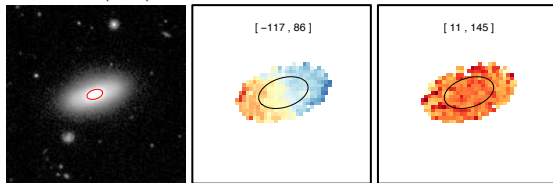

SAMI230793 (KiDS): S0

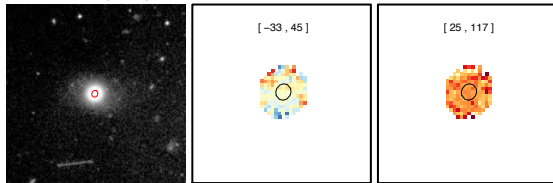

SAMI230796 (KiDS): \*E

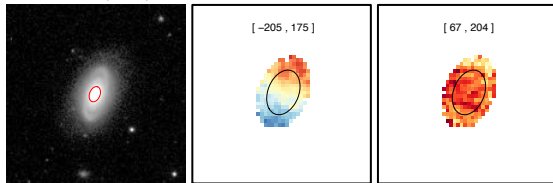

SAMI238204 (KiDS): eSp

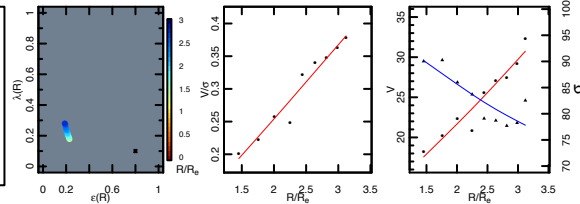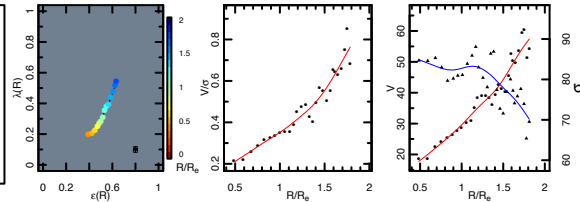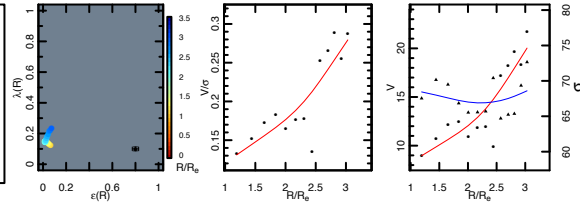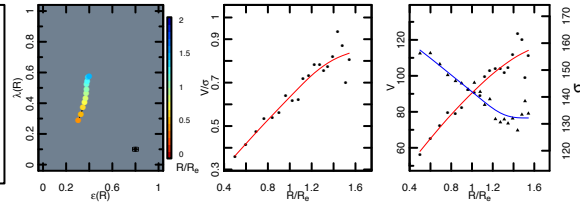

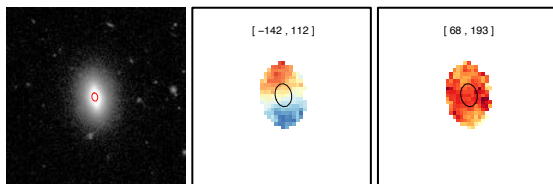

SAMI238276 (KiDS): S0

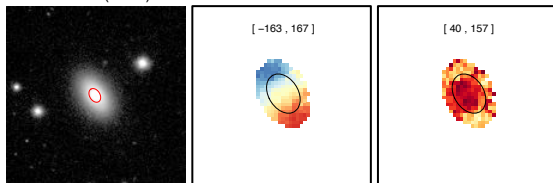

SAMI238282 (KiDS): S0

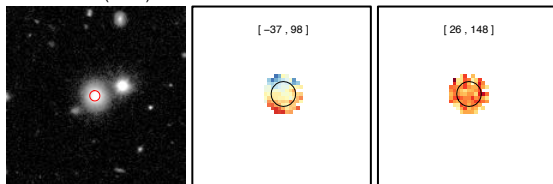

SAMI238398 (KiDS): \*E

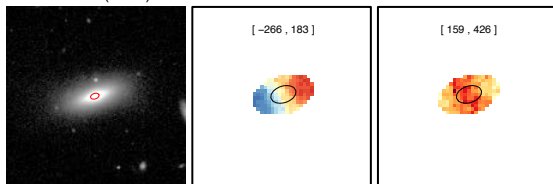

SAMI238412 (KiDS): S0

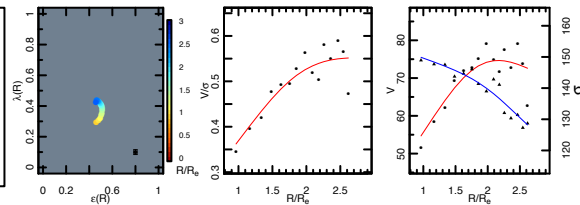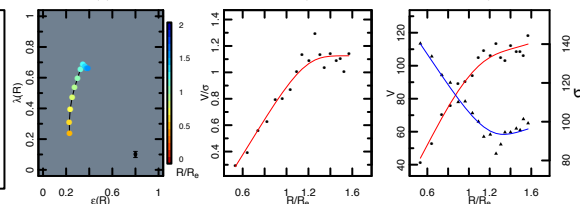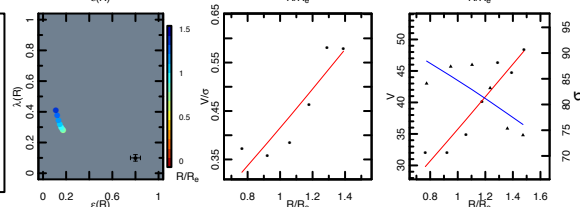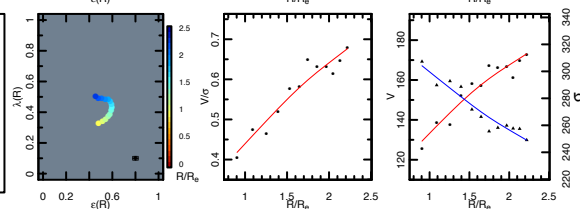

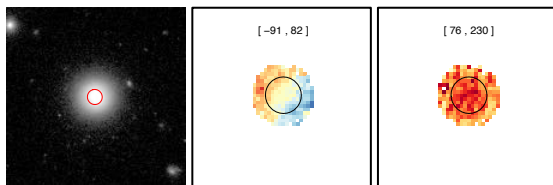

SAMI238453 (KiDS): \*E

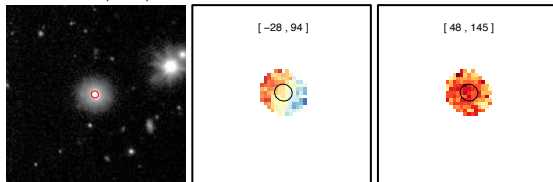

SAMI238500 (KiDS): E

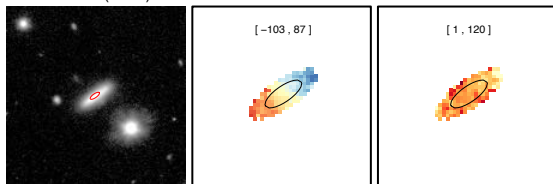

SAMI239249 (KiDS): ISp

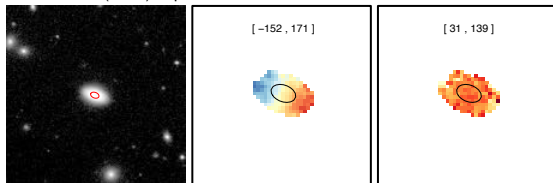

SAMI239292 (KiDS): \*S0

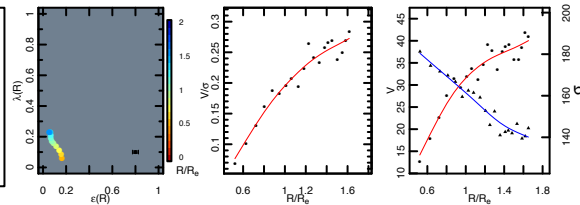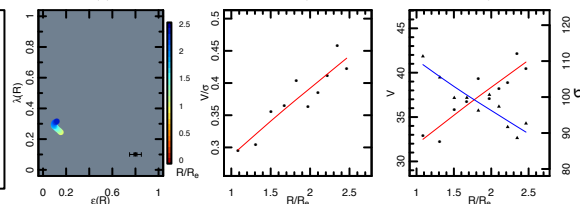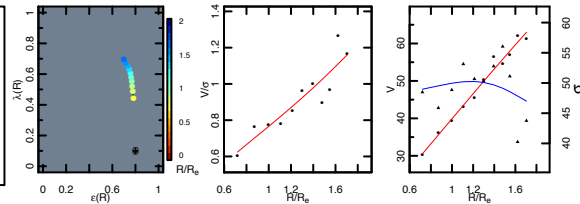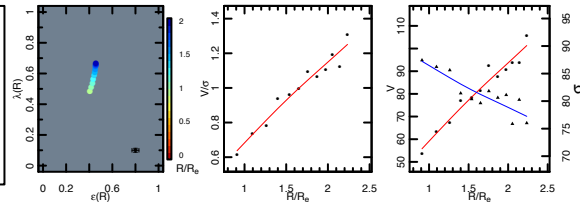

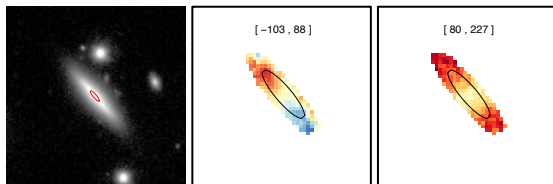

SAMI239560 (KiDS): \*2-sigma

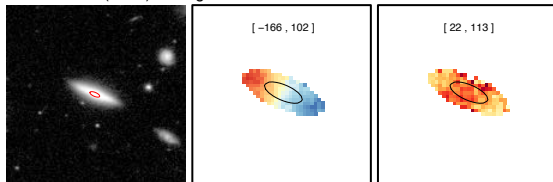

SAMI240352 (KiDS): \*S0

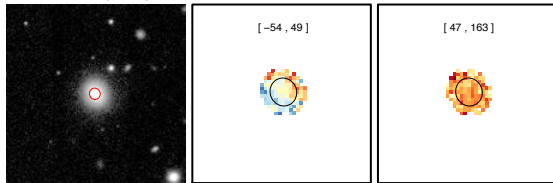

SAMI250179 (KiDS): \*E

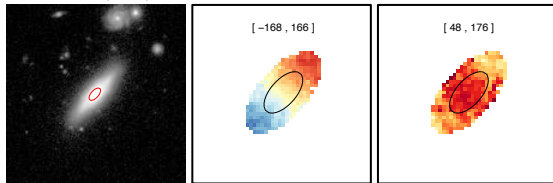

SAMI250192 (KiDS): \*S0

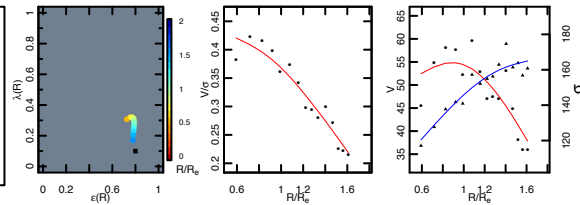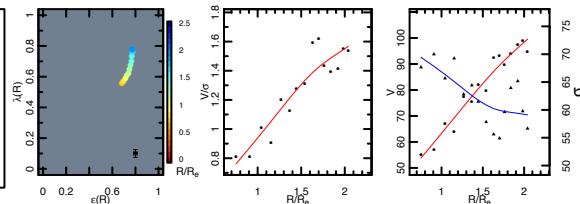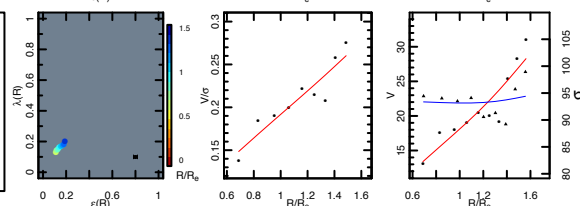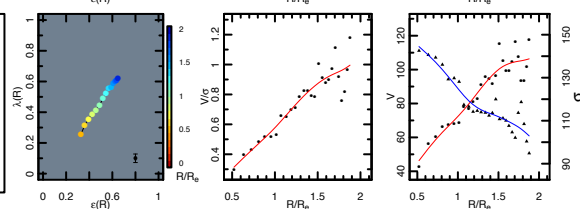

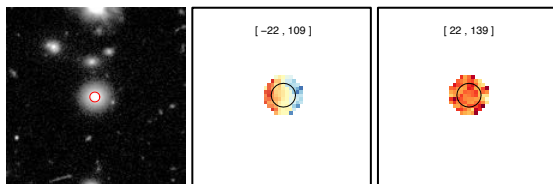

SAMI250243 (KiDS): E

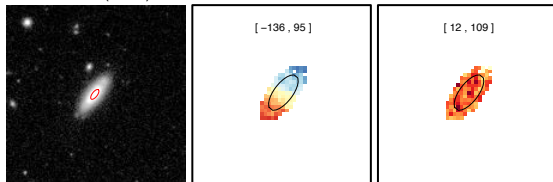

SAMI250466 (KiDS): \*eSp

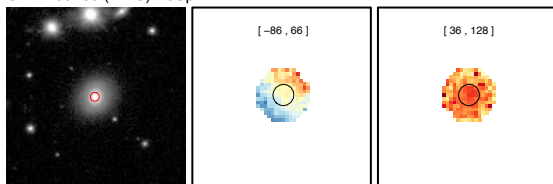

SAMI252057 (KiDS): \*S0

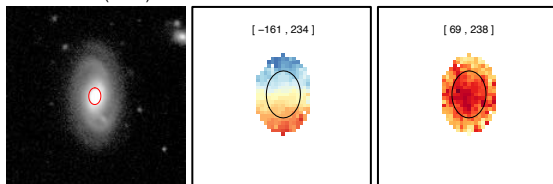

SAMI271385 (KiDS): eSp

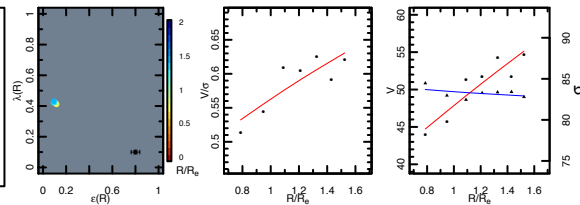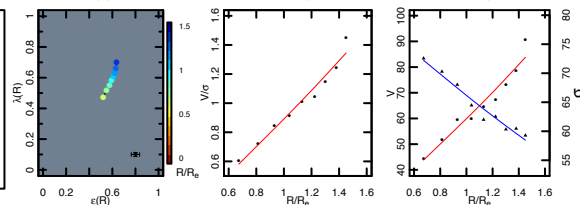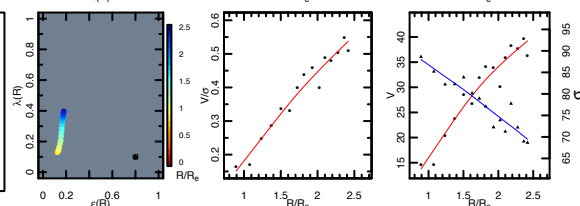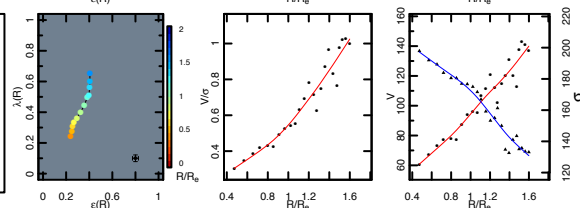

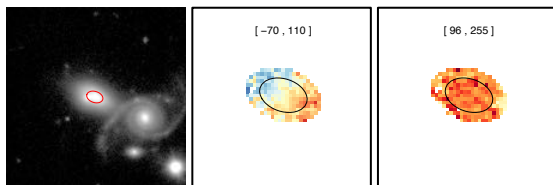

SAMI271387 (KiDS): S0

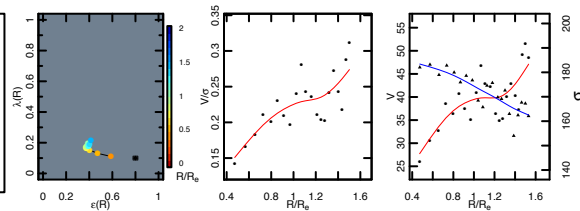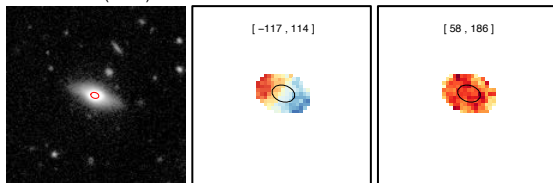

SAMI271431 (KiDS): S0/eSp

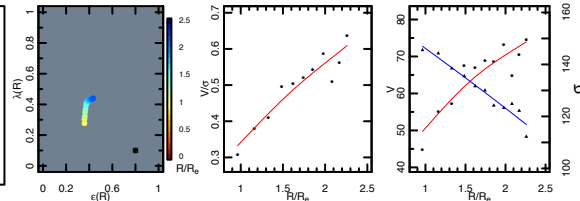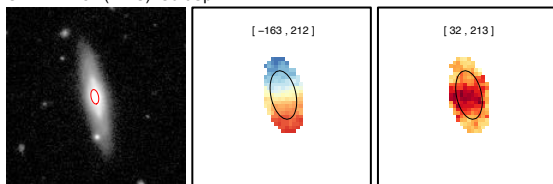

SAMI271455 (KiDS): eSp

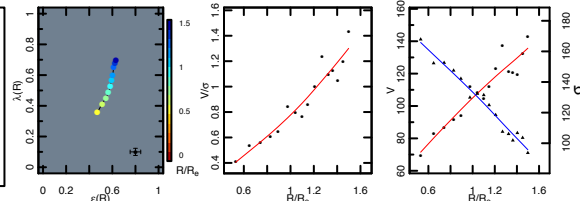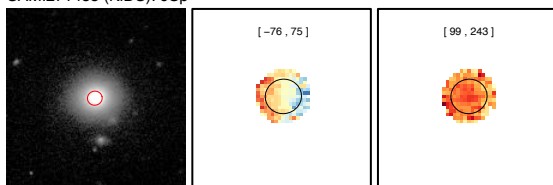

SAMI272190 (KiDS): E

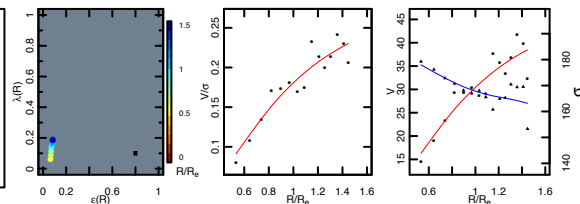

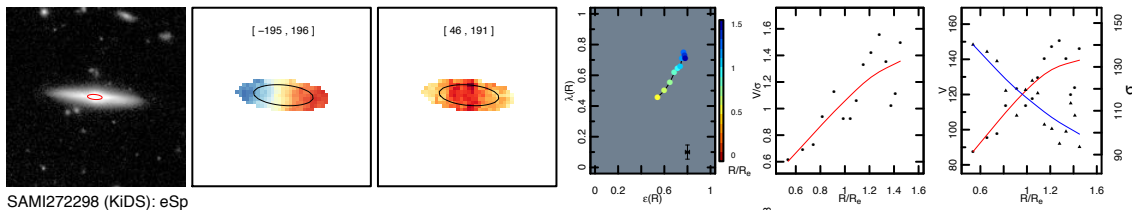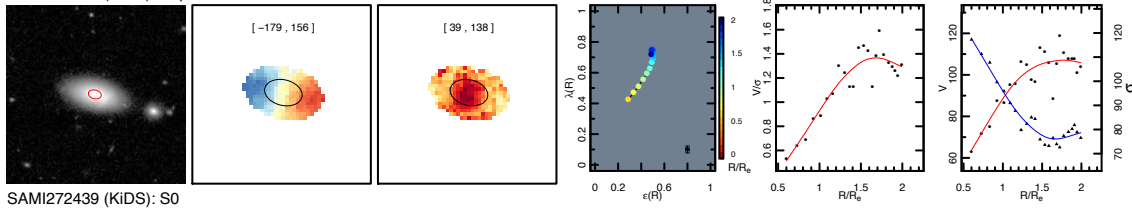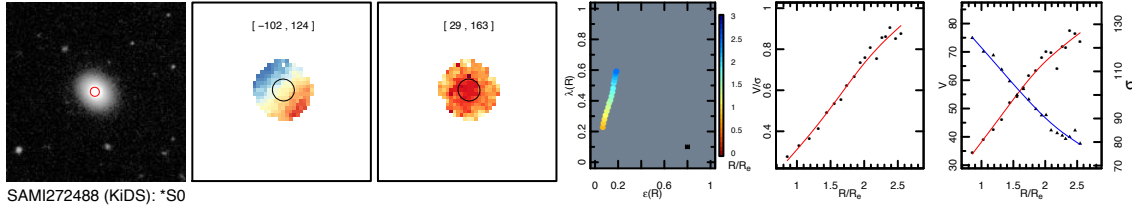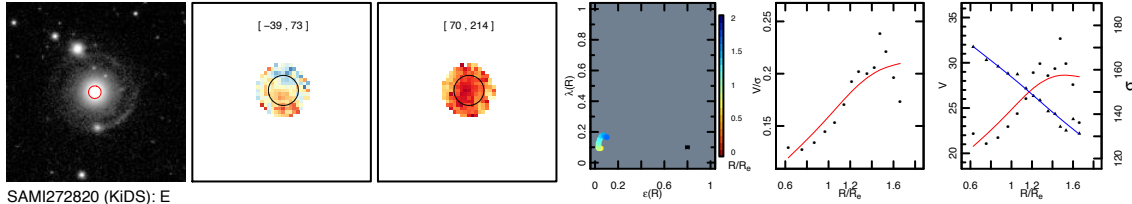



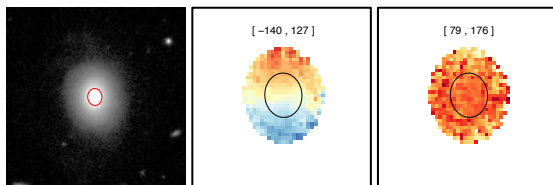

SAMI272990 (KiDS): E/S0

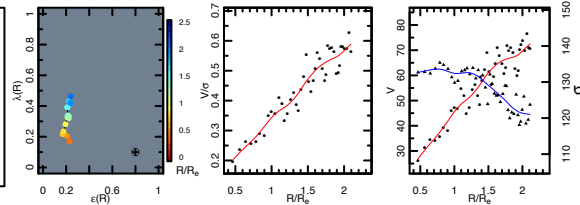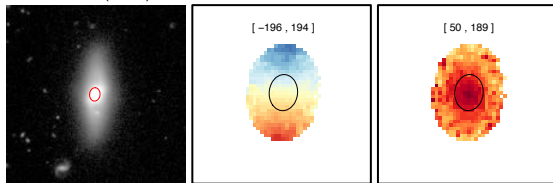

SAMI278109 (KiDS): \*eSp

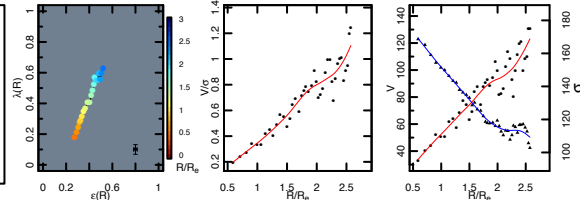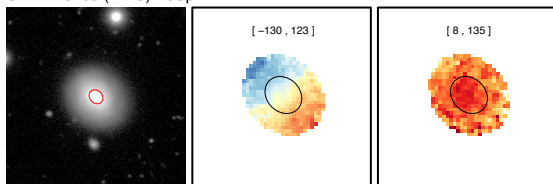

SAMI278840 (HSC): \*S0

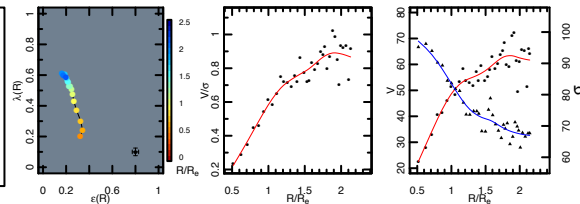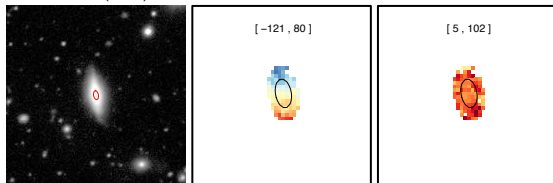

SAMI279148 (HSC): eSp/ISp

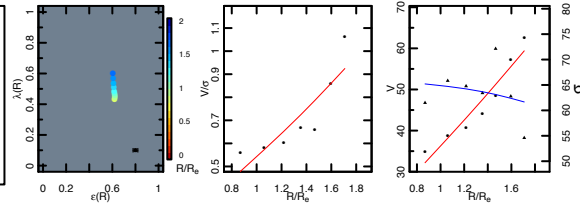

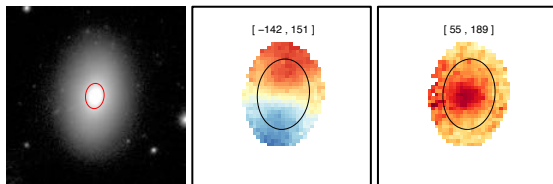

SAMI279905 (KiDS): \*S0

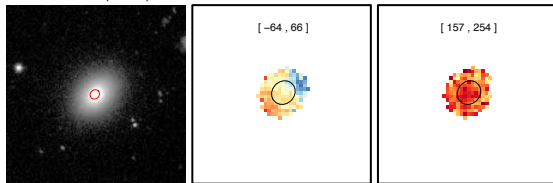

SAMI279910 (KiDS): \*E

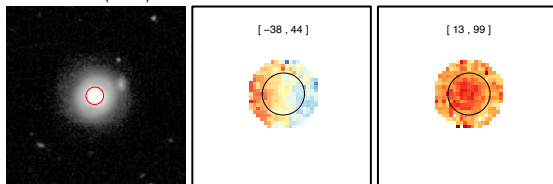

SAMI287827 (KiDS): S0/eSp

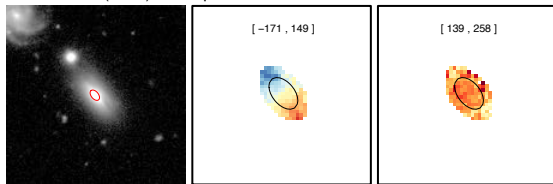

SAMI288679 (KiDS): S0

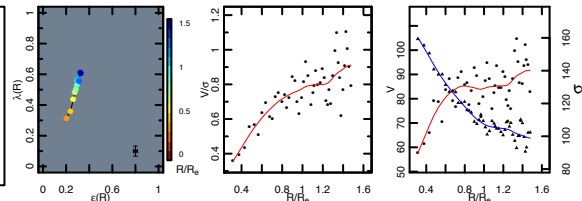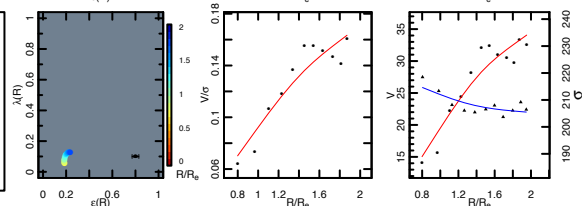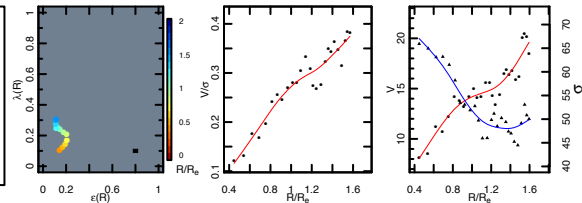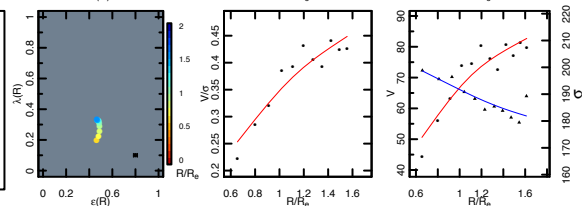

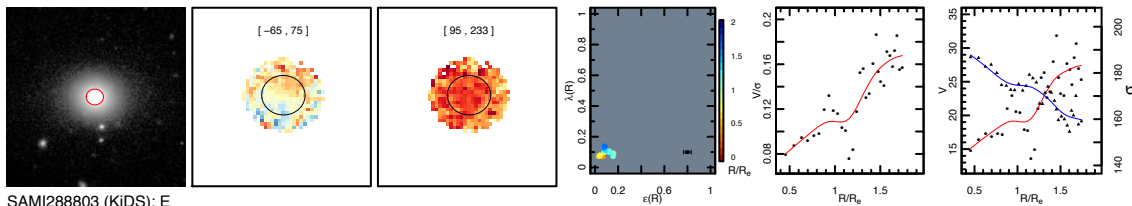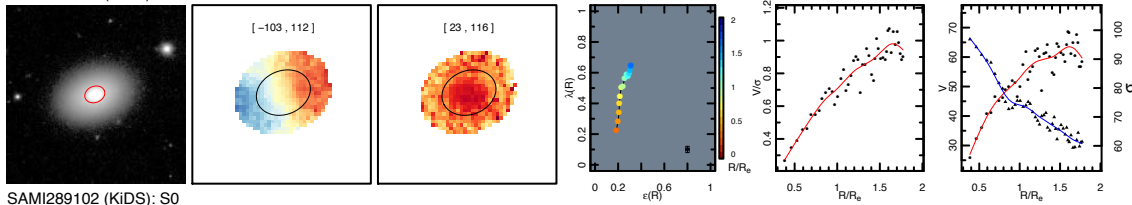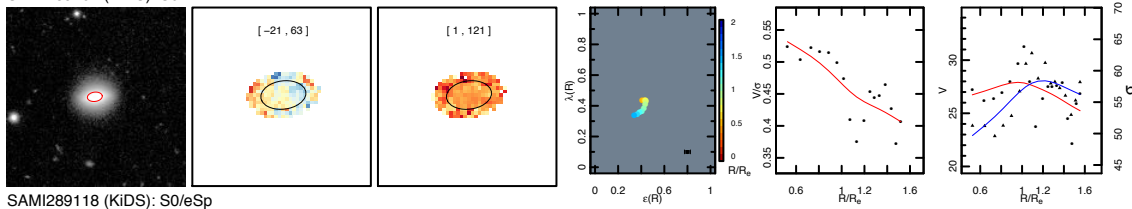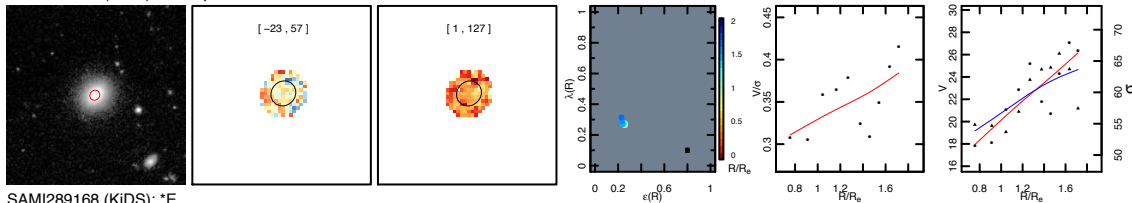

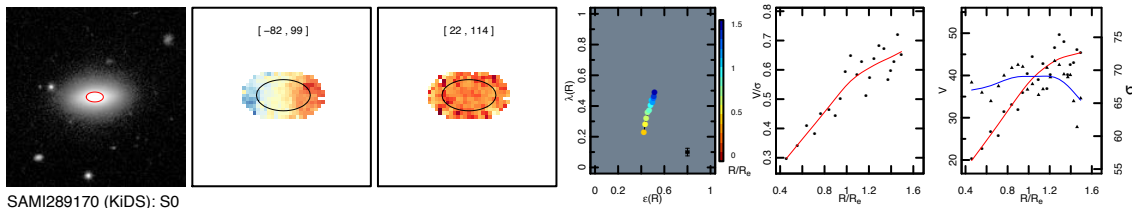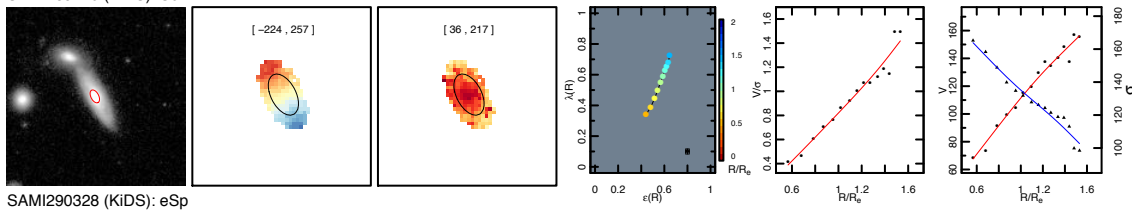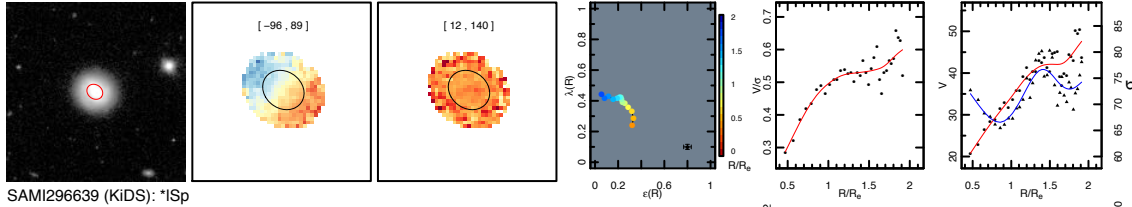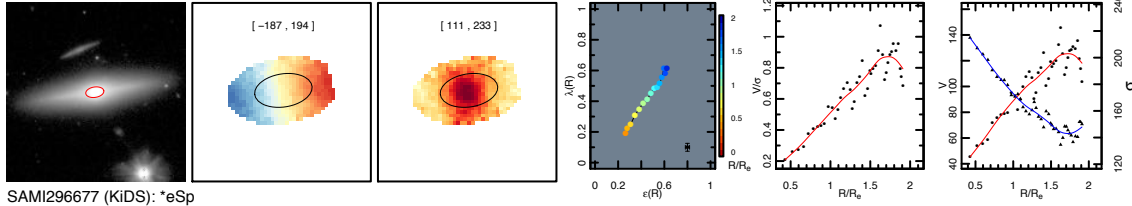

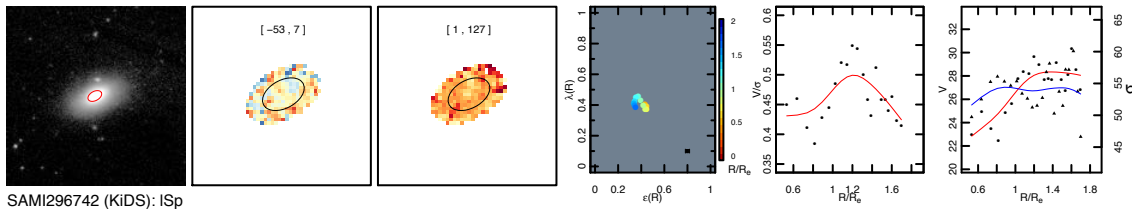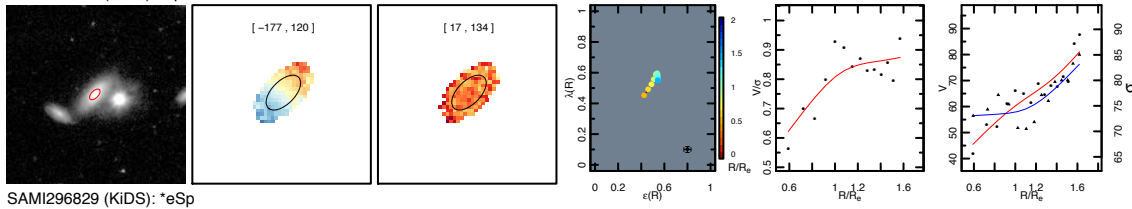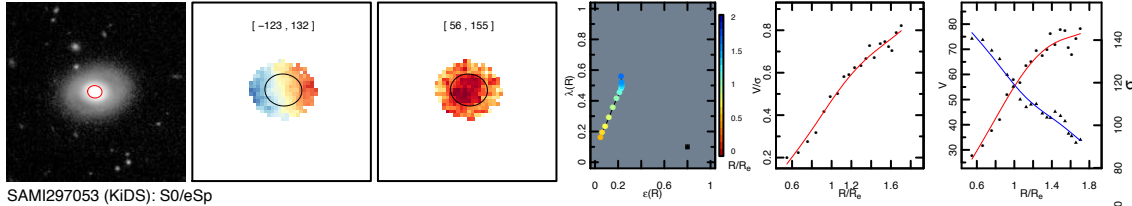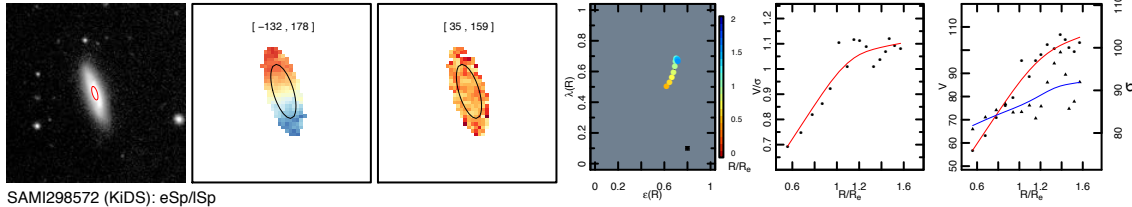

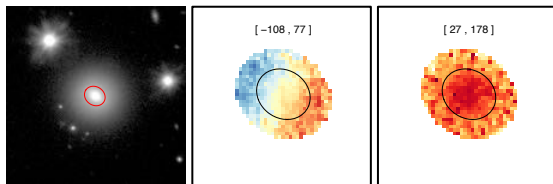

SAMI298590 (KiDS): E

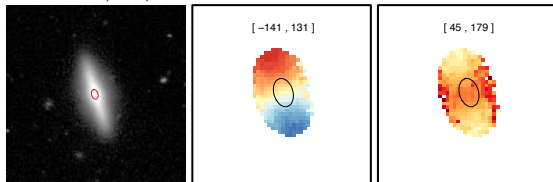

SAMI298591 (KiDS): \*eSp

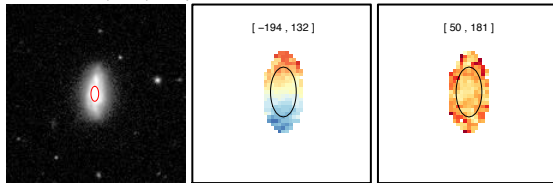

SAMI298862 (KiDS): eSp/Sp

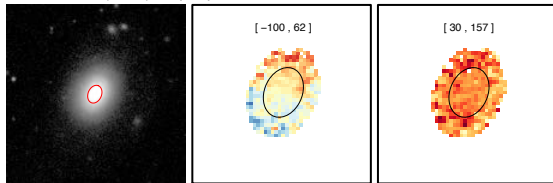

SAMI298980 (KiDS): \*E

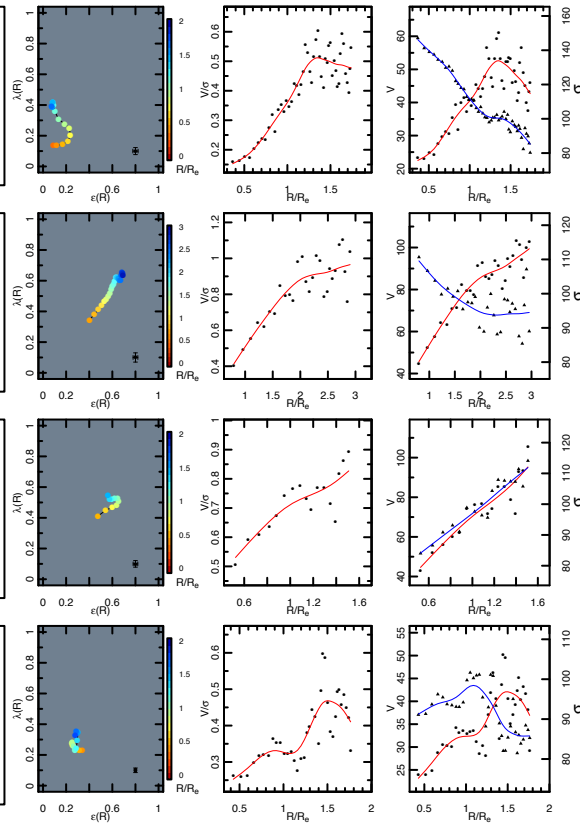

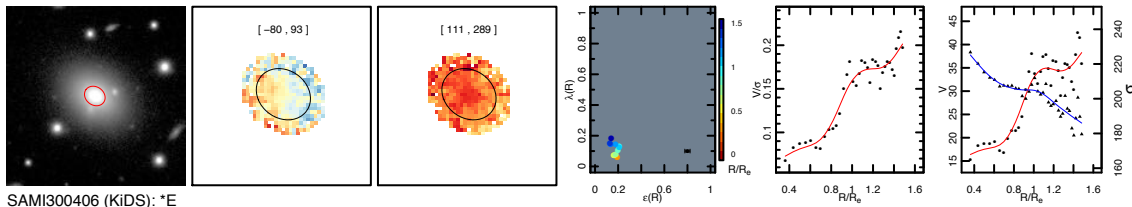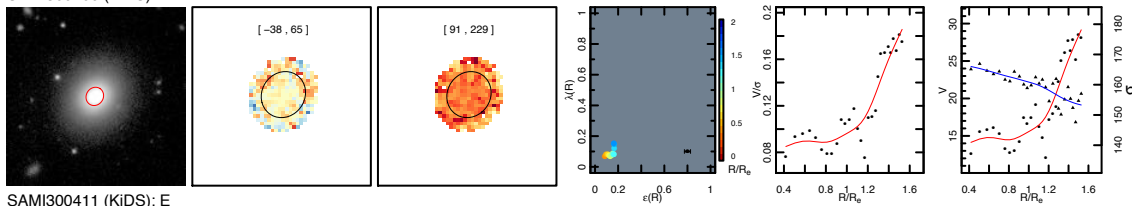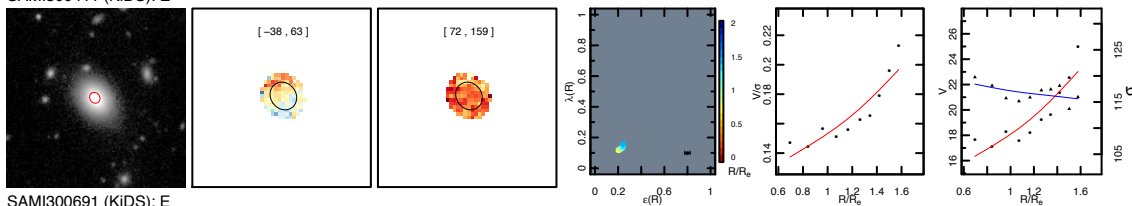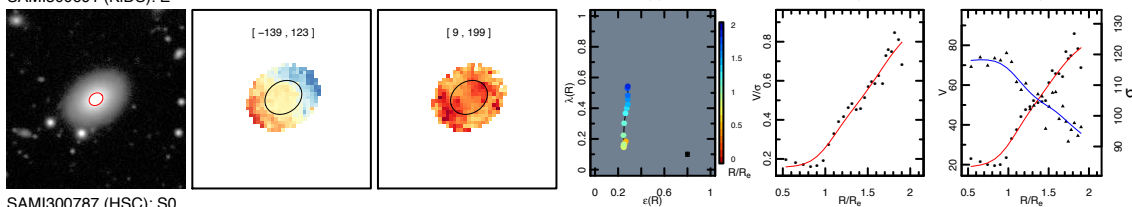

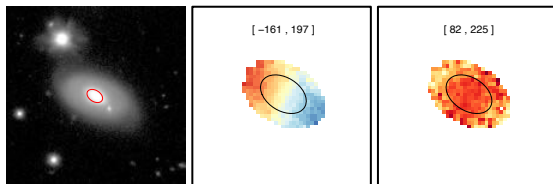

SAMI301191 (KiDS): \*eSp

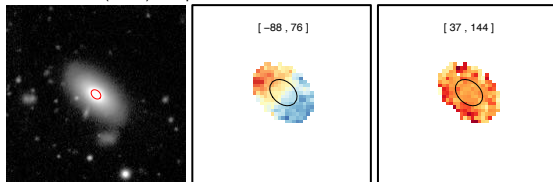

SAMI301199 (HSC): S0/eSp

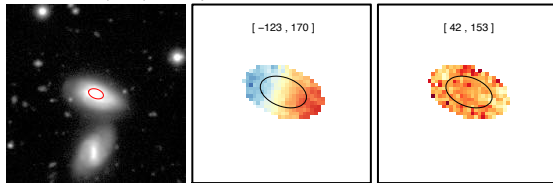

SAMI301346 (HSC): \*ISp

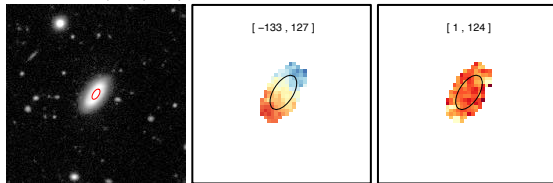

SAMI301799 (HSC): ?

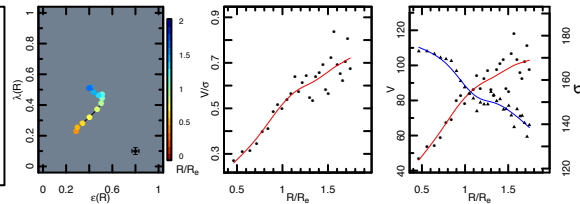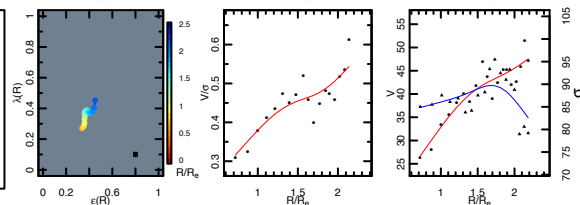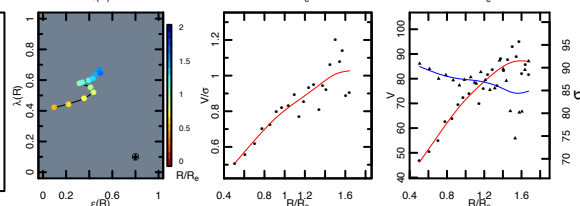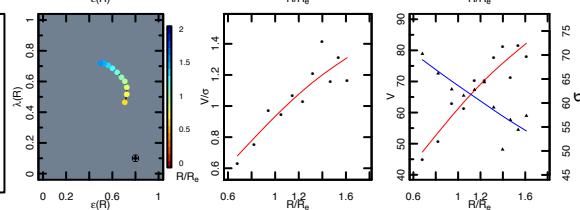



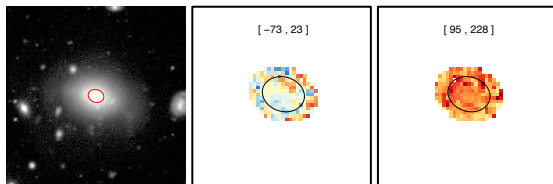

SAMI301937 (HSC): \*Merger

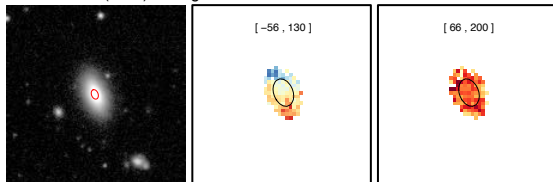

SAMI302684 (KiDS): S0

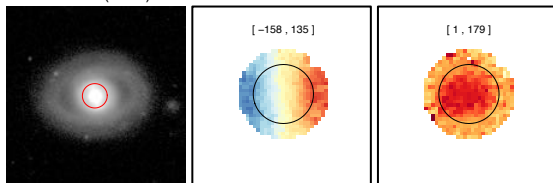

SAMI303099 (KiDS): eSp

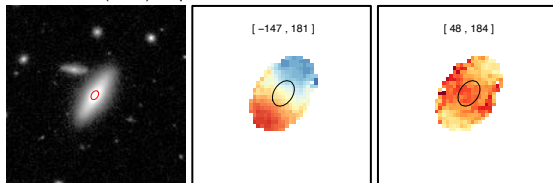

SAMI319060 (KiDS): S0

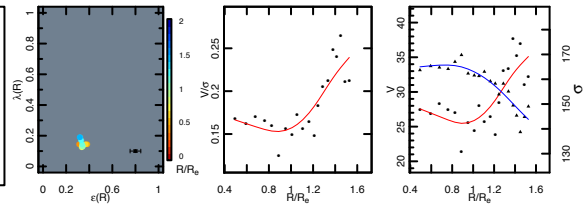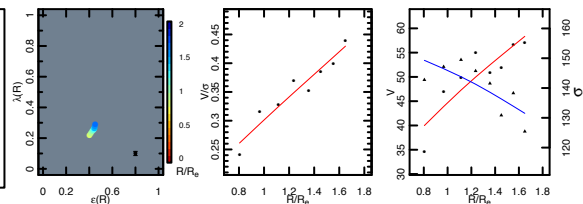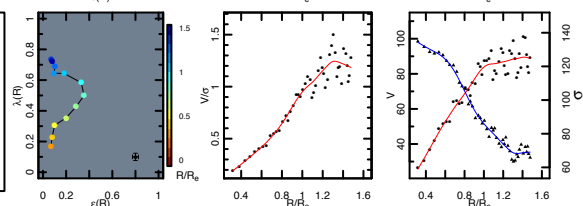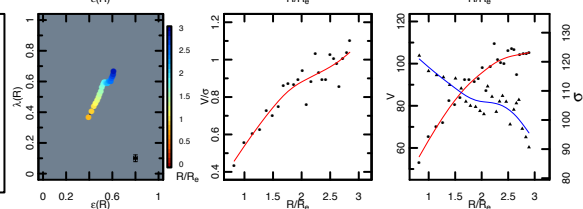

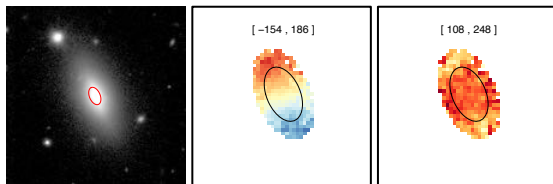

SAMI319067 (KiDS): S0

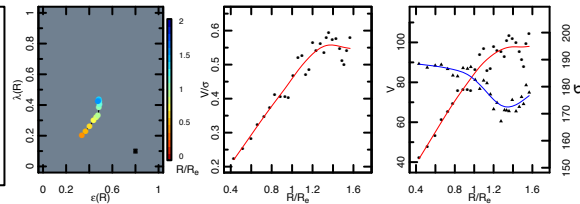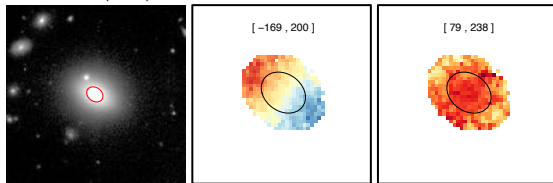

SAMI319070 (KiDS): E/S0

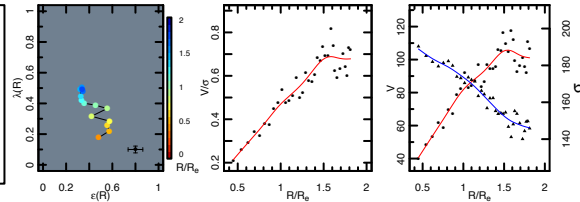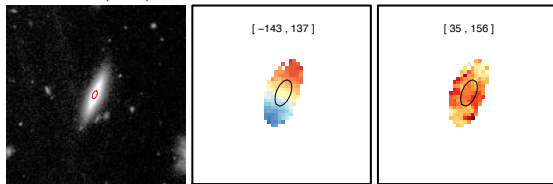

SAMI319157 (KiDS): \*S0

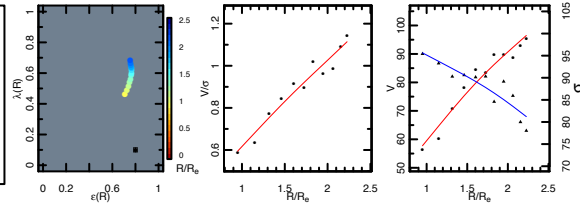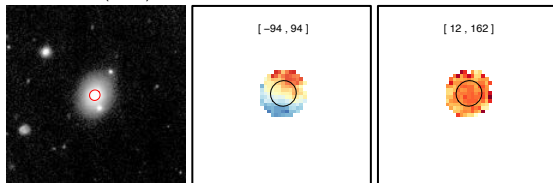

SAMI319196 (KiDS): E/S0

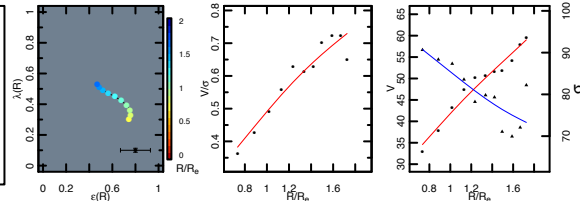

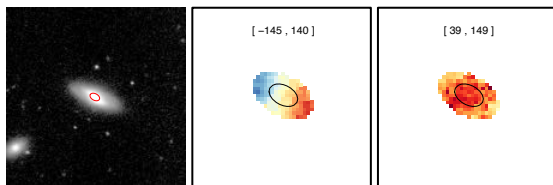

SAMI319197 (KiDS): \*S0

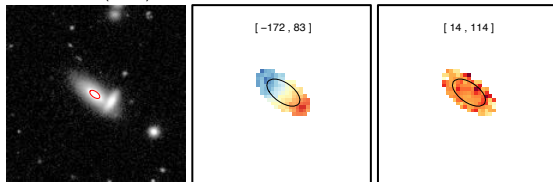

SAMI319393 (KiDS): ISp

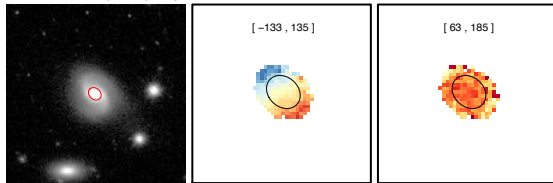

SAMI319397 (KiDS): eSp

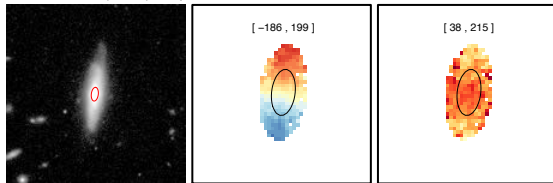

SAMI319400 (KiDS): eSp

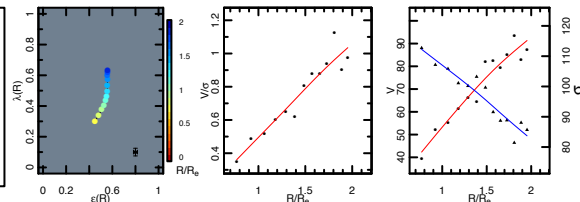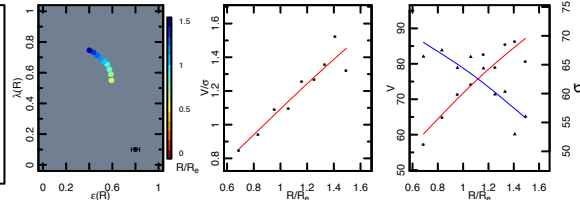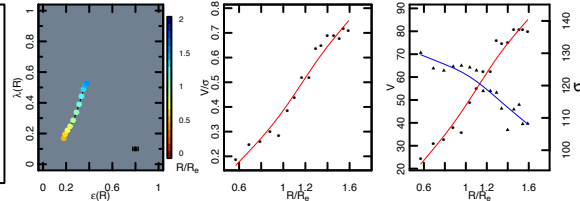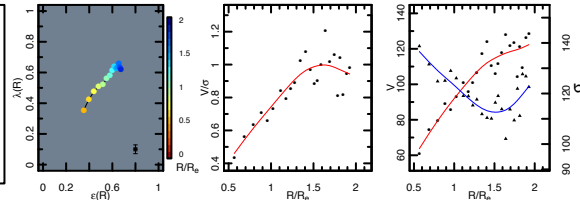

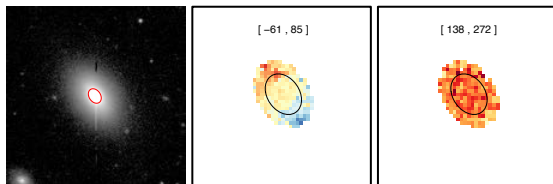

SAMI319402 (KiDS): \*E

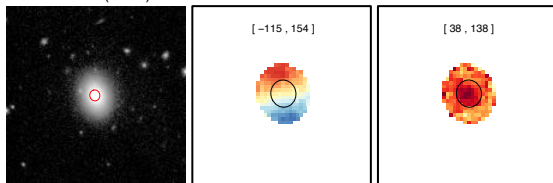

SAMI319452 (KiDS): S0

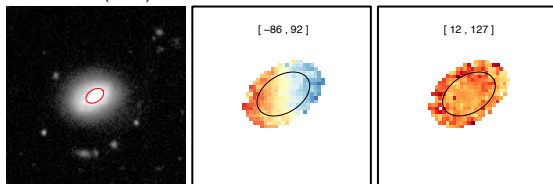

SAMI320281 (KiDS): ISP

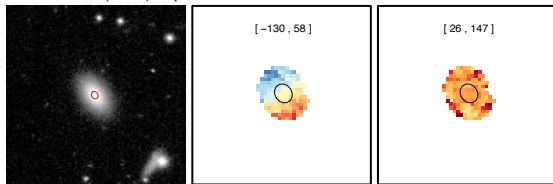

SAMI321035 (KiDS): S0

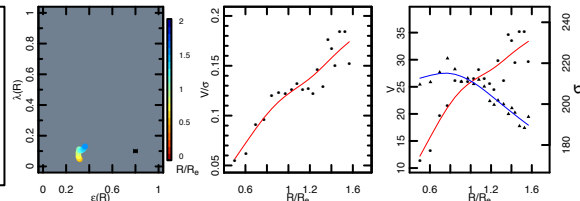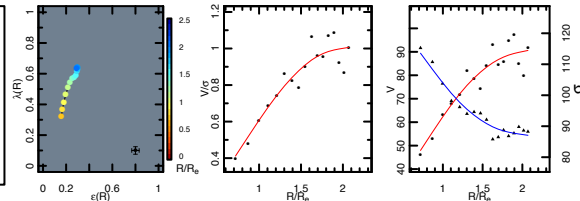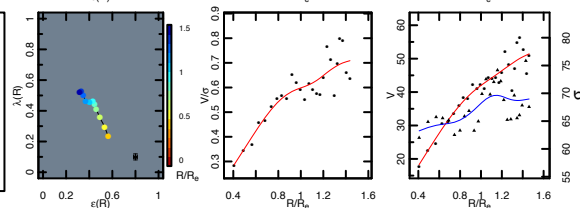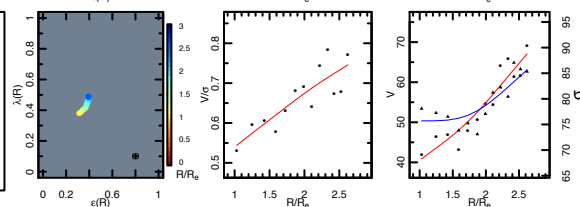

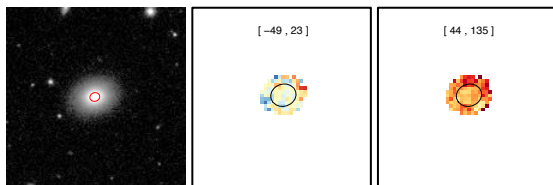

SAMI321146 (KiDS): \*E

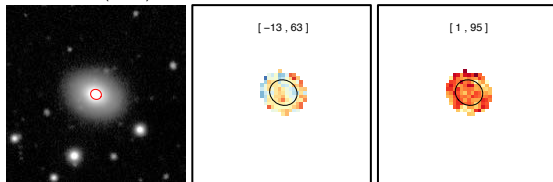

SAMI323242 (HSC): ?

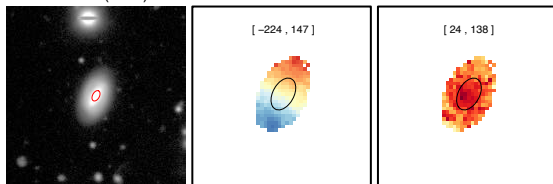

SAMI323329 (HSC): eSp

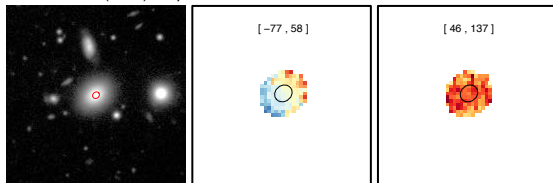

SAMI323566 (HSC): E

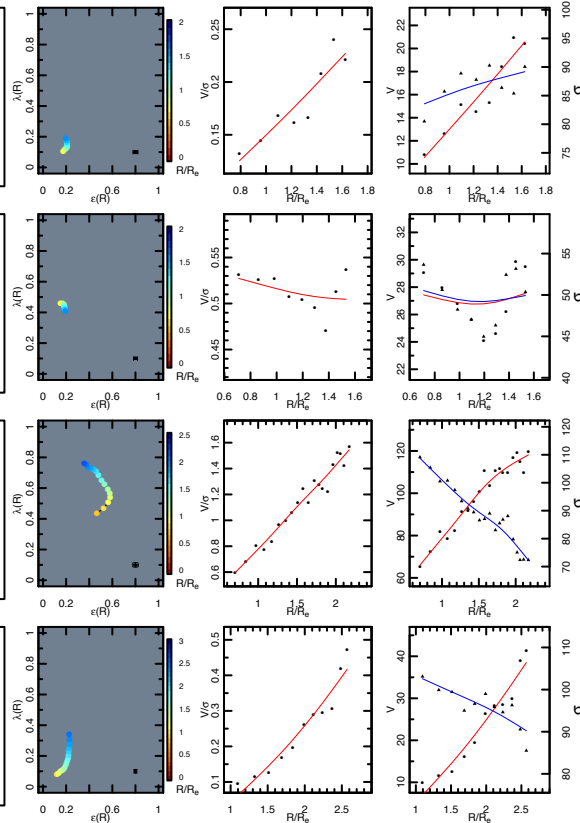

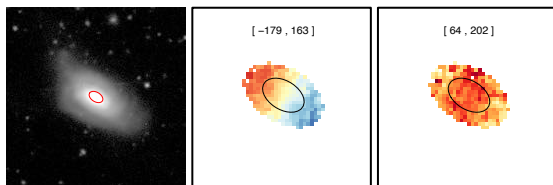

SAMI323854 (HSC): \*Merger

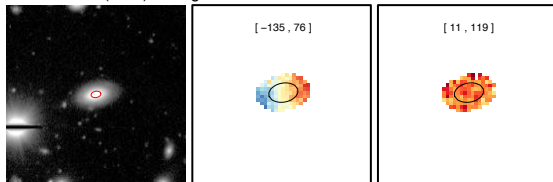

SAMI324323 (HSC): ISp

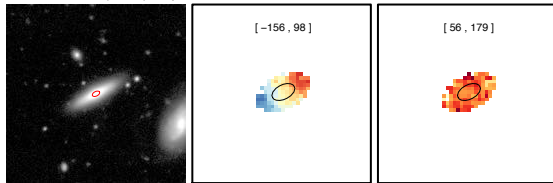

SAMI324351 (HSC): SO/eSp

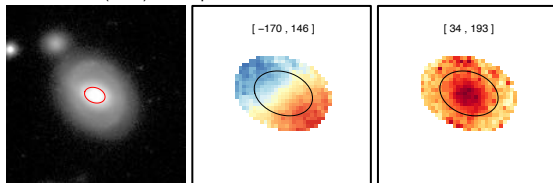

SAMI325007 (KiDS): eSp

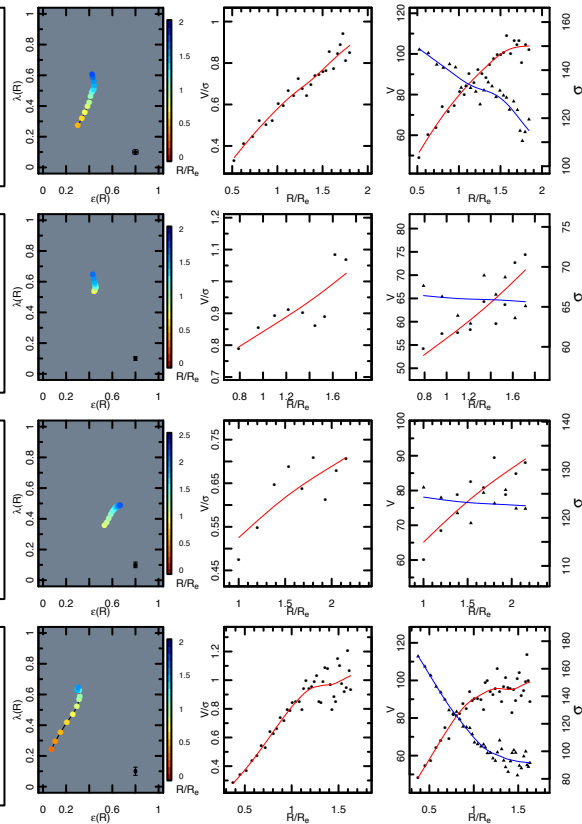

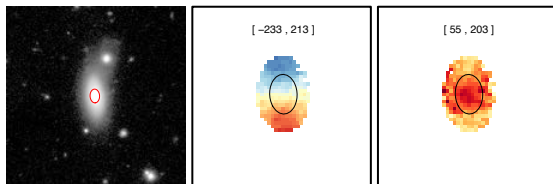

SAMI325321 (KiDS): S0

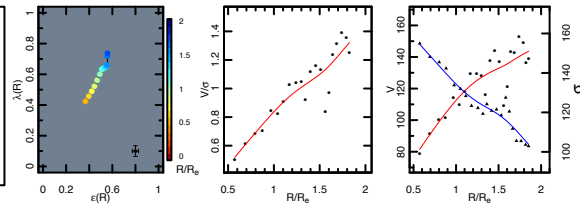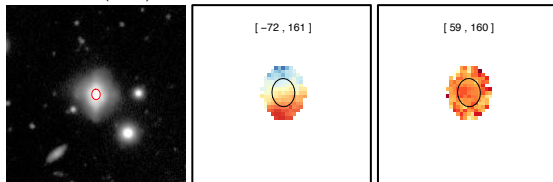

SAMI345820 (HSC): \*S0

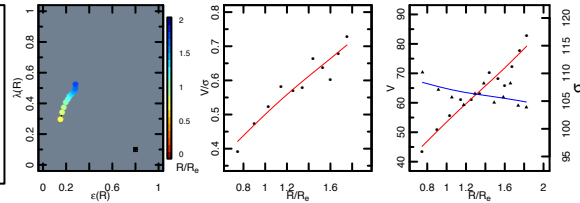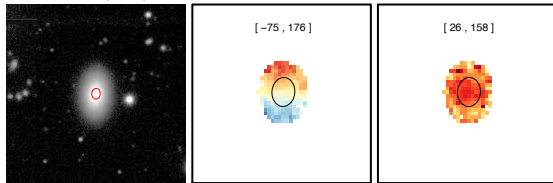

SAMI346046 (HSC): S0

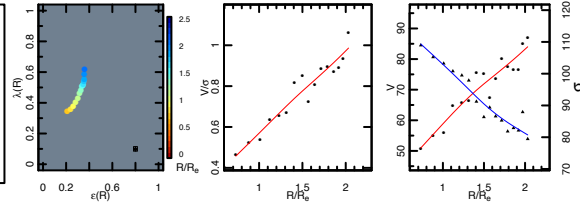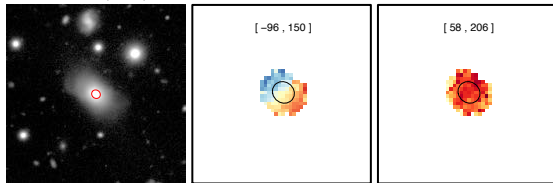

SAMI346623 (HSC): \*S0

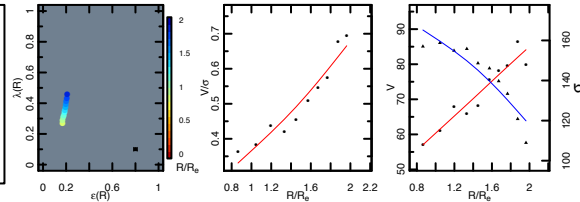

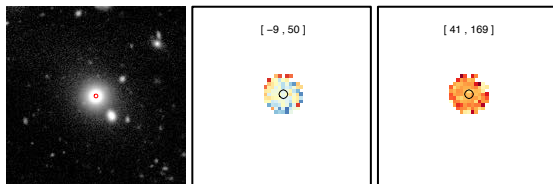

SAMI346837 (HSC): E

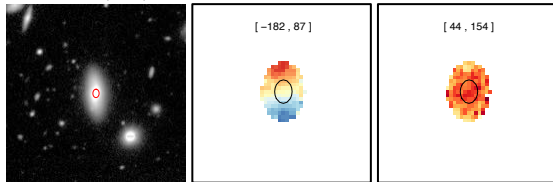

SAMI346839 (HSC): S0

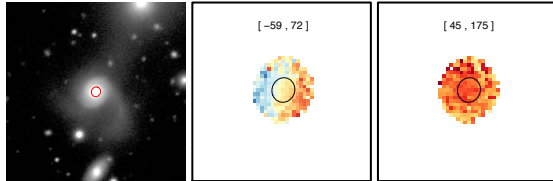

SAMI346887 (HSC): \*Merger

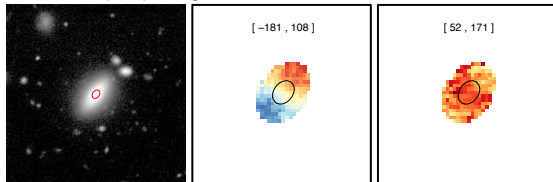

SAMI346890 (HSC): S0

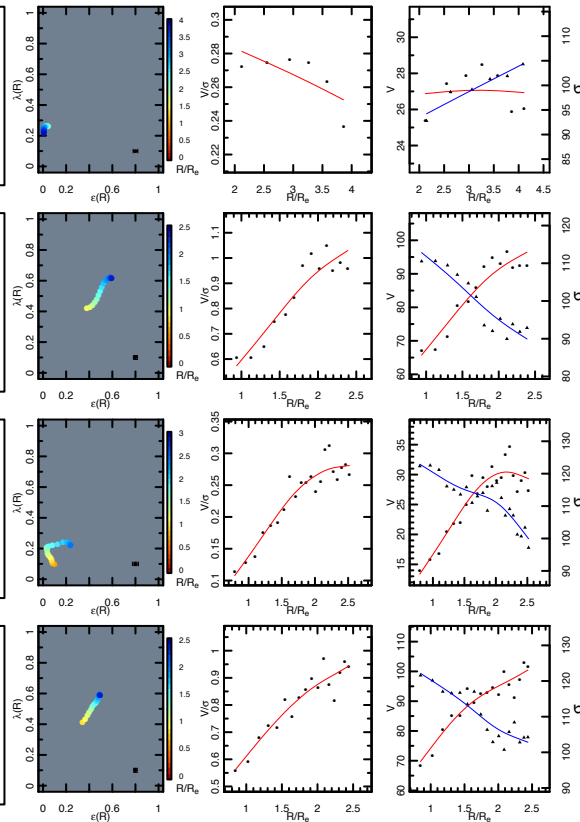



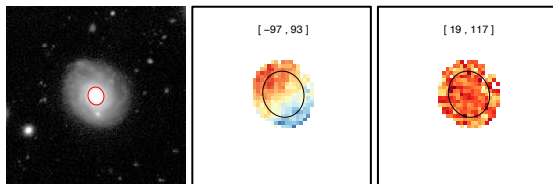

SAMI346892 (HSC): eSp

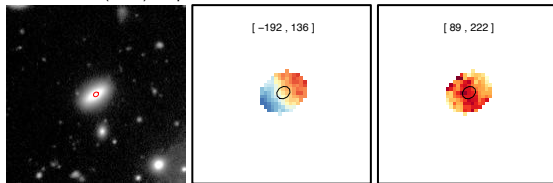

SAMI346894 (HSC): \*eSp

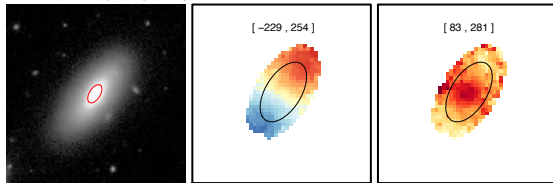

SAMI347432 (KiDS): \*Embedded Disc

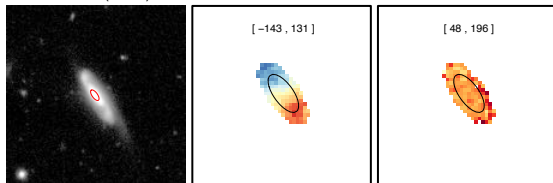

SAMI347470 (KiDS): eSp

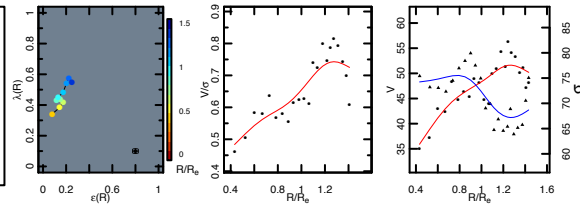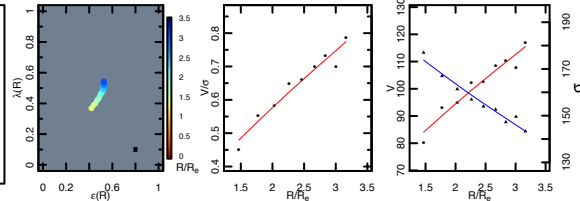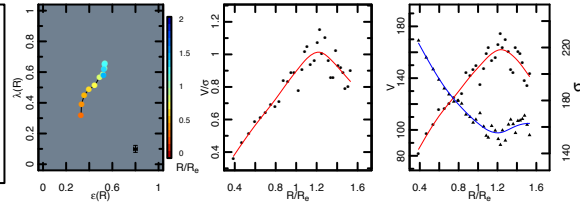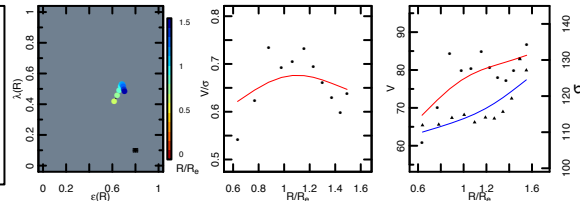

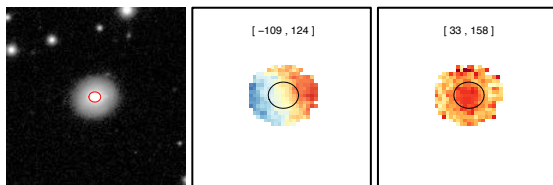

SAMI365334 (KiDS): eSp

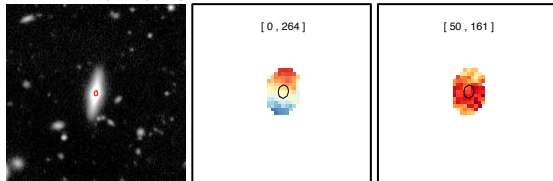

SAMI371145 (HSC): S0/eSp

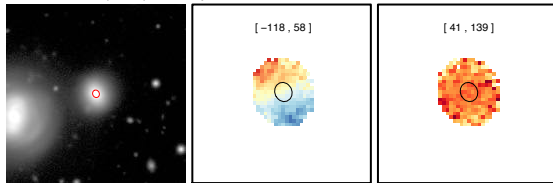

SAMI371171 (HSC): E

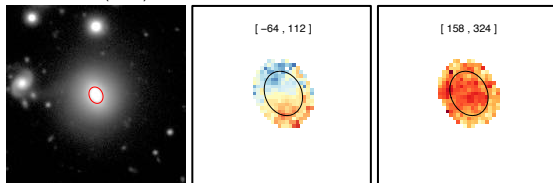

SAMI371172 (HSC): E

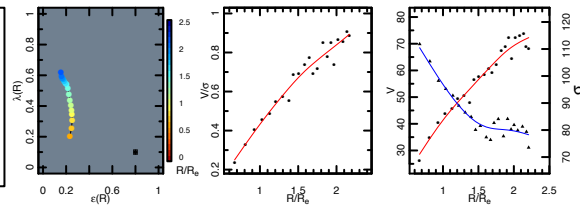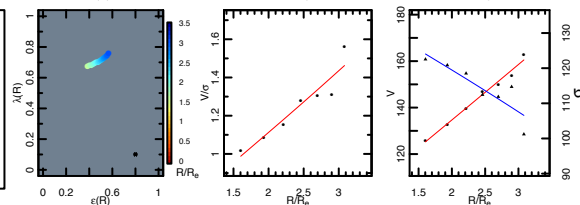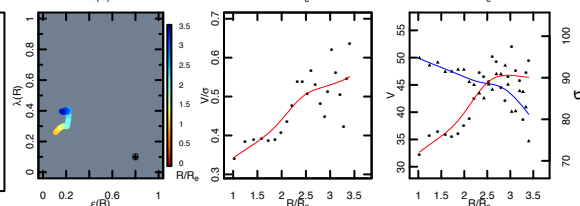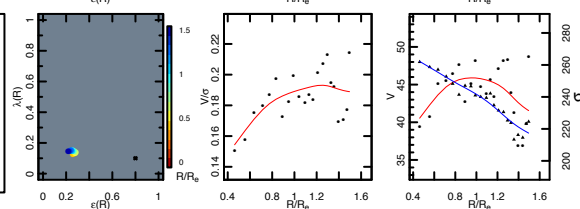

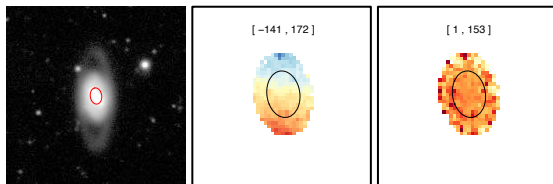

SAMI371789 (HSC): eSp

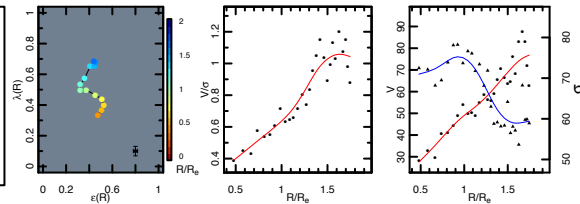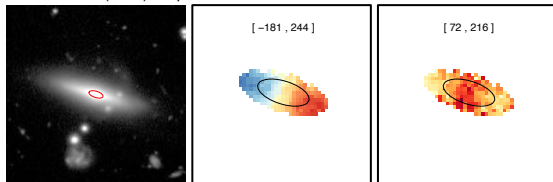

SAMI371889 (HSC): \*eSp

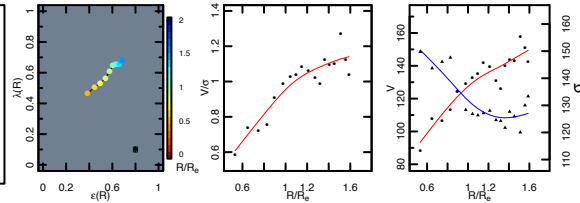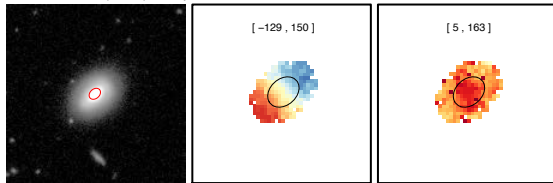

SAMI371976 (KiDS): S0

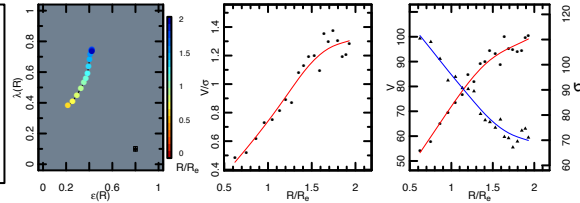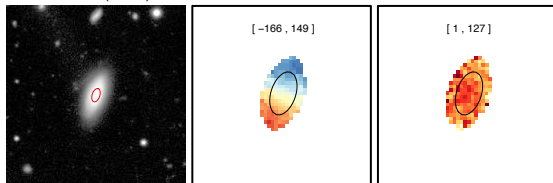

SAMI372105 (HSC): \*S0

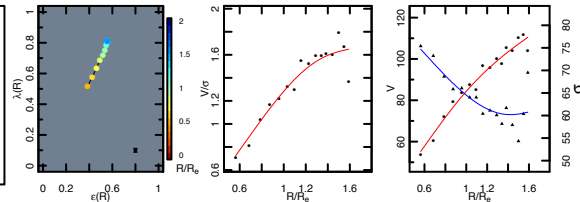

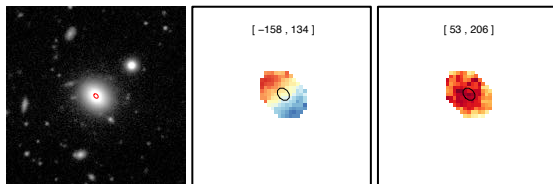

SAMI372133 (HSC): \*S0

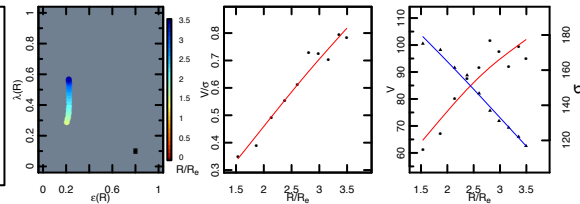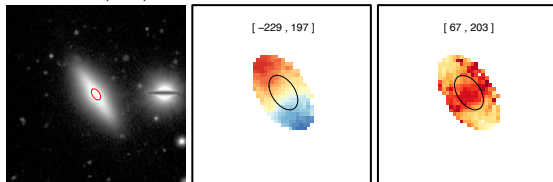

SAMI372408 (HSC): S0

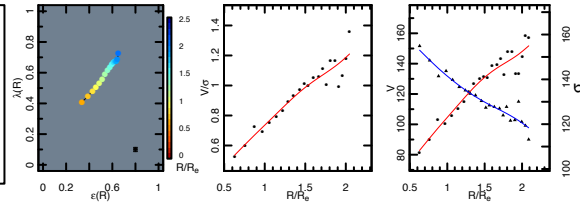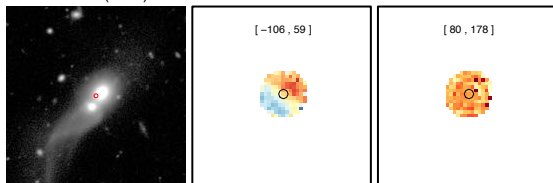

SAMI372446 (HSC): \*Merger

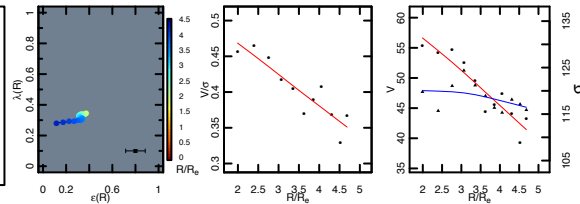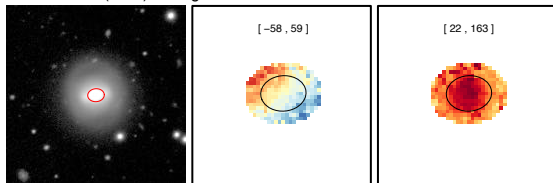

SAMI372452 (HSC): E/S0

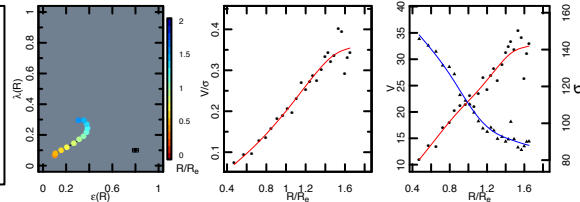

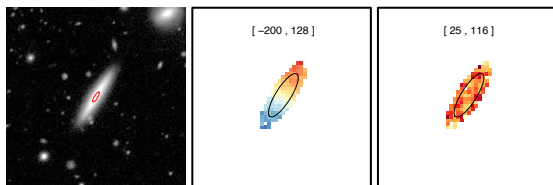

SAMI372568 (HSC): \*eSp

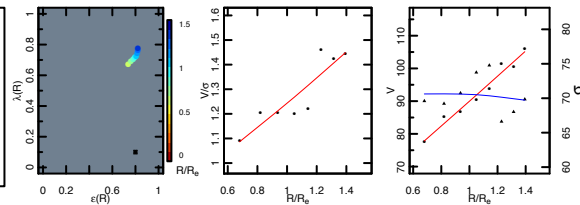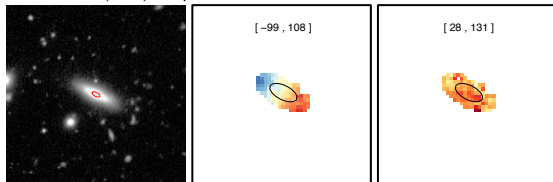

SAMI372599 (HSC): \*eSp

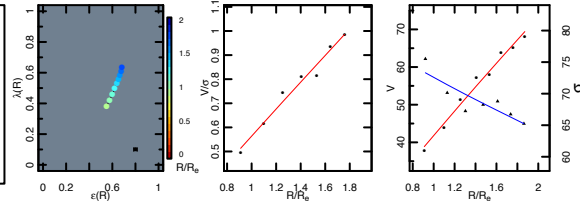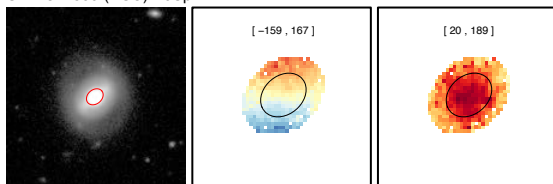

SAMI373105 (KiDS): \*eSp

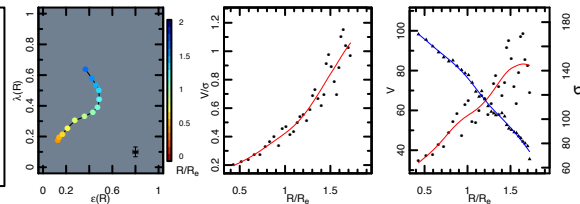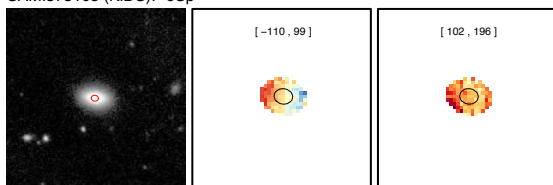

SAMI375564 (KiDS): S0

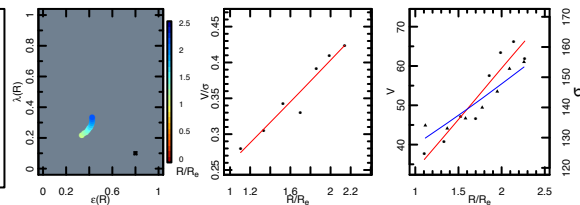

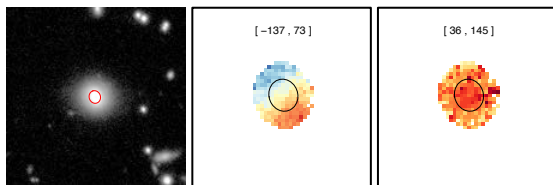

SAMI375615 (KiDS): \*E

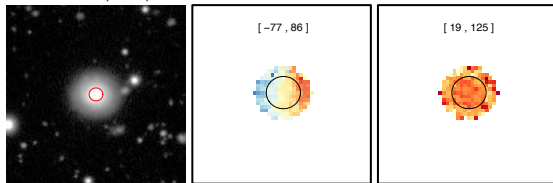

SAMI376001 (HSC): ?

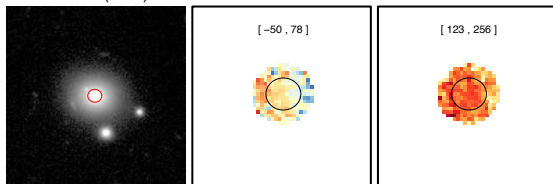

SAMI376703 (KiDS): E

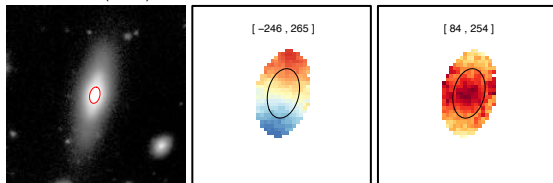

SAMI377666 (KiDS): \*eSp

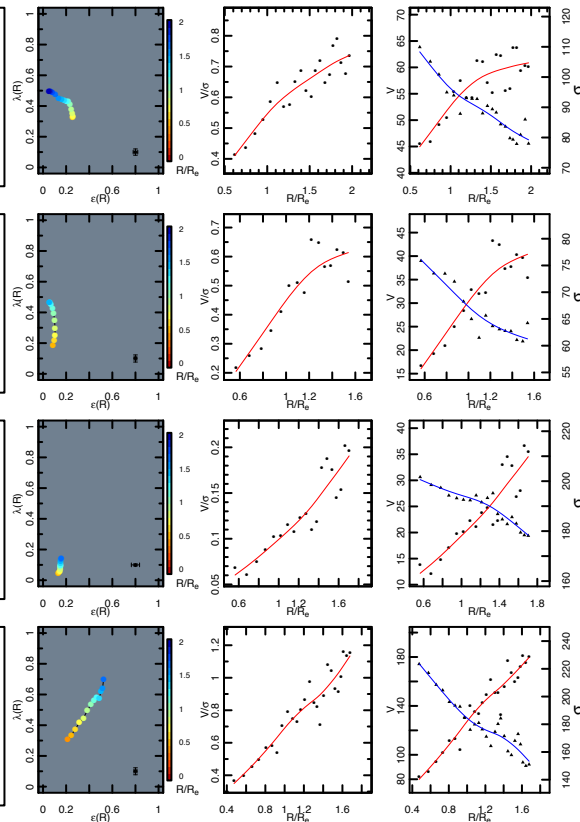

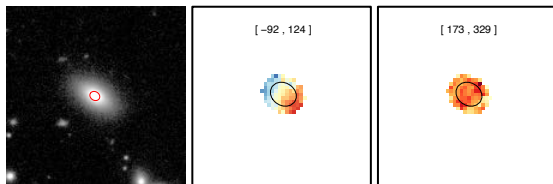

SAMI378104 (KiDS): S0

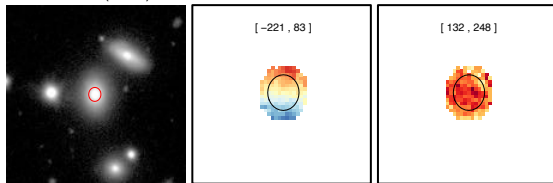

SAMI380697 (KiDS): S0

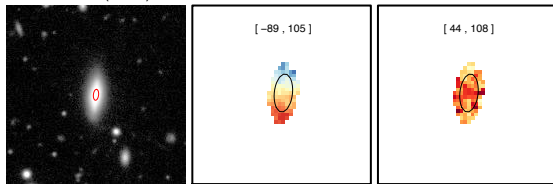

SAMI381156 (HSC): \*S0

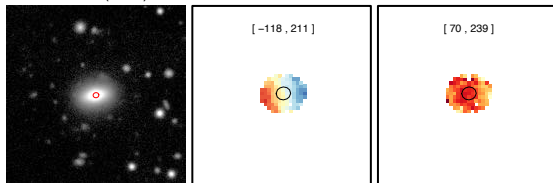

SAMI381157 (HSC): S0

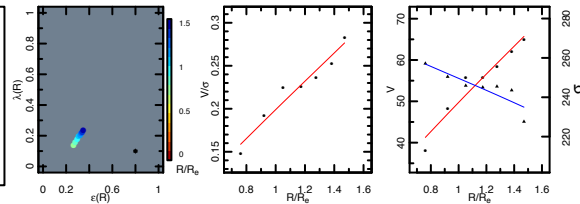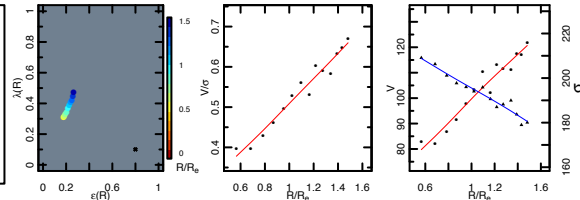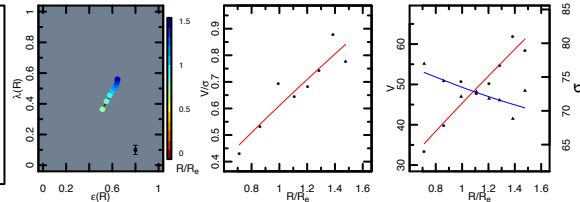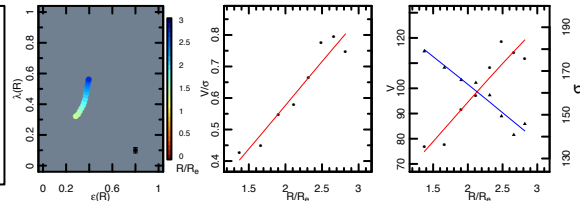

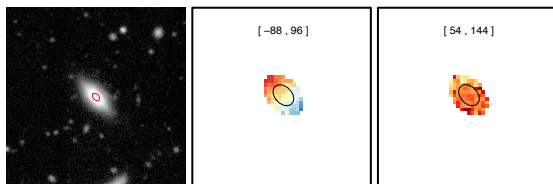

SAMI381160 (HSC): S0

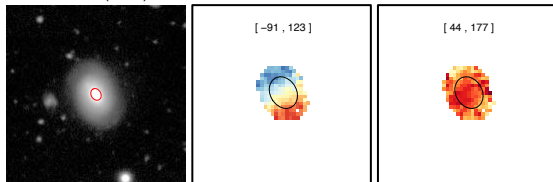

SAMI381219 (HSC): \*eSp

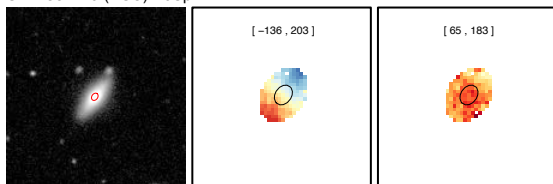

SAMI382158 (KiDS): S0

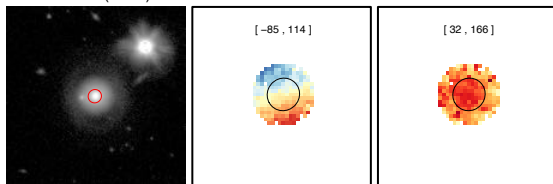

SAMI382505 (KiDS): E

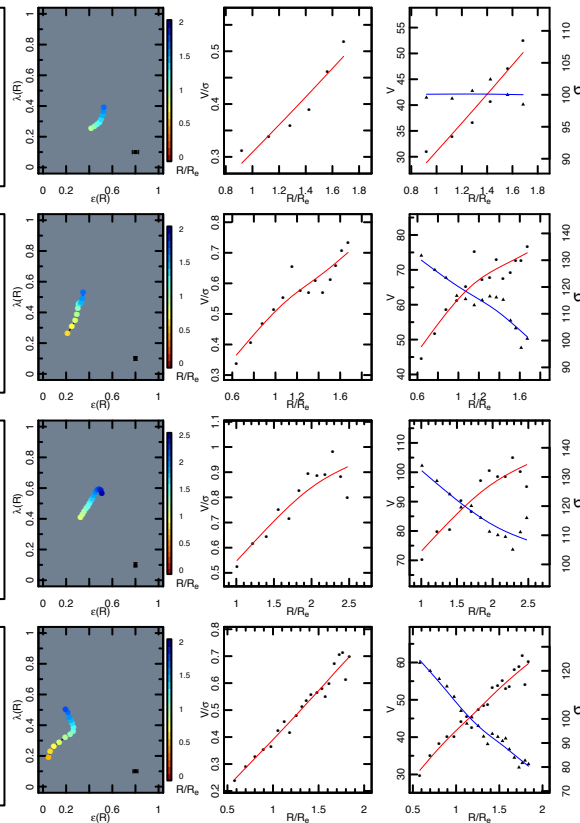



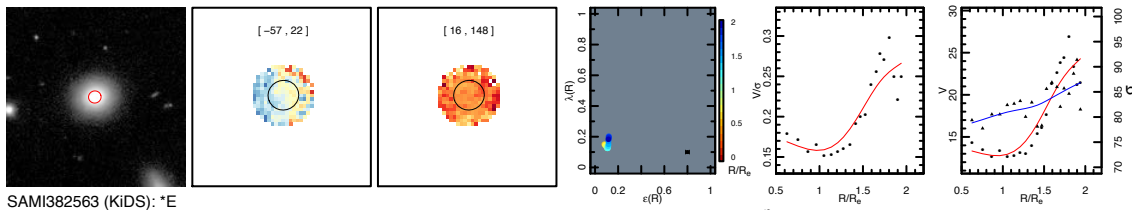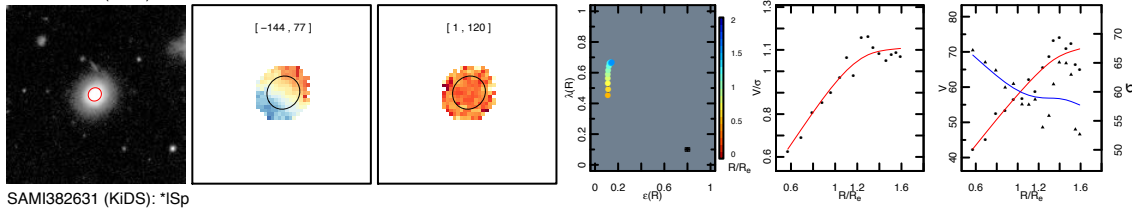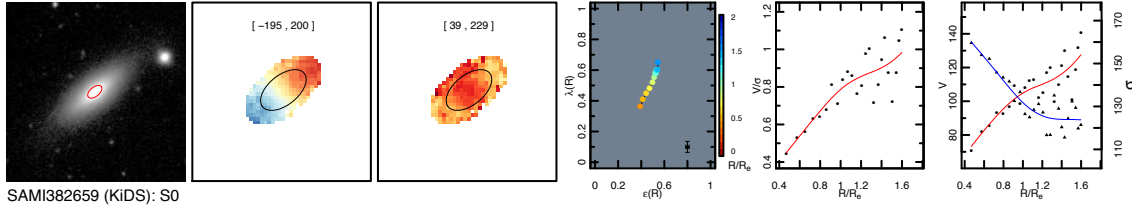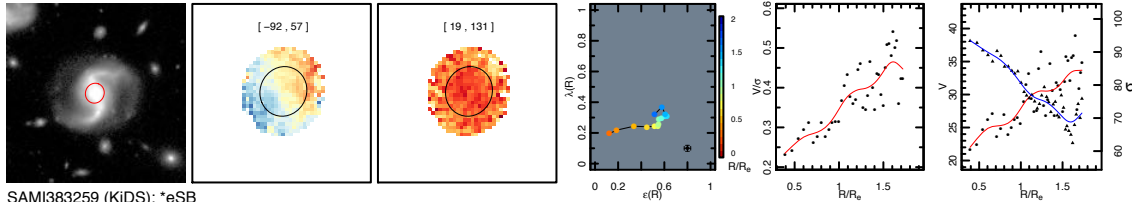

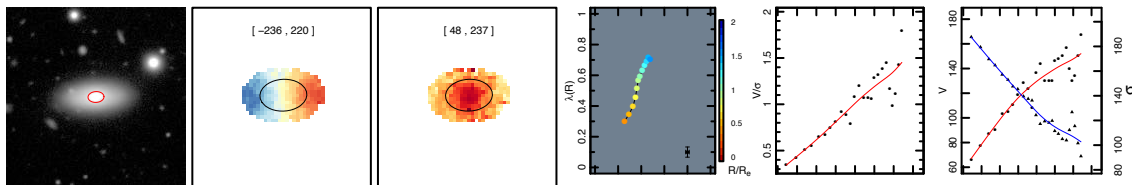

SAMI386268 (HSC): S0

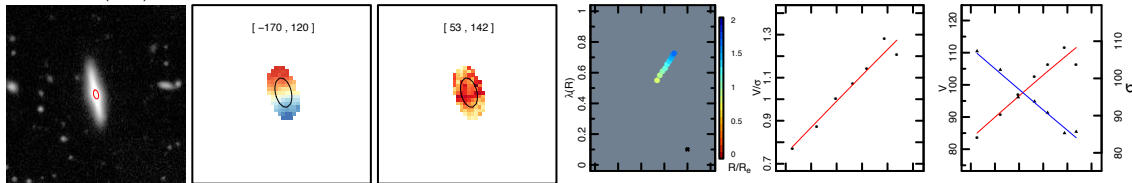

SAMI386316 (HSC): \*S0

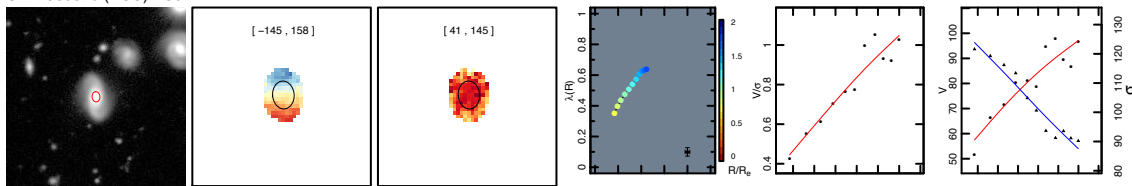

SAMI386366 (HSC): eSp

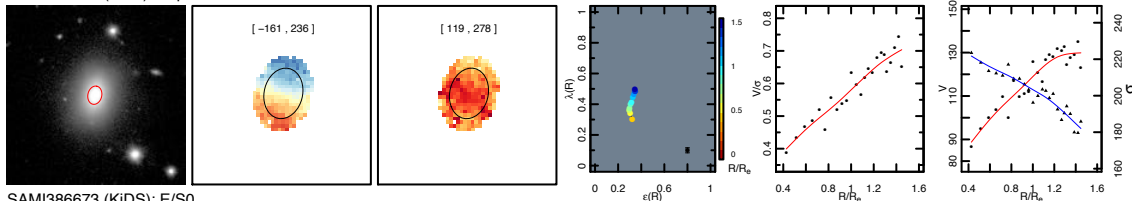

SAMI386673 (KiDS): E/S0

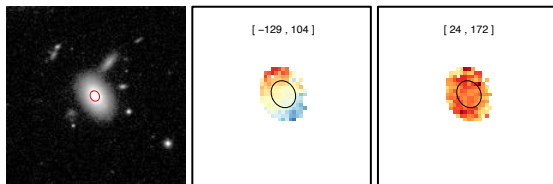

SAMI386722 (KiDS): \*S0

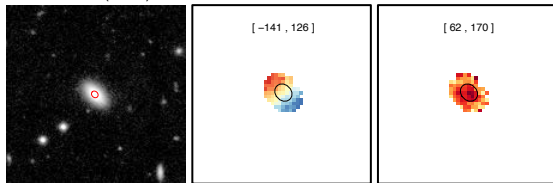

SAMI387042 (KiDS): S0

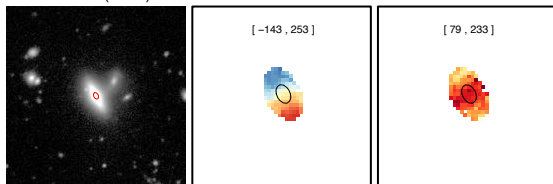

SAMI387080 (HSC): S0/eSp

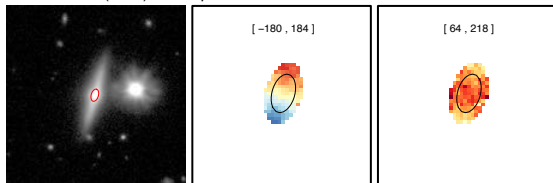

SAMI387675 (KiDS): \*S0

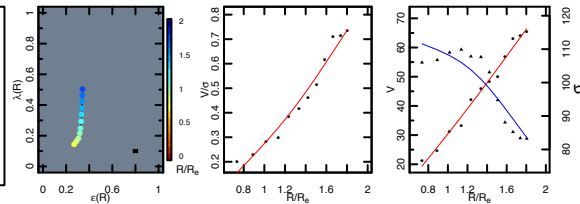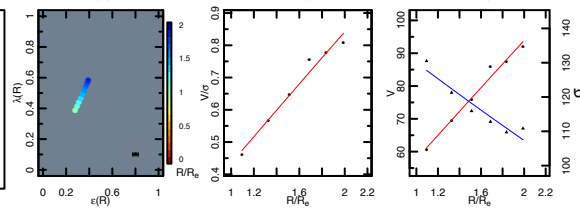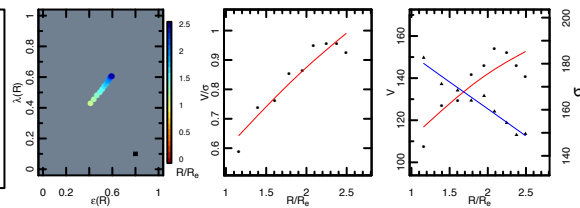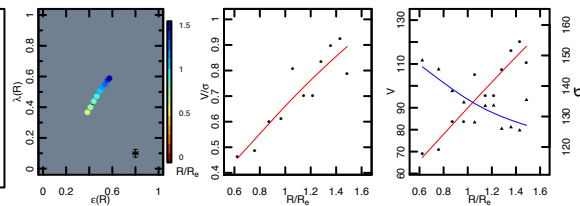

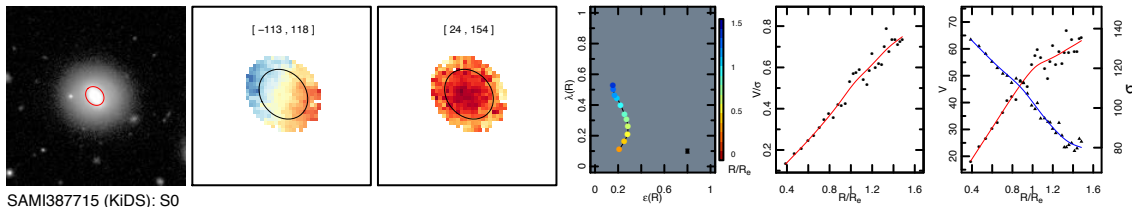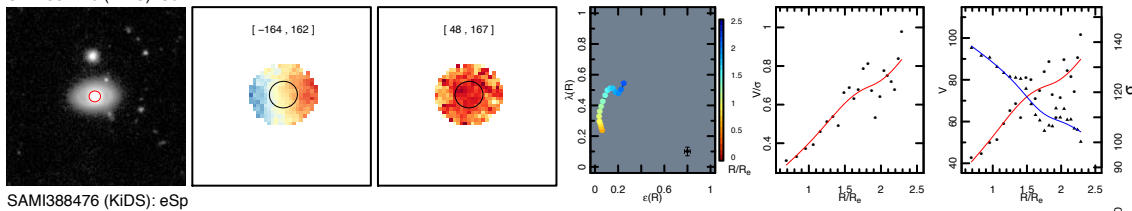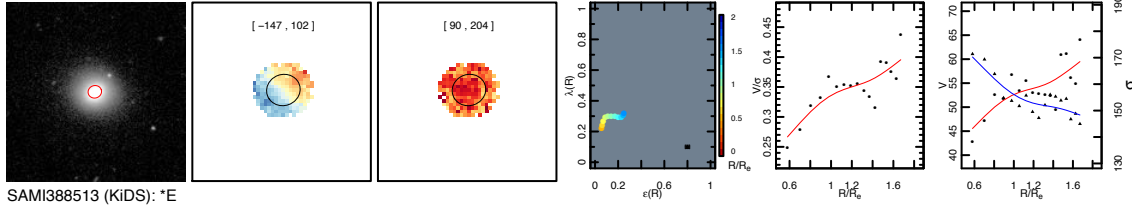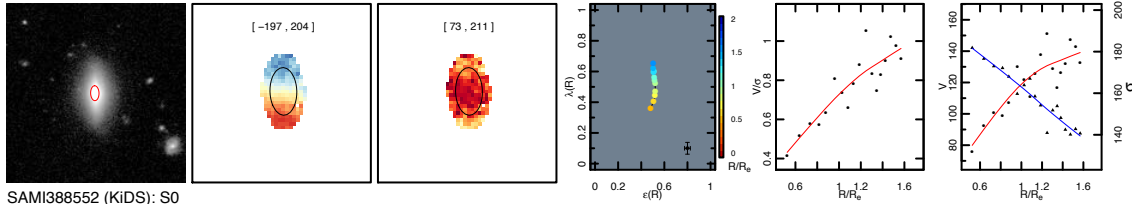

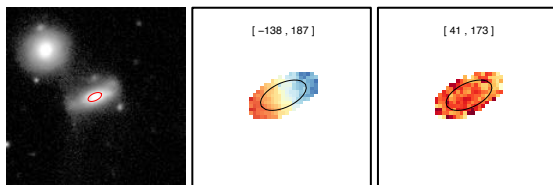

SAMI396584 (KiDS): eSp

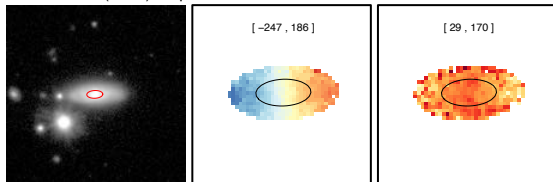

SAMI396607 (KiDS): eSp

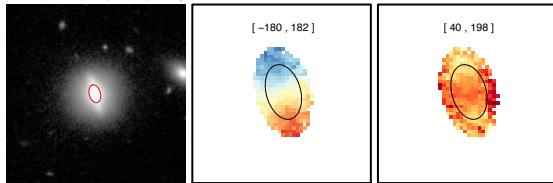

SAMI396615 (KiDS): \*eSp

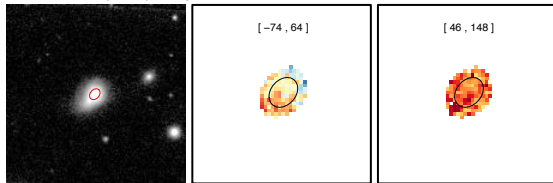

SAMI396709 (KiDS): eSp/ISp

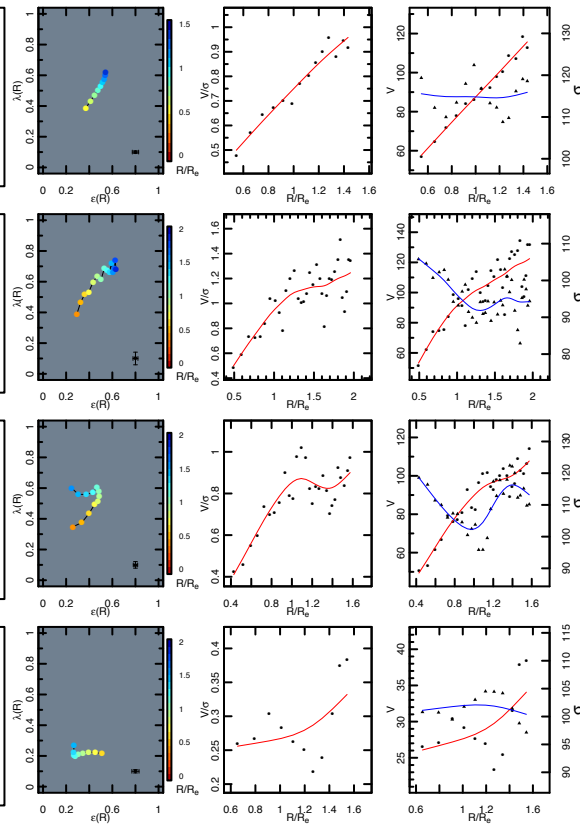

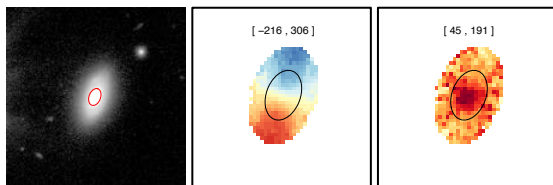

SAMI396781 (KiDS): \*eSp

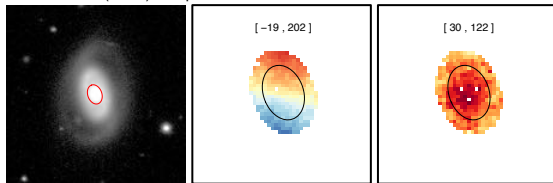

SAMI396833 (KiDS): eSp

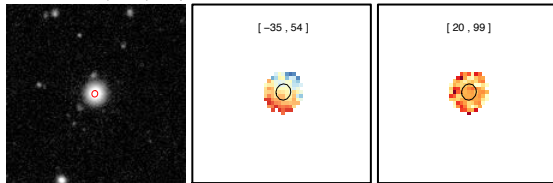

SAMI402988 (KiDS): \*E/S0

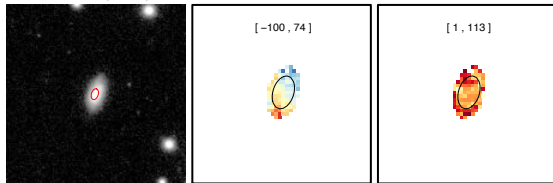

SAMI417392 (KiDS): ISp

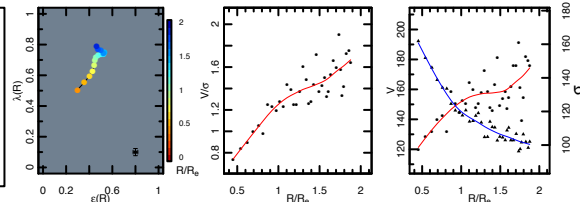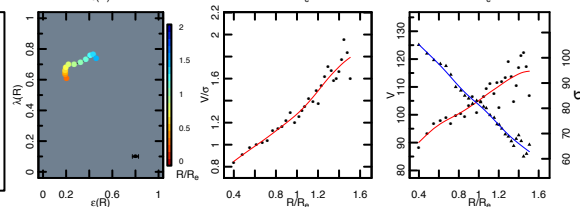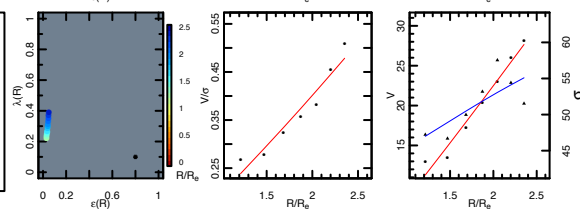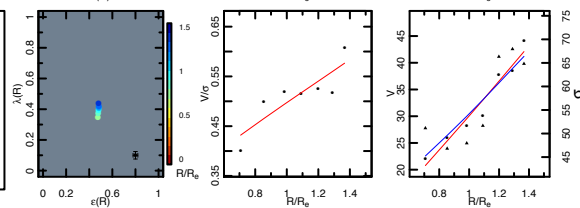

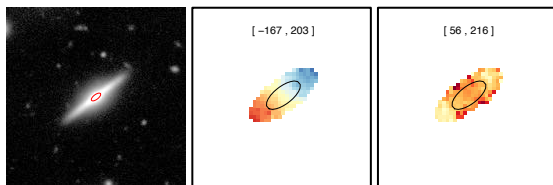

SAMI417433 (HSC): eSp

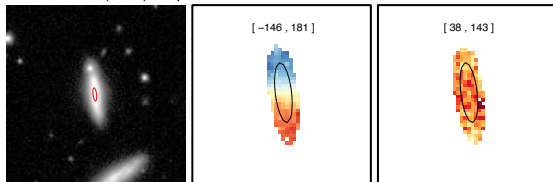

SAMI417678 (KiDS): \*ISp

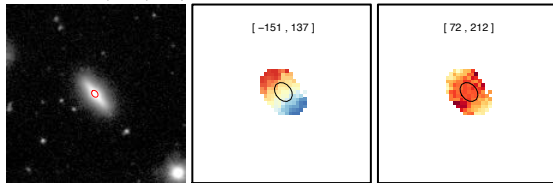

SAMI418630 (KiDS): S0

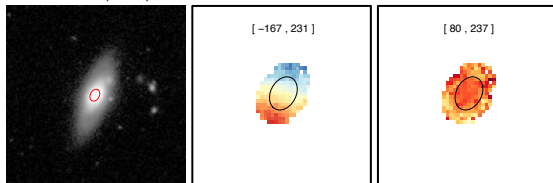

SAMI418693 (KiDS): \*eSp

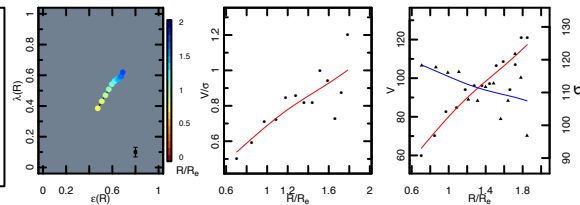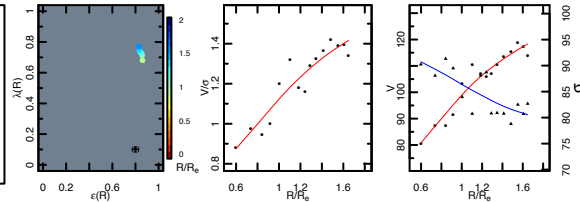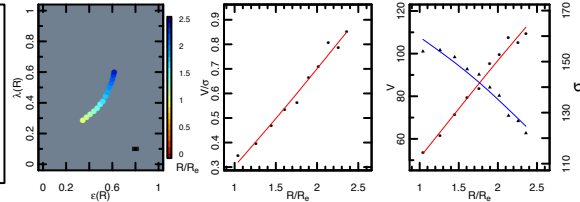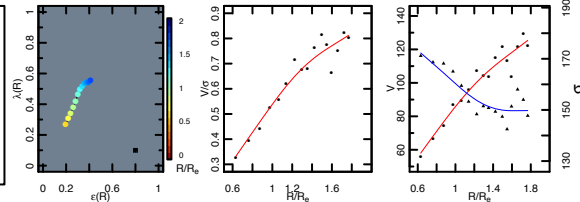

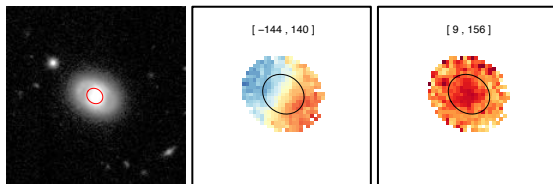

SAMI418725 (KiDS): eSp

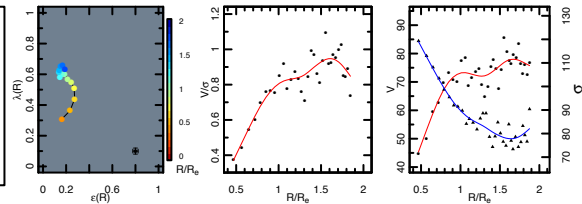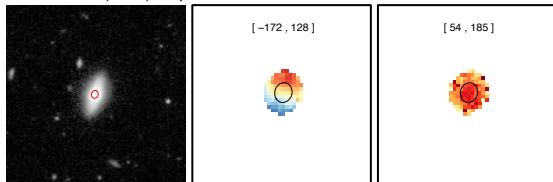

SAMI419294 (KiDS): S0

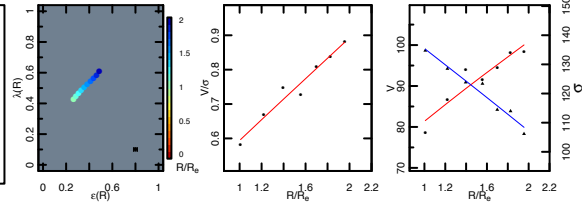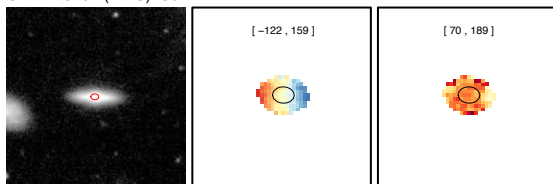

SAMI419335 (KiDS): S0

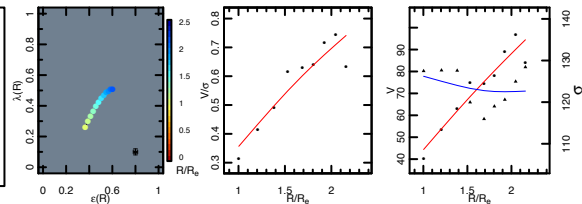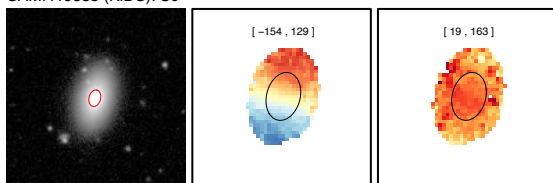

SAMI419345 (KiDS): S0

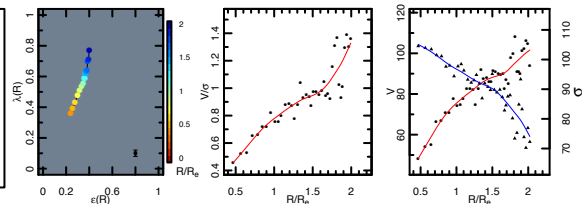



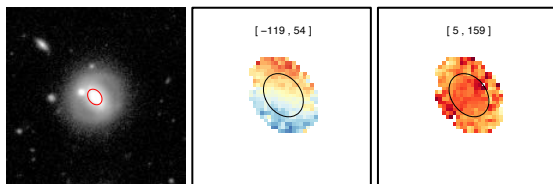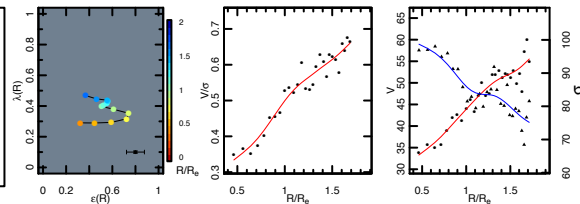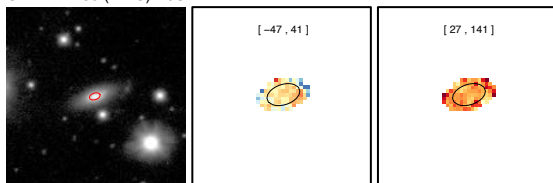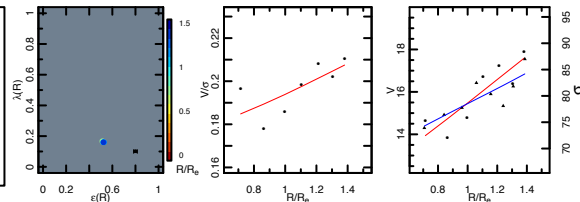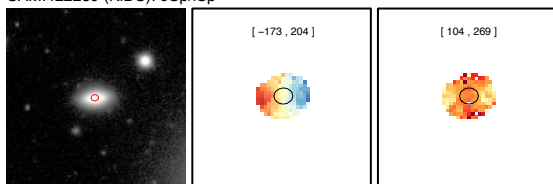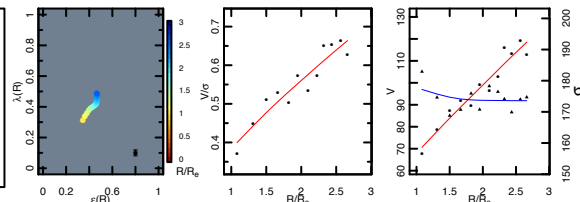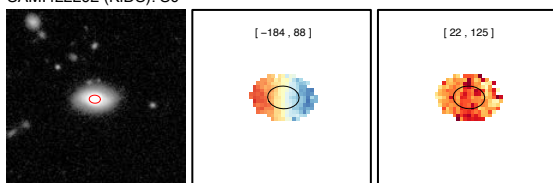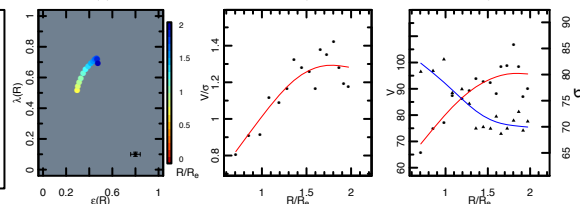

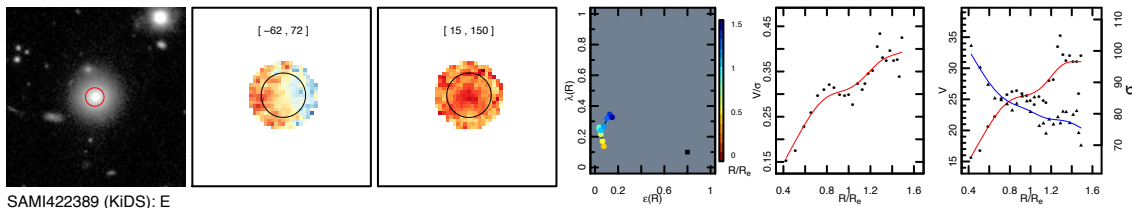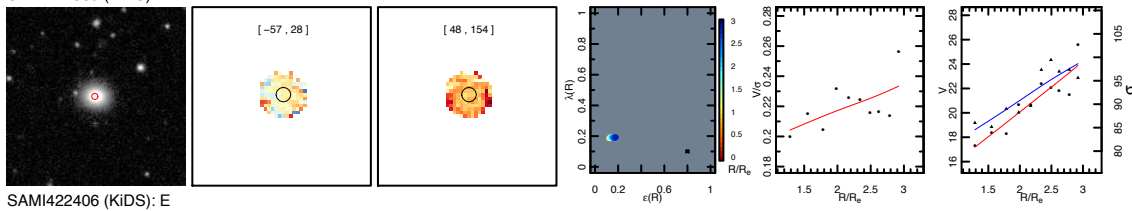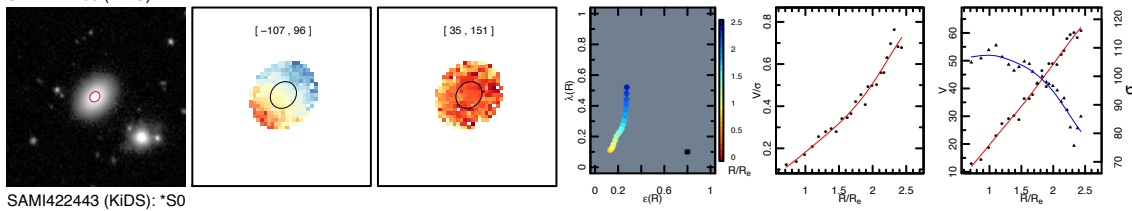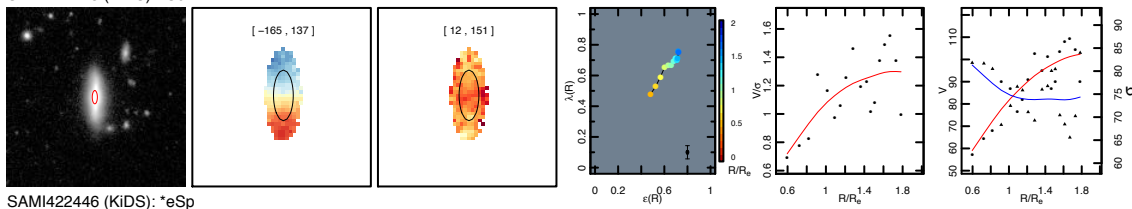

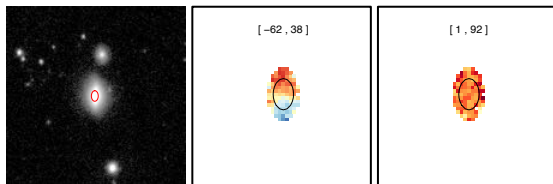

SAMI422610 (KiDS): ISp

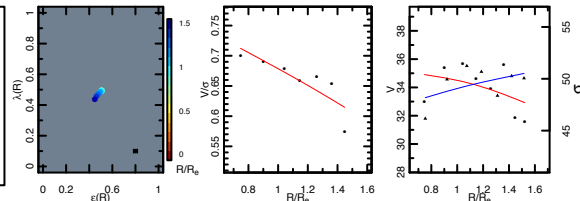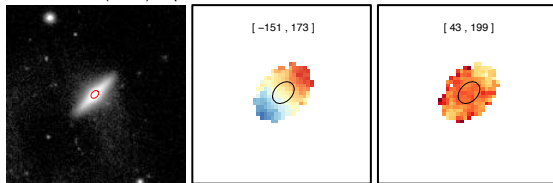

SAMI457615 (KiDS): \*S0

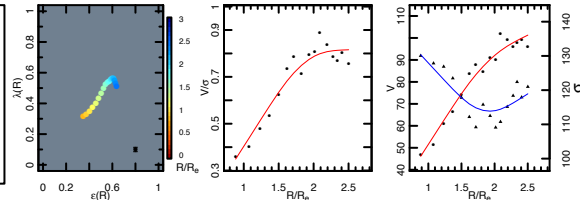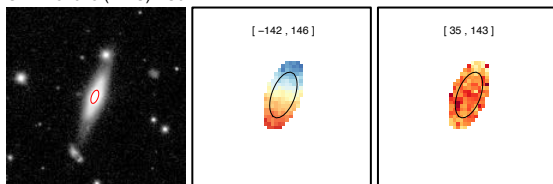

SAMI460380 (KiDS): eSp

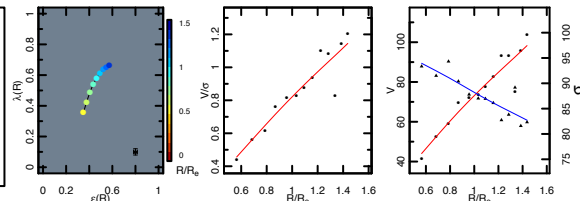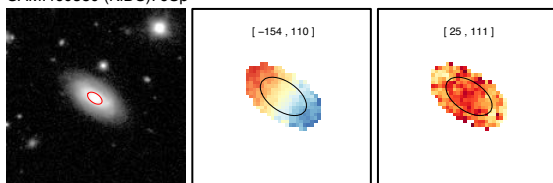

SAMI460756 (KiDS): eSp

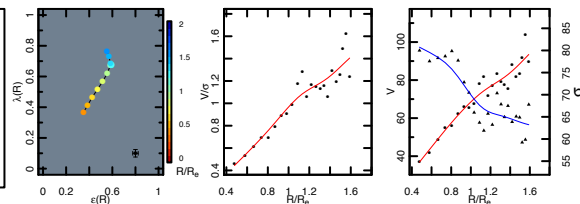

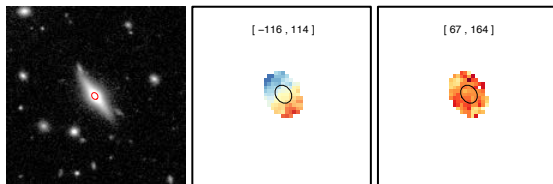

SAMI460767 (KiDS): \*S0

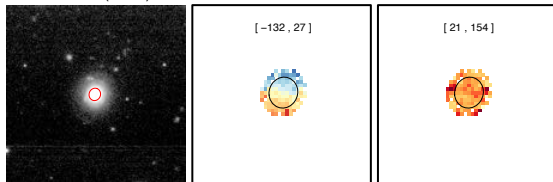

SAMI463148 (KiDS): \*E

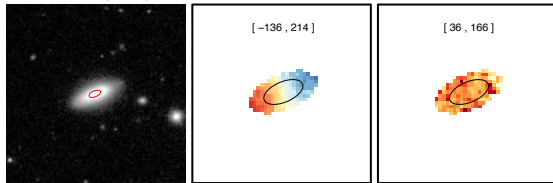

SAMI463434 (KiDS): \*eSp

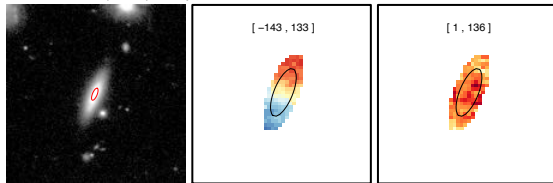

SAMI463641 (KiDS): ISp

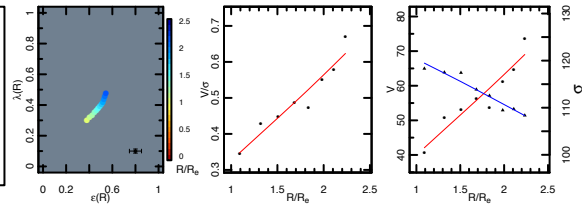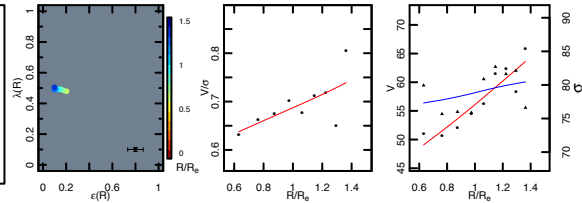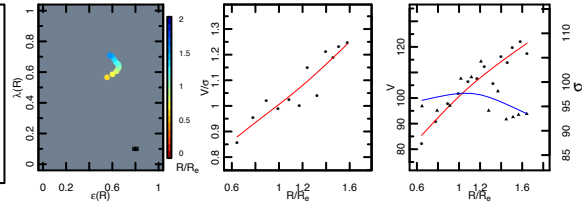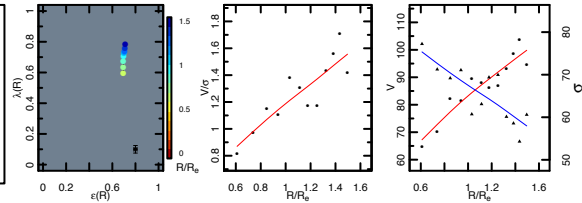

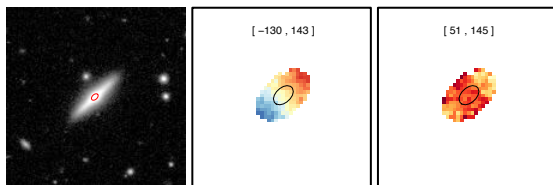

SAMI485047 (KiDS): \*S0

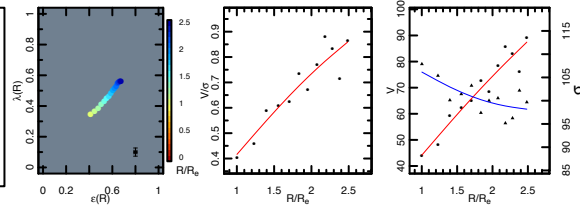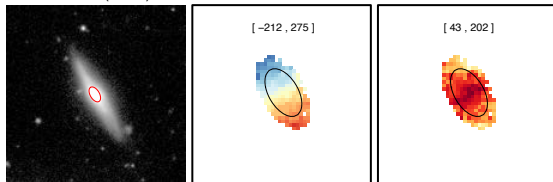

SAMI485127 (KiDS): eSp

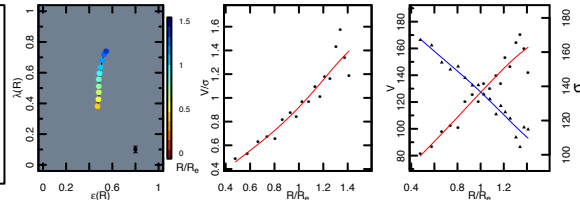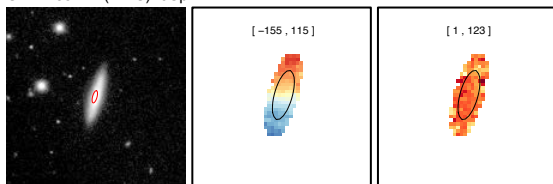

SAMI485688 (KiDS): \*eSp

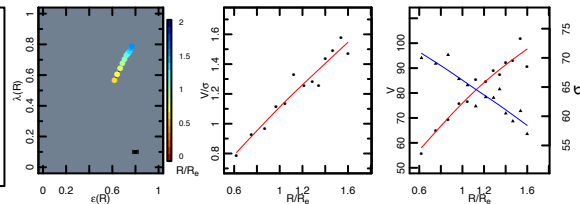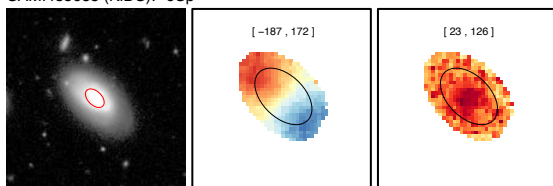

SAMI485834 (KiDS): eSp/ISp

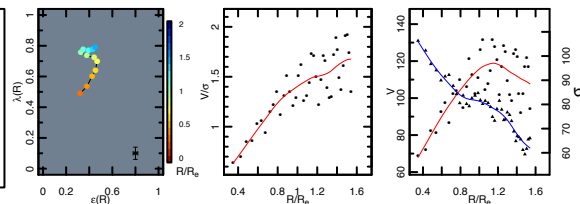

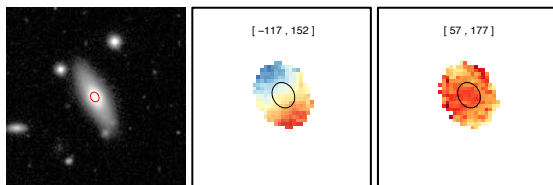

SAMI485882 (KiDS): eSp

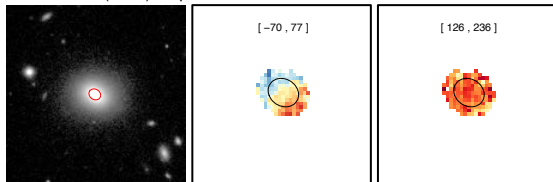

SAMI485883 (KiDS): \*E

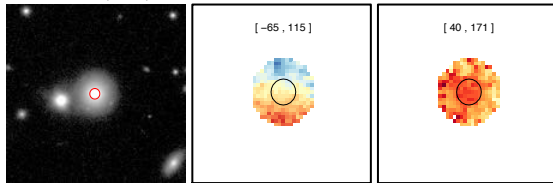

SAMI485921 (KiDS): E

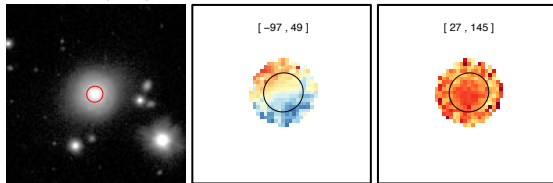

SAMI485924 (KiDS): eSp

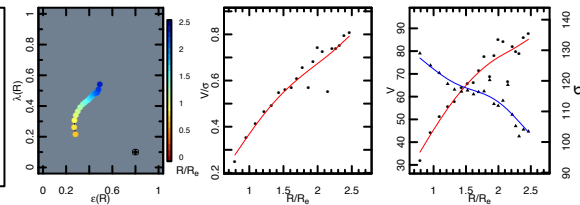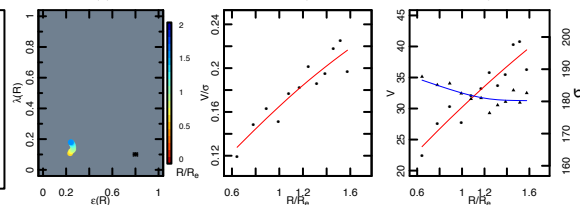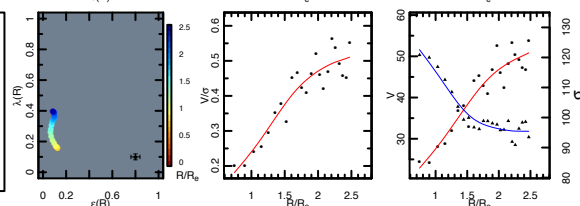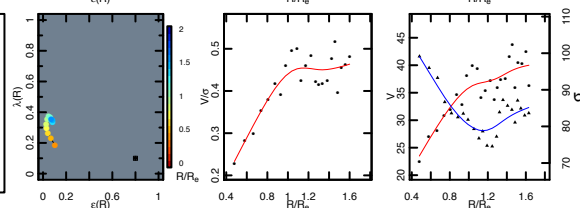

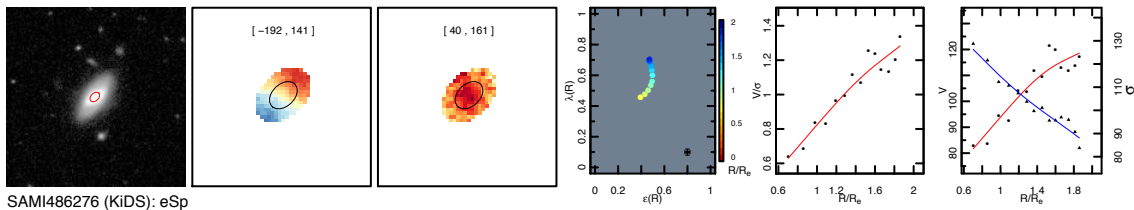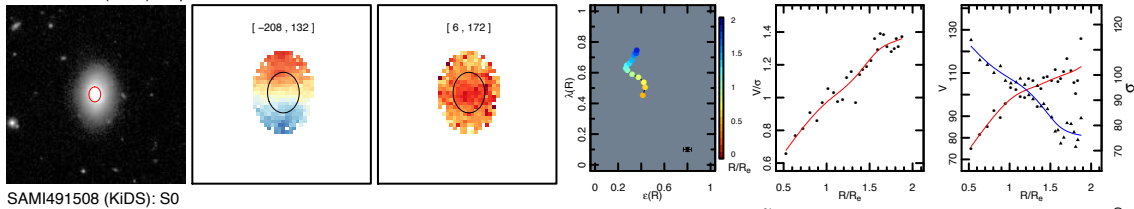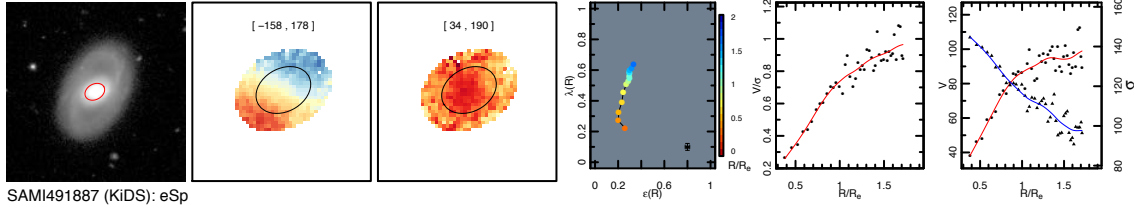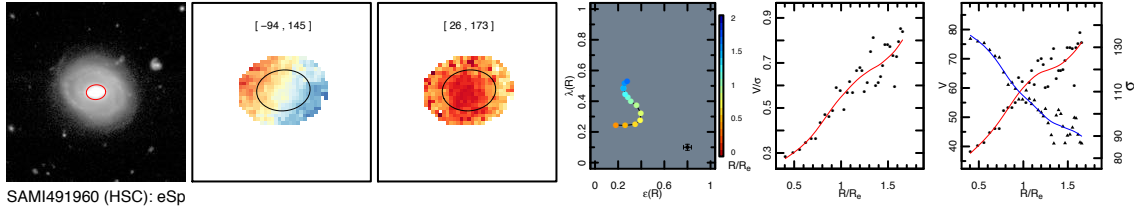

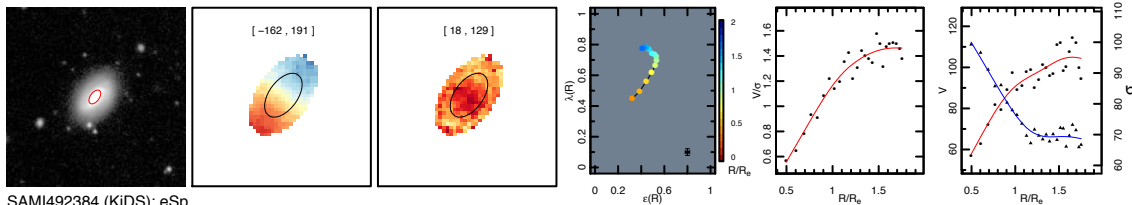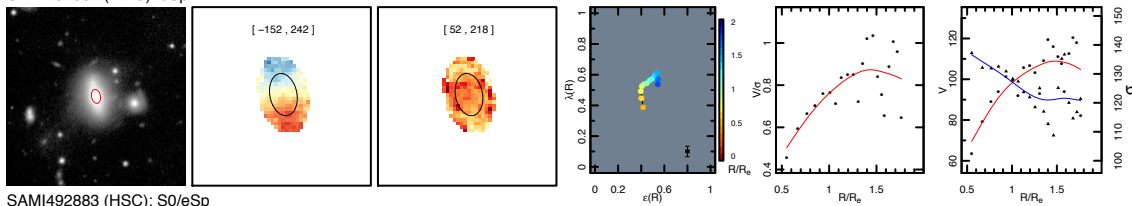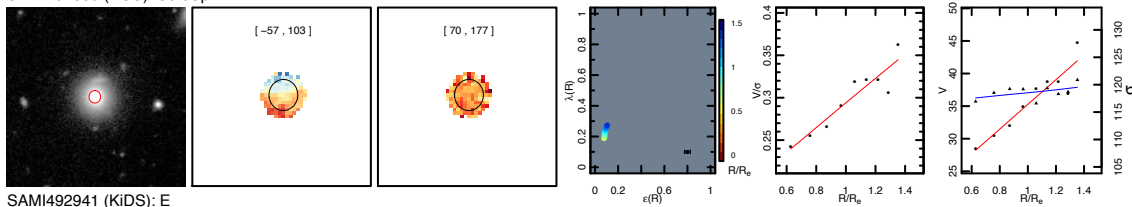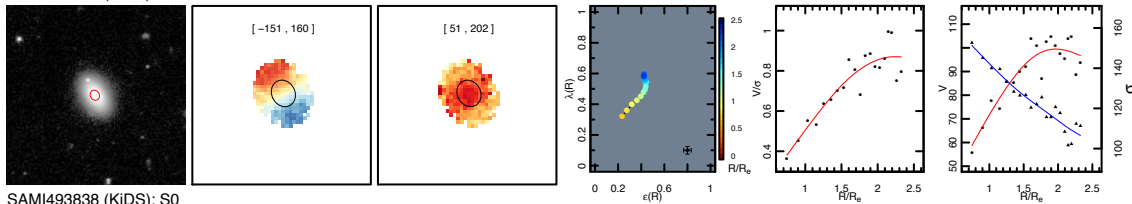



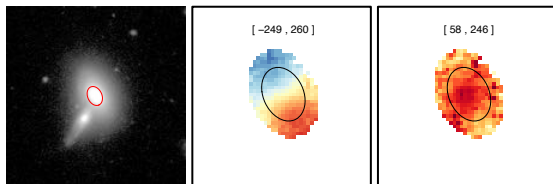

SAMI497035 (KiDS): \*S0

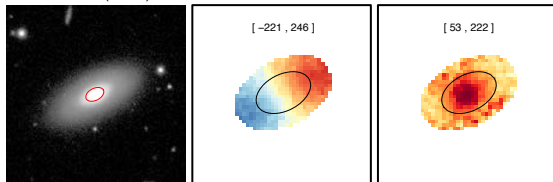

SAMI504730 (KiDS): S0

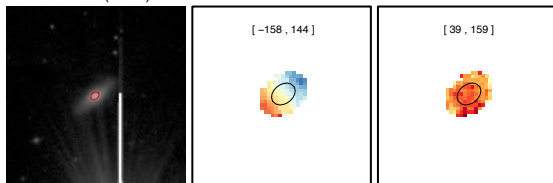

SAMI504877 (KiDS): S0

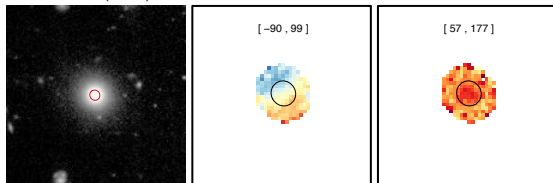

SAMI504879 (KiDS): \*E

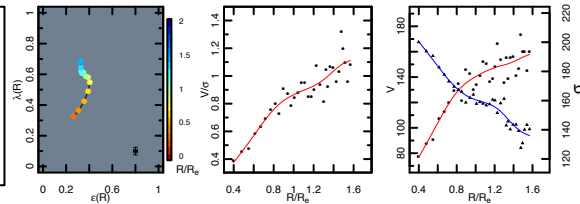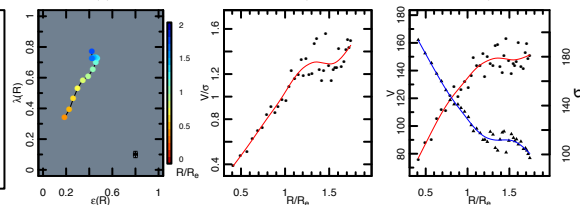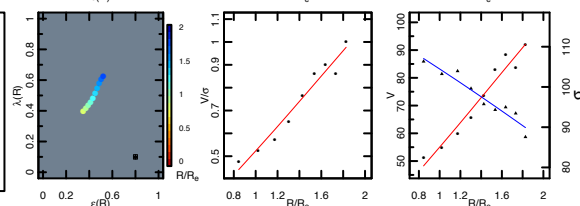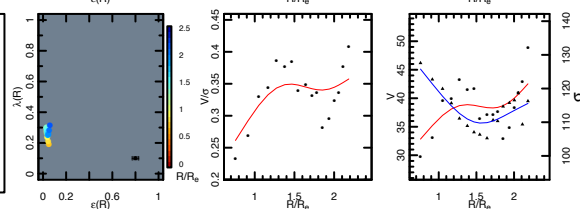

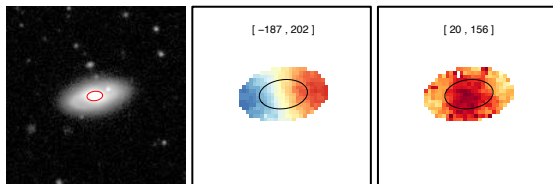

SAMI505316 (KiDS): eSp

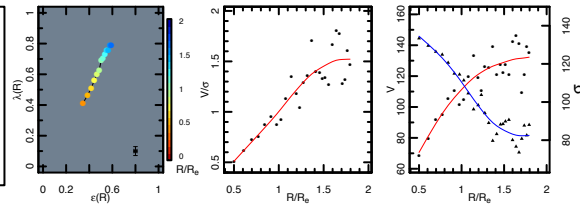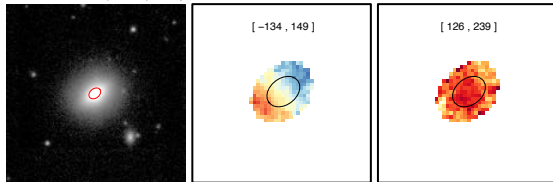

SAMI505341 (KiDS): \*Embedded Disc?

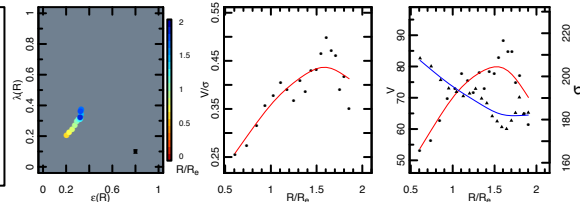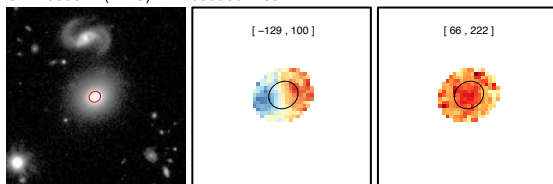

SAMI505765 (KiDS): E

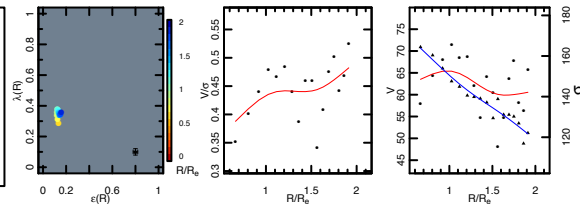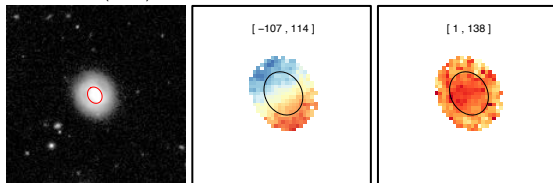

SAMI505828 (KiDS): eSp

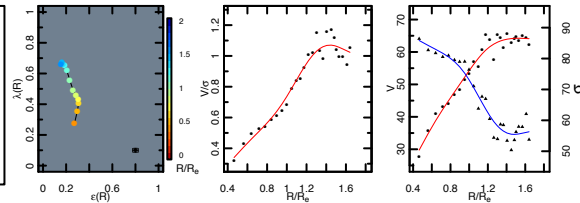

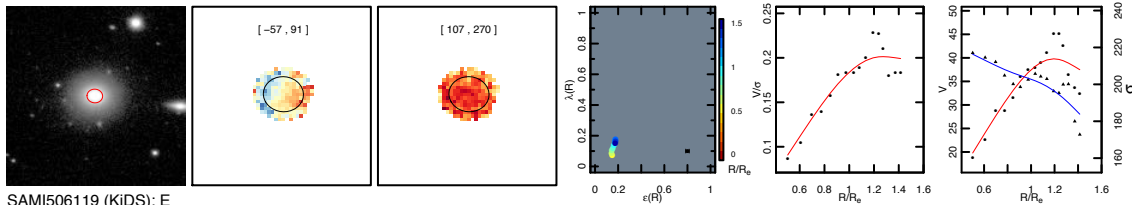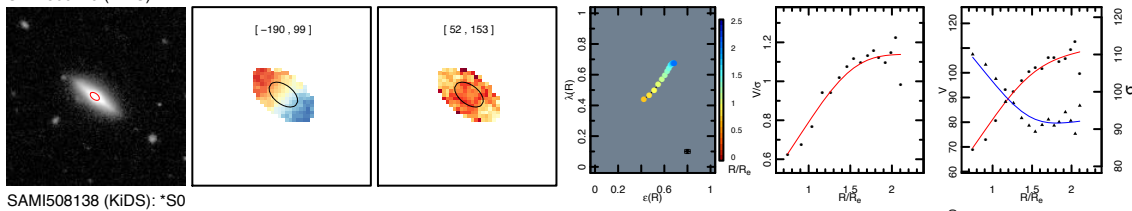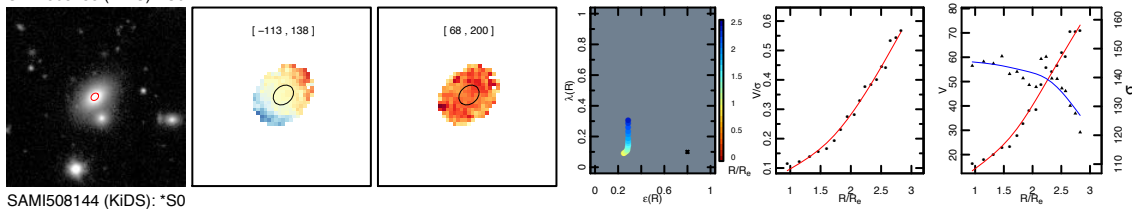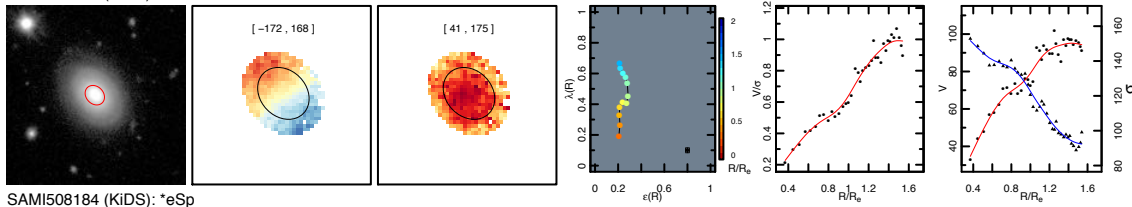

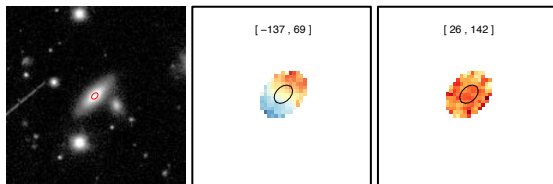

SAMI508312 (KiDS): \*S0

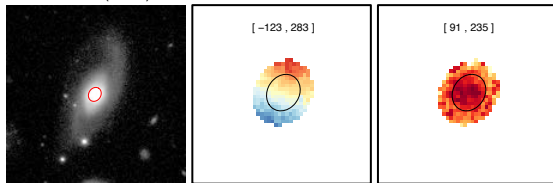

SAMI508315 (KiDS): S0/eSp

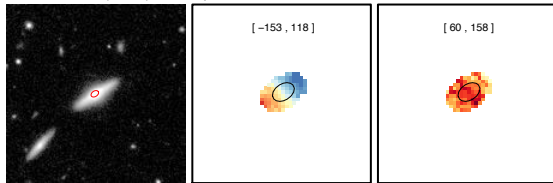

SAMI508568 (KiDS): \*eSp

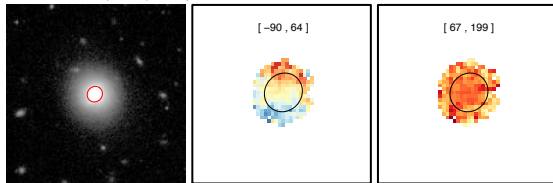

SAMI508593 (KiDS): \*E

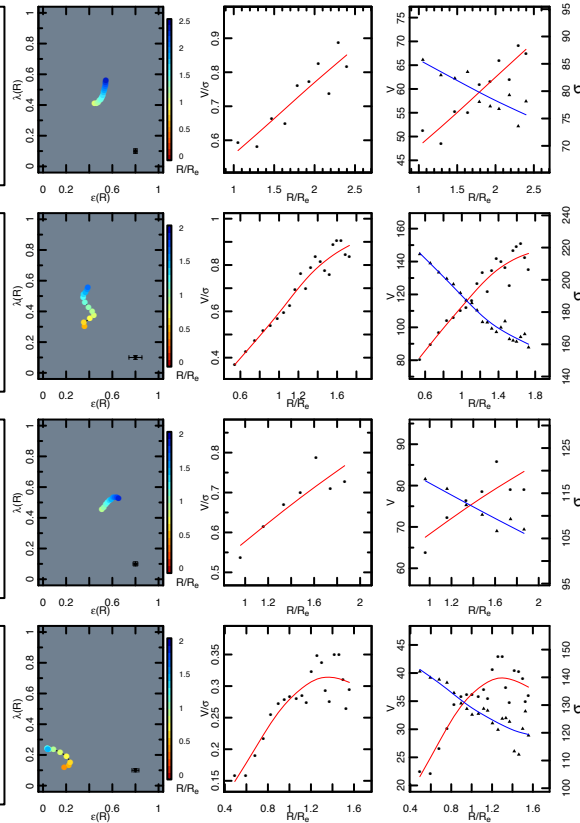

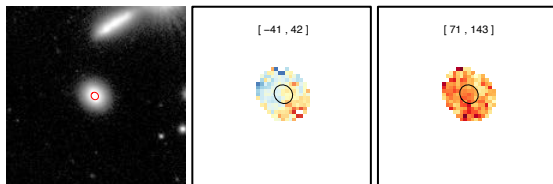

SAMI508751 (KiDS): \*E

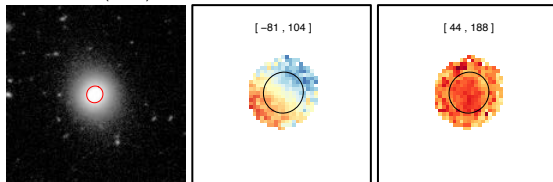

SAMI509075 (KiDS): E

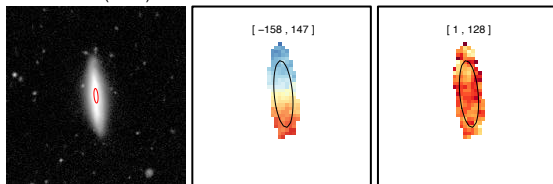

SAMI511456 (HSC): \*eSp

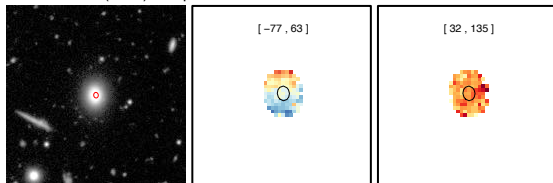

SAMI511864 (HSC): \*E/S0

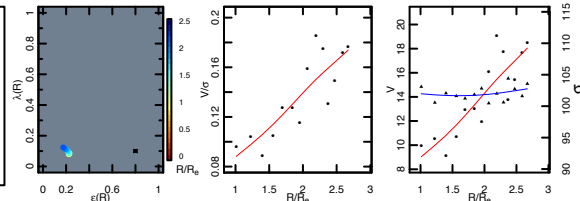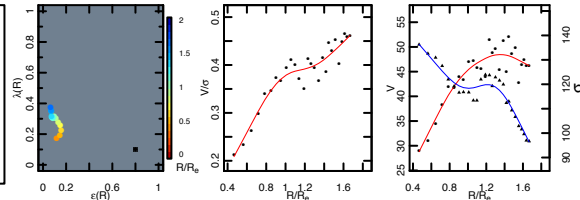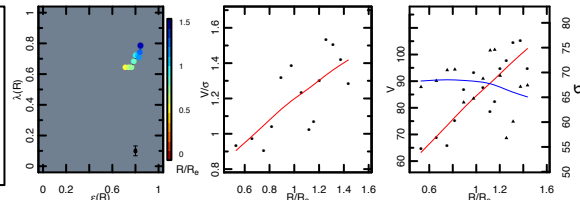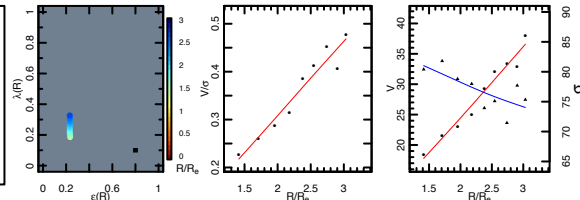

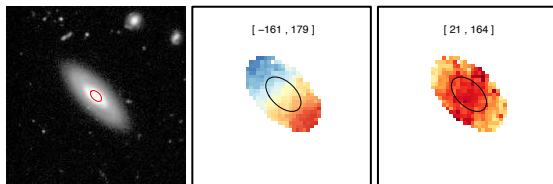

SAMI511890 (HSC): \*eSp

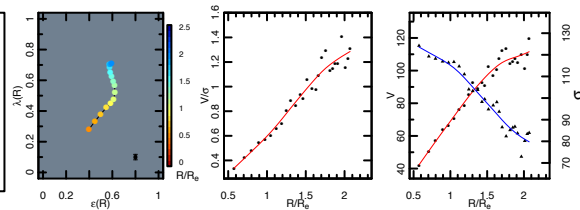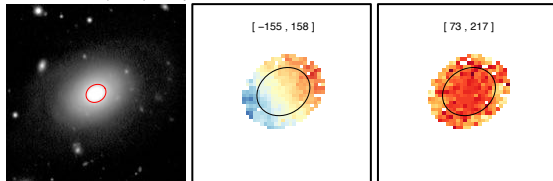

SAMI511892 (HSC): S0

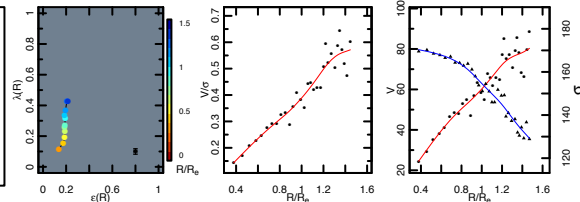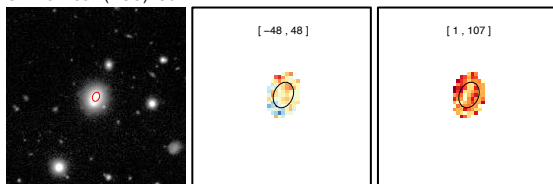

SAMI511921 (HSC): lSp

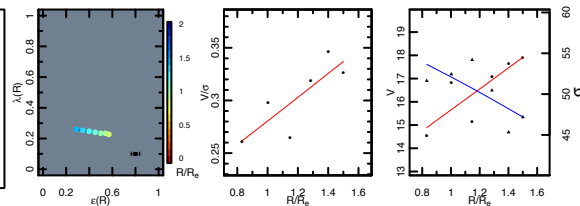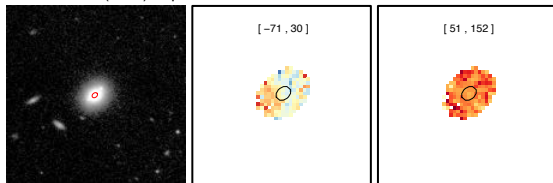

SAMI514022 (KiDS): S0/eSp

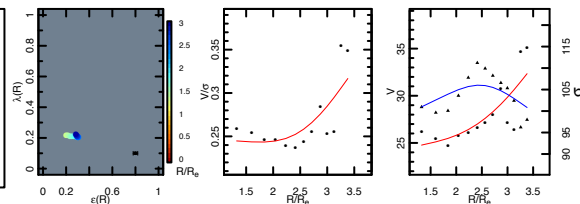

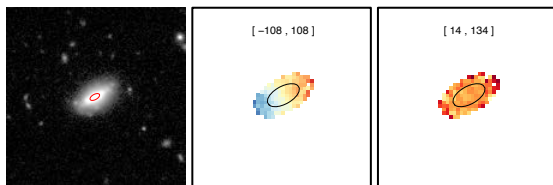

SAMI514212 (KiDS): ISp

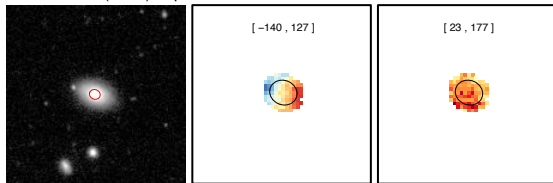

SAMI517244 (KiDS): \*S0

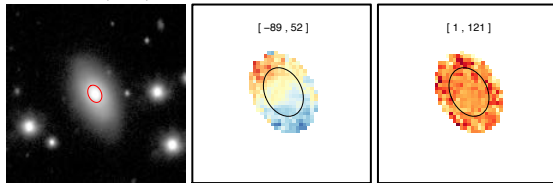

SAMI517273 (KiDS): ISp

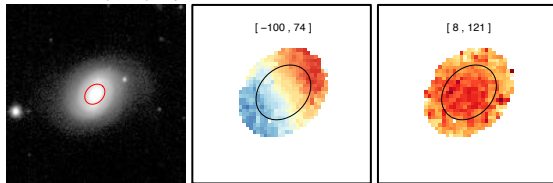

SAMI517302 (KiDS): \*eSB

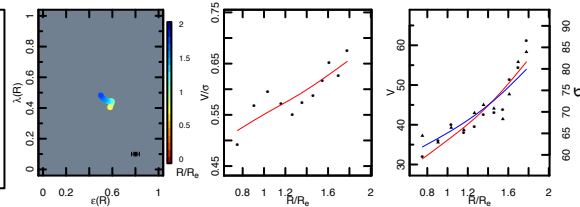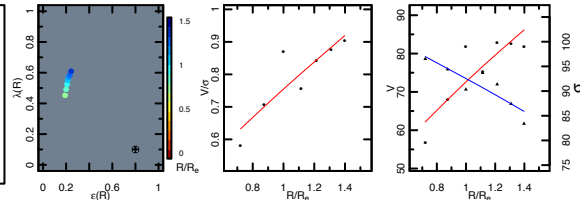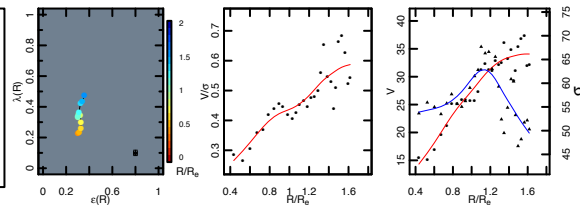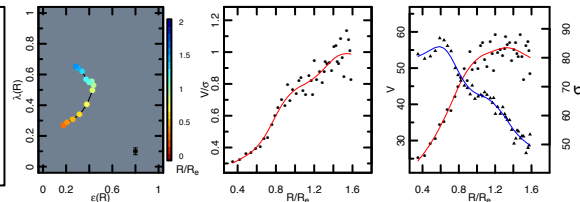

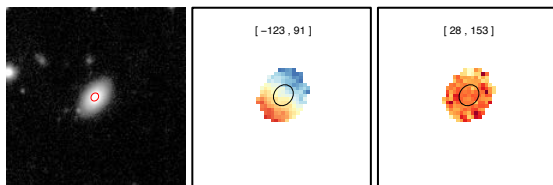

SAMI518829 (KiDS): \*S0

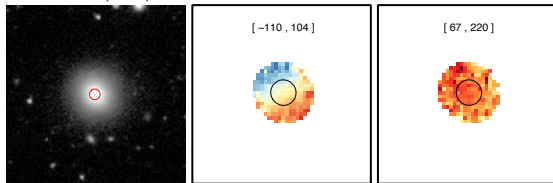

SAMI519141 (KiDS): \*S0

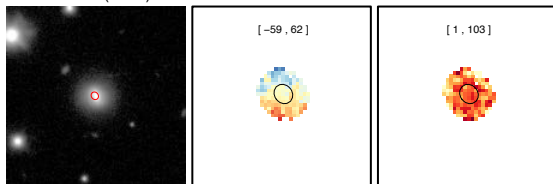

SAMI521736 (KiDS): \*ISp

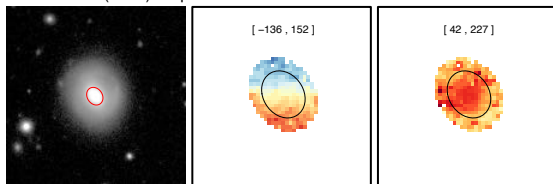

SAMI527984 (KiDS): eSp

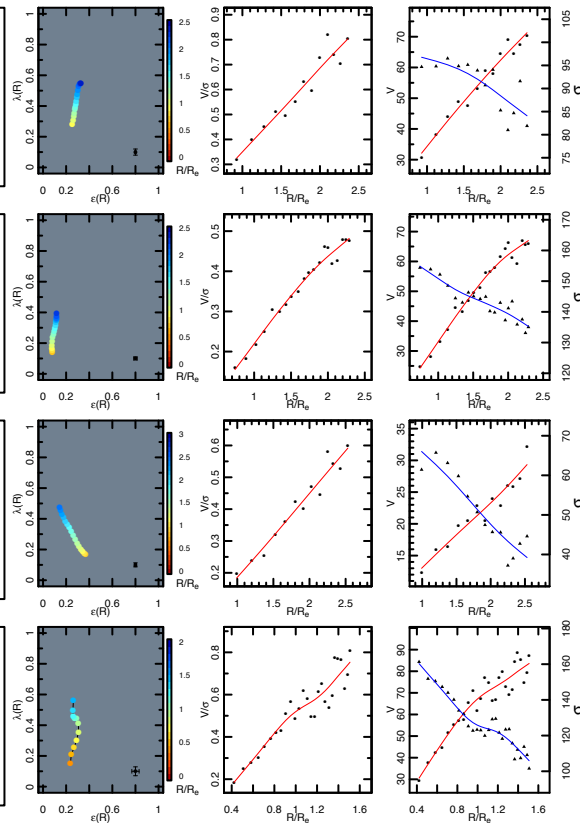



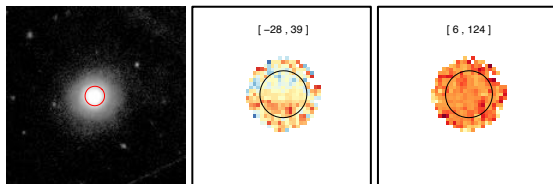

SAMI534654 (KiDS): \*E

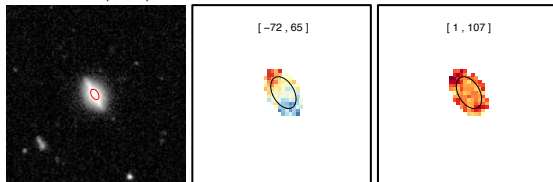

SAMI534710 (KiDS): eSp/Sp

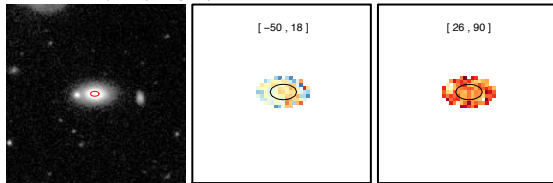

SAMI534763 (KiDS): S0

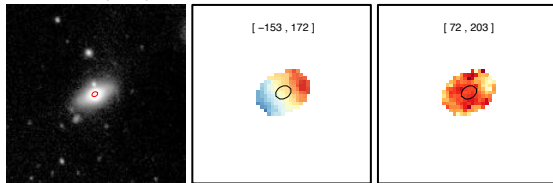

SAMI534904 (KiDS): S0

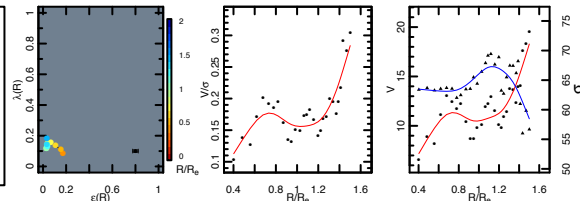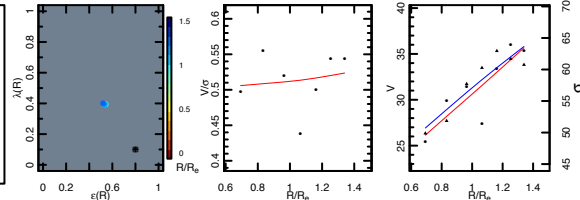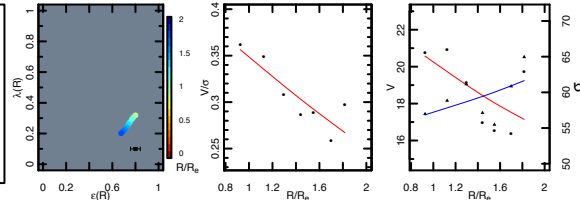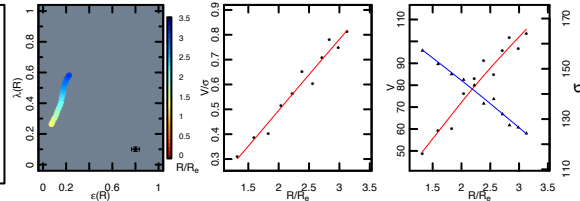

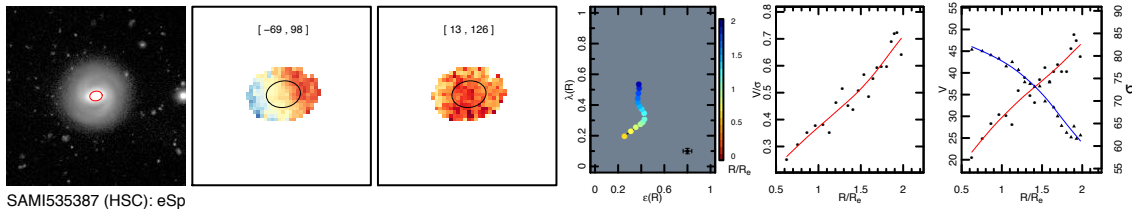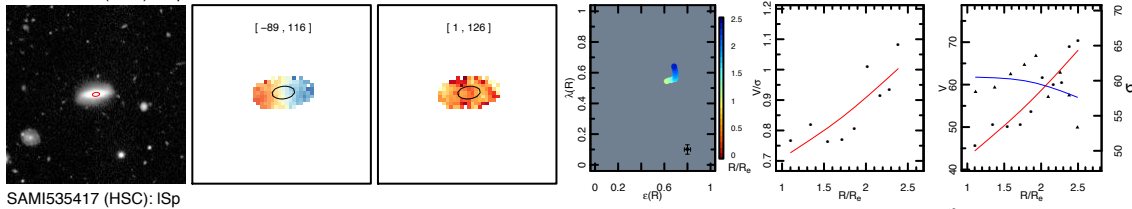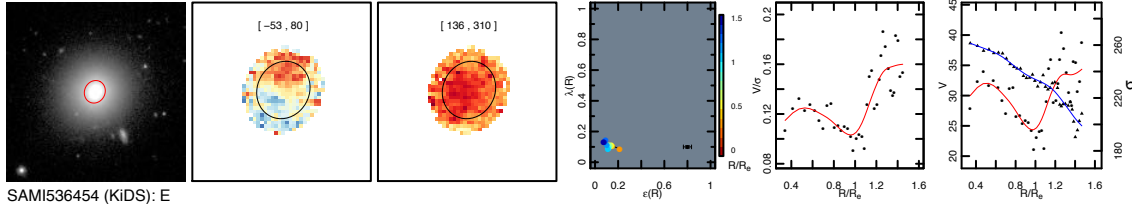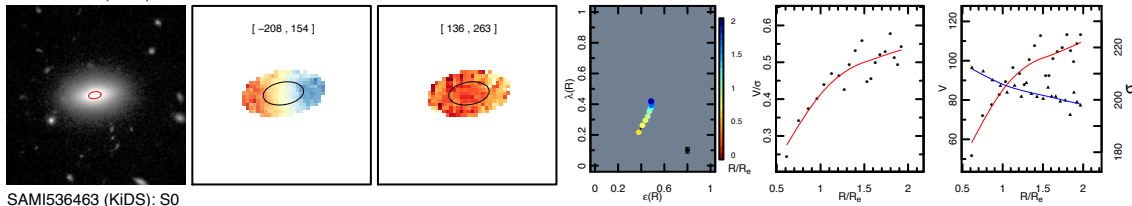

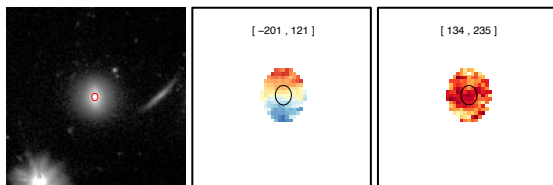

SAMI536963 (KiDS): \*S0

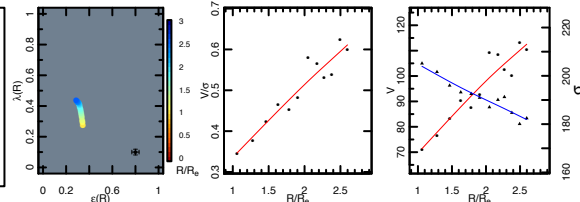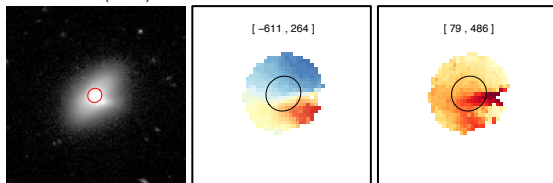

SAMI537467 (KiDS): \*Merger

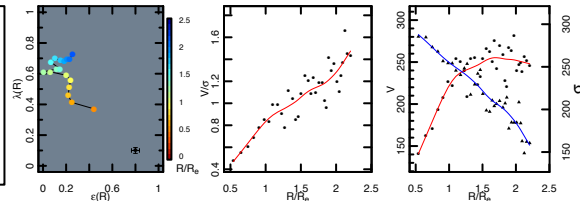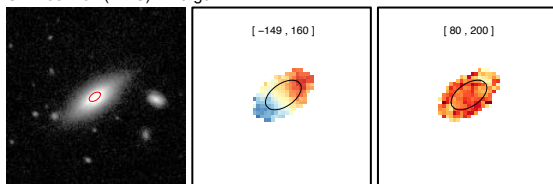

SAMI543501 (KiDS): S0

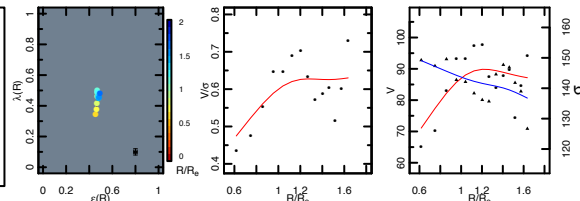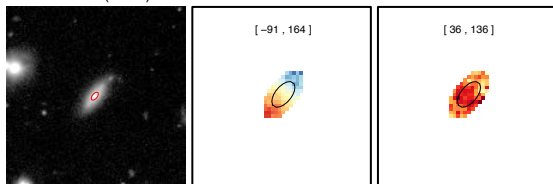

SAMI543552 (KiDS): \*S0

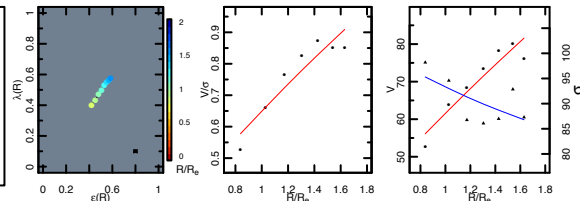

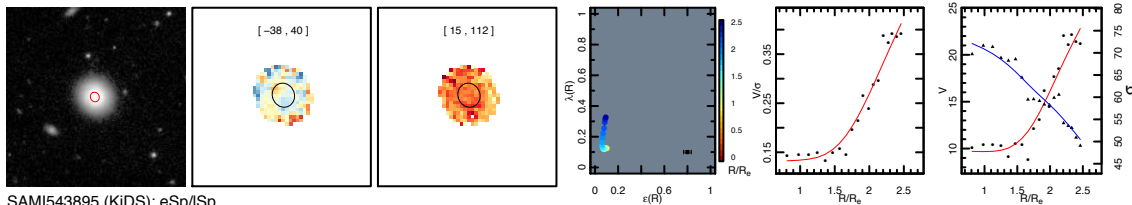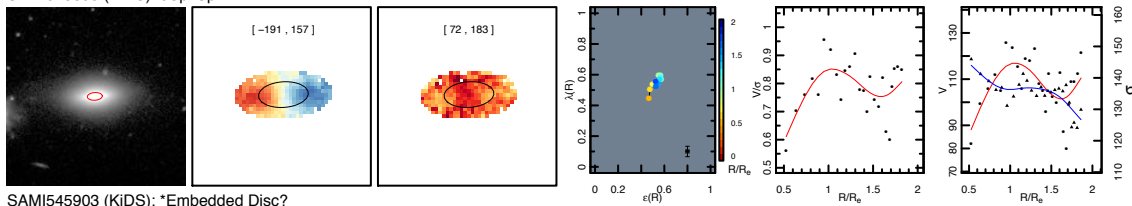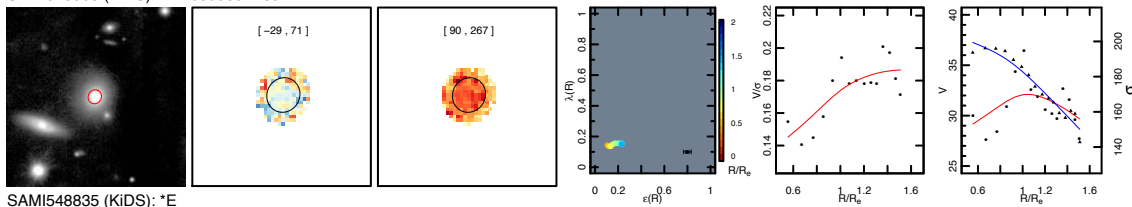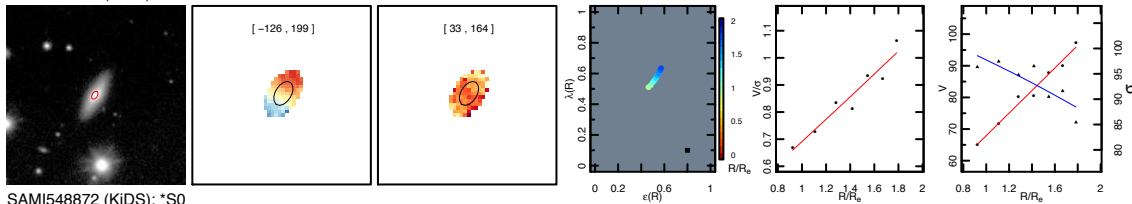

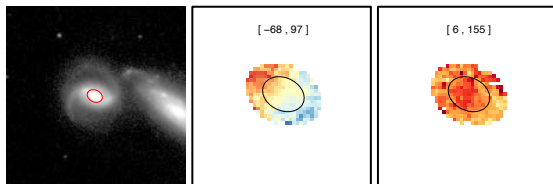

SAMI548946 (KiDS): \*eSB

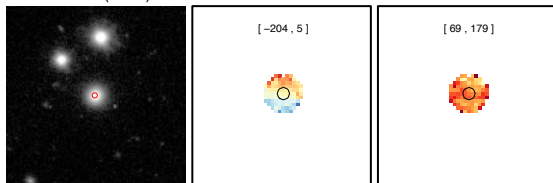

SAMI549070 (KiDS): \*E

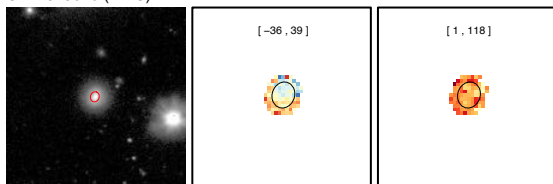

SAMI549313 (KiDS): ?

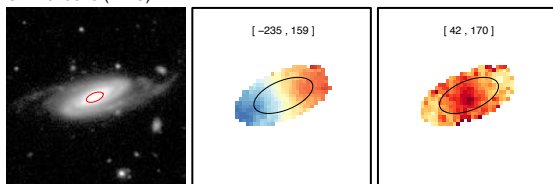

SAMI550328 (KiDS): eSp

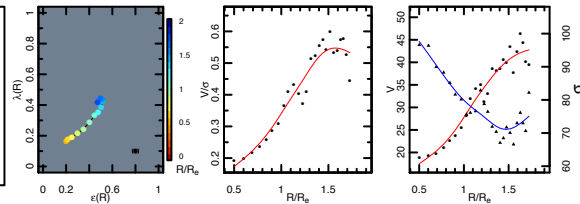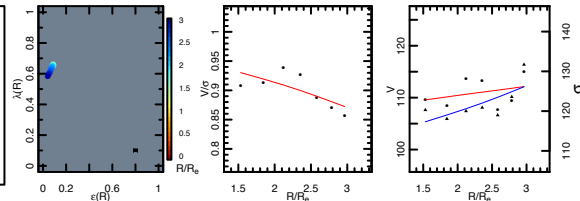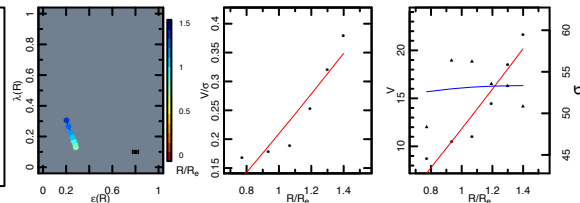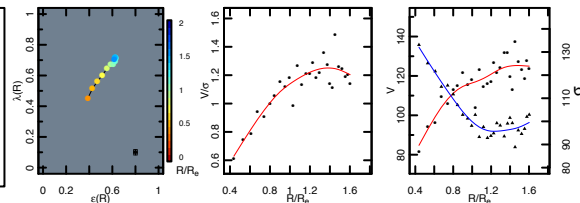

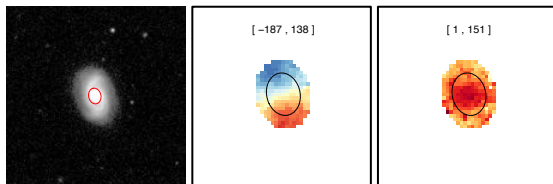

SAMI550780 (KiDS): eSp

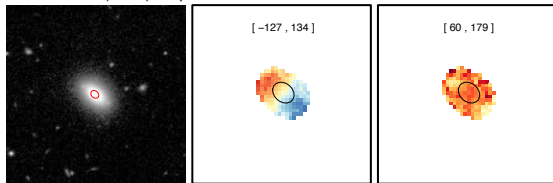

SAMI550781 (KiDS): S0

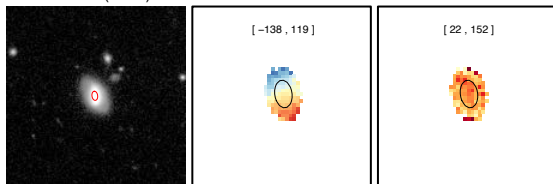

SAMI551332 (KiDS): \*ISp

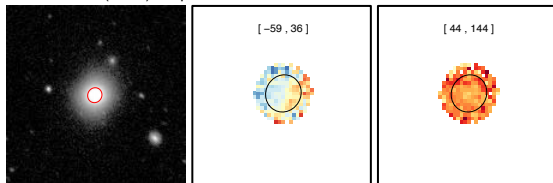

SAMI559490 (KiDS): E

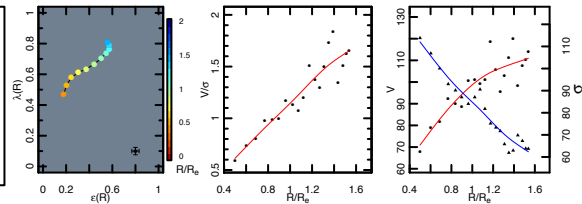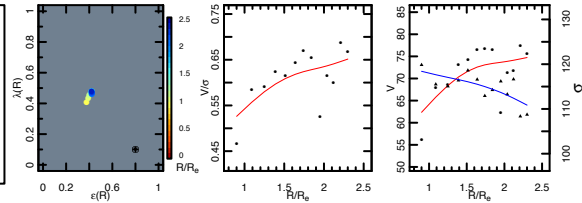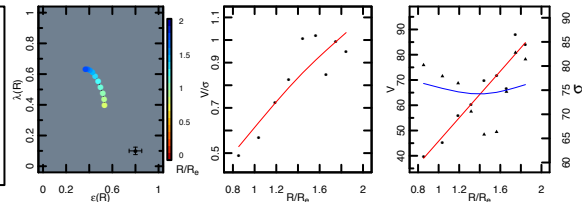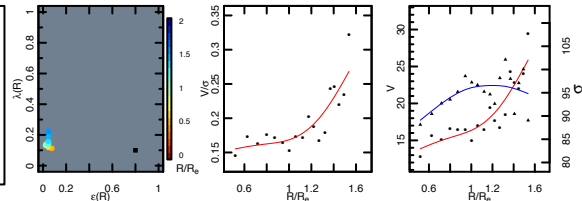

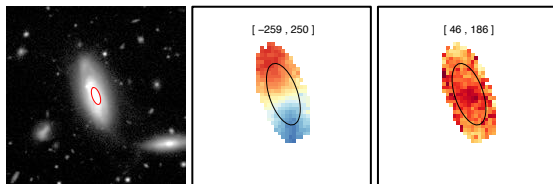

SAMI560407 (HSC): \*ISp

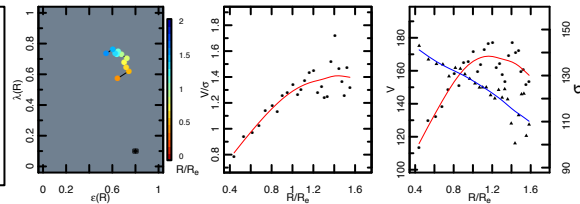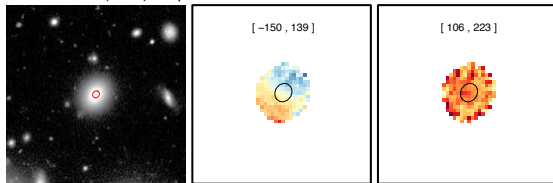

SAMI560982 (HSC): \*E

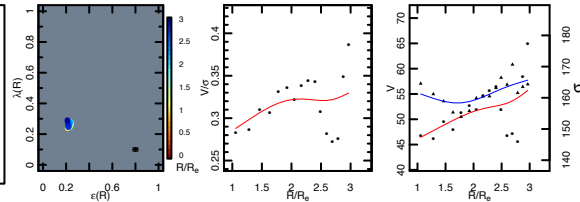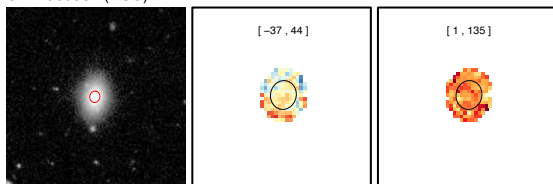

SAMI561488 (KiDS): \*S0

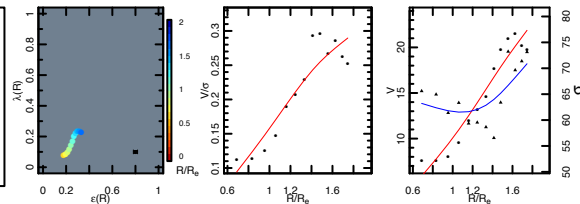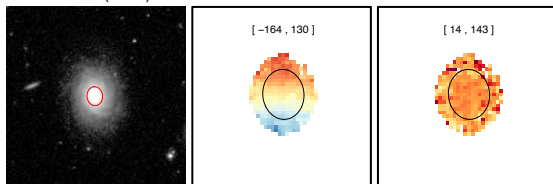

SAMI561856 (KiDS): eSp

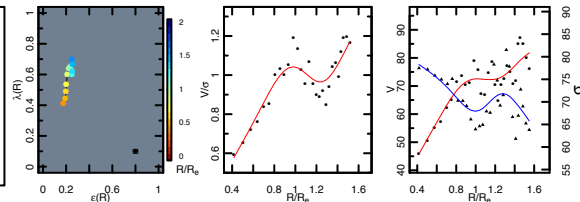

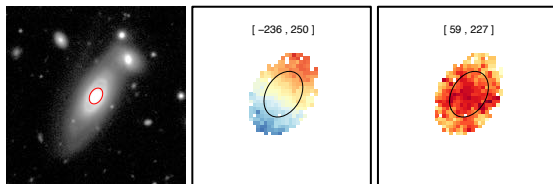

SAMI569466 (HSC): eSp

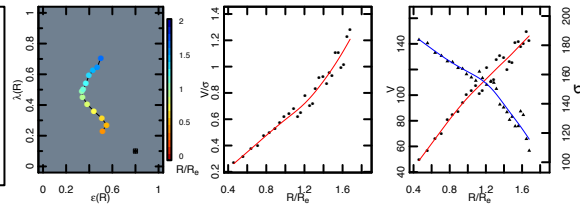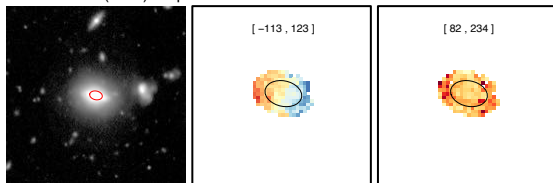

SAMI569555 (HSC): S0/eSp

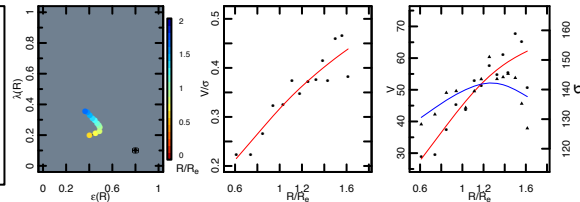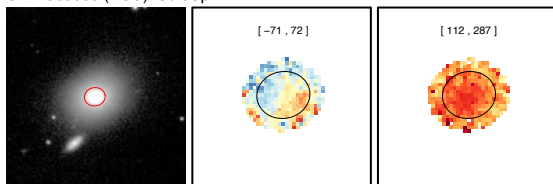

SAMI570203 (KiDS): \*E

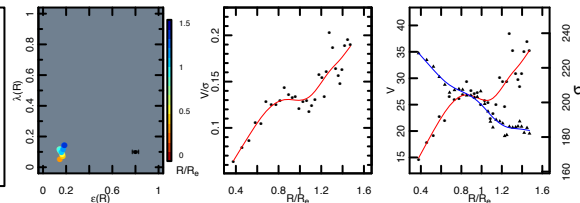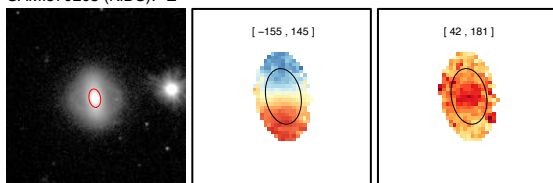

SAMI570206 (KiDS): \*eSp

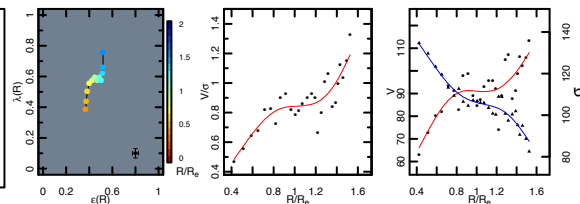



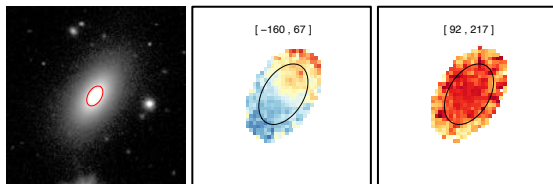

SAMI570207 (KiDS): S0

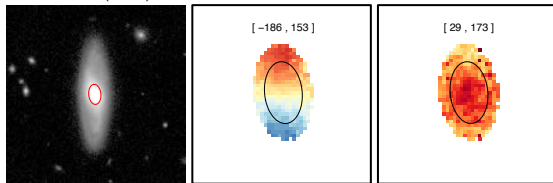

SAMI570227 (KiDS): eSp

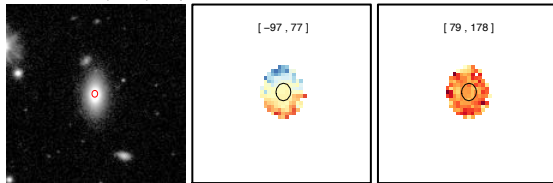

SAMI570240 (KiDS): S0

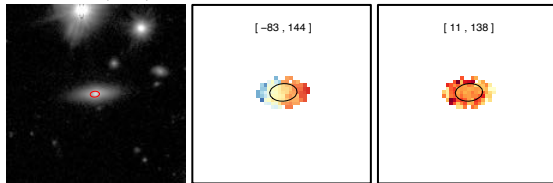

SAMI573617 (KiDS): \*S0

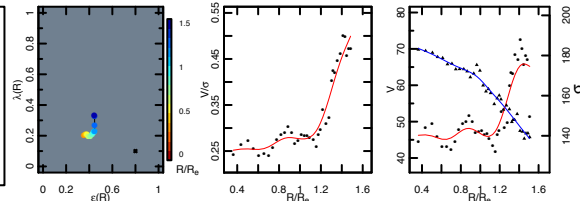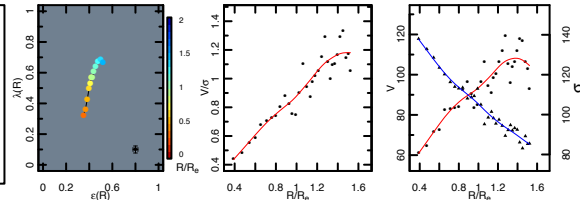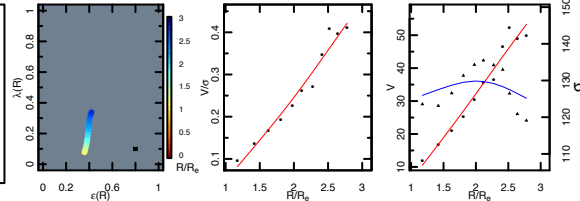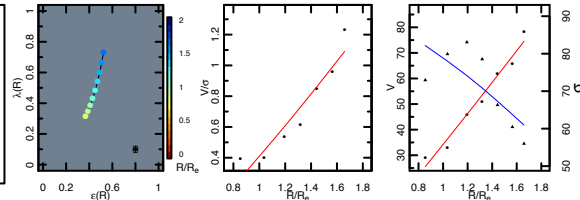

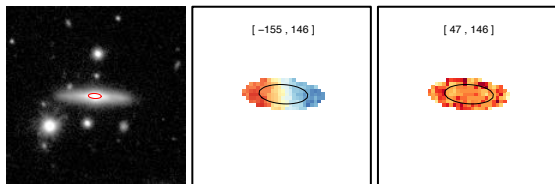

SAMI573621 (KiDS): eSp

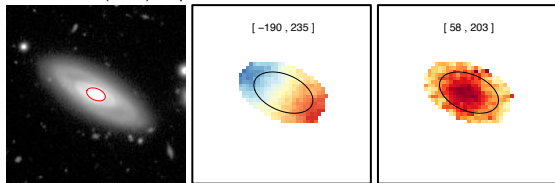

SAMI574285 (HSC): eSp

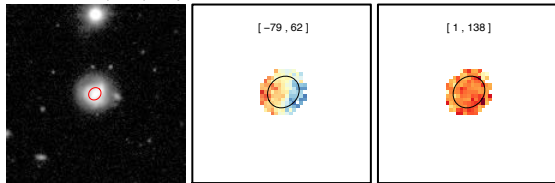

SAMI574617 (KiDS): eSp

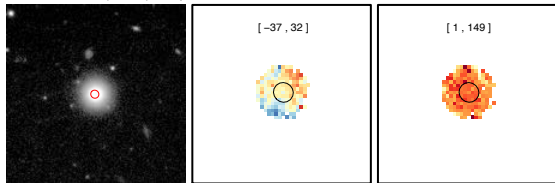

SAMI575339 (KiDS): E

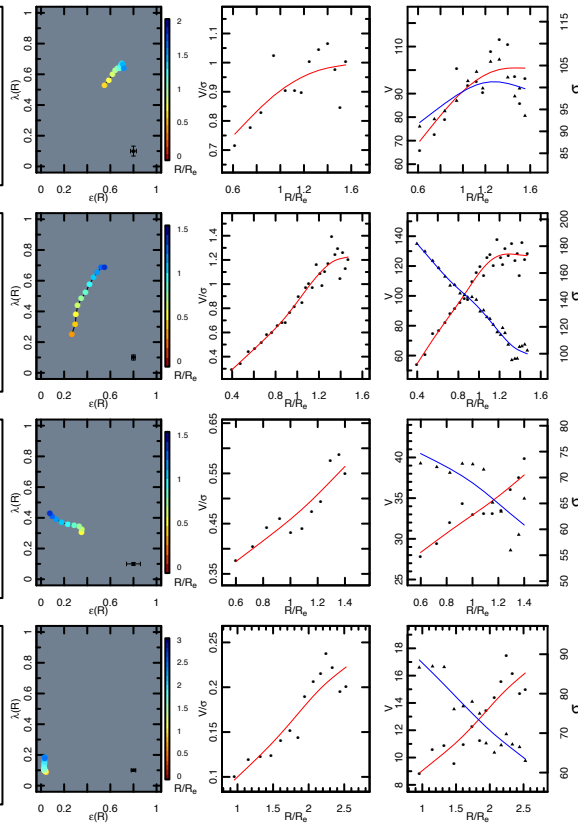

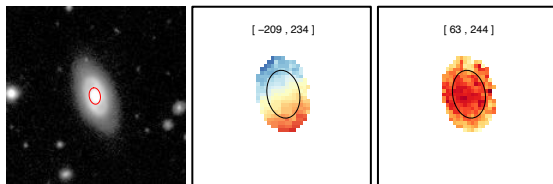

SAMI575532 (KiDS): eSp

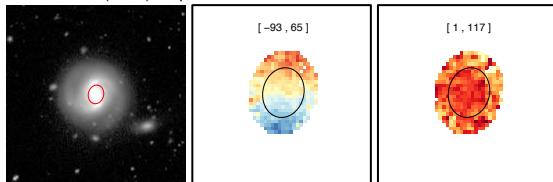

SAMI584013 (HSC): \*eSB

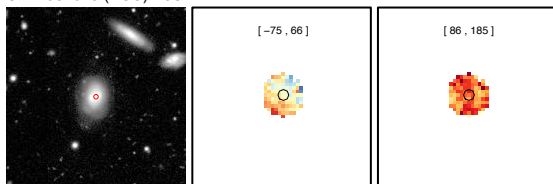

SAMI585196 (HSC): E/SO

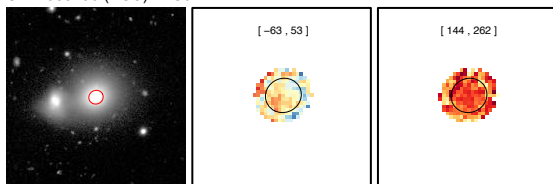

SAMI585215 (HSC): E

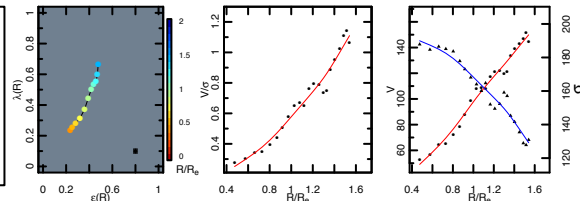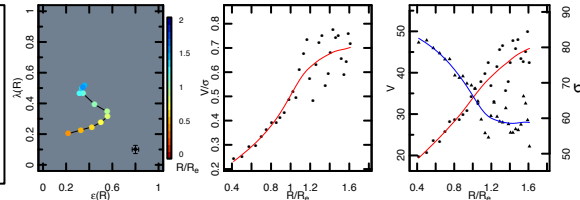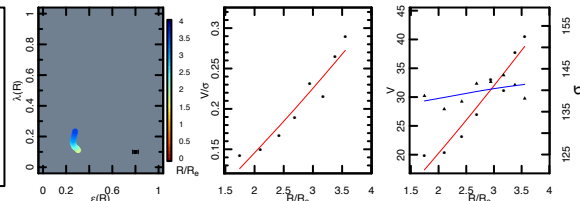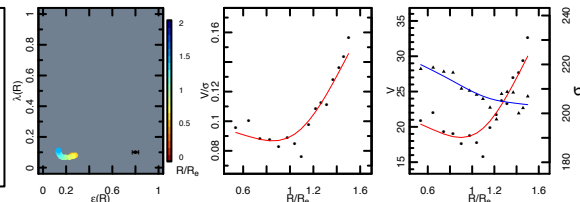

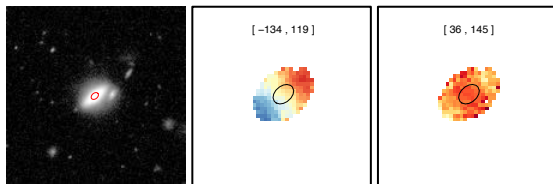

SAMI586330 (KiDS): S0

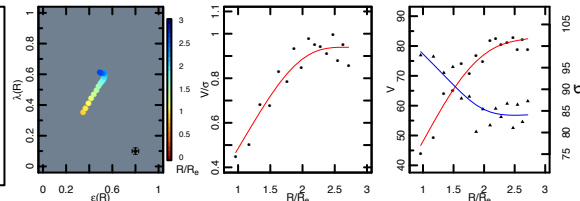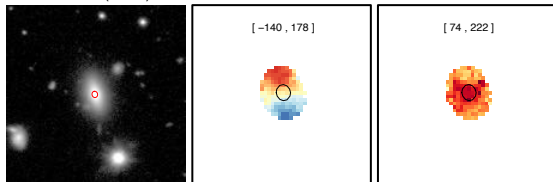

SAMI592294 (KiDS): S0

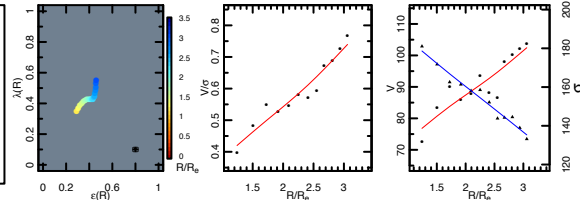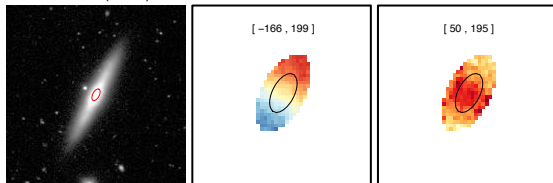

SAMI592858 (HSC): \*eSp

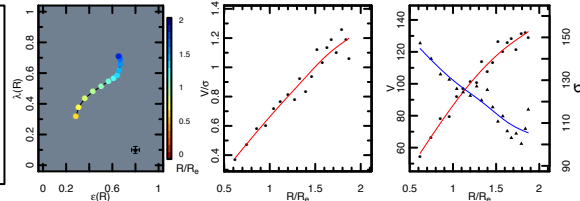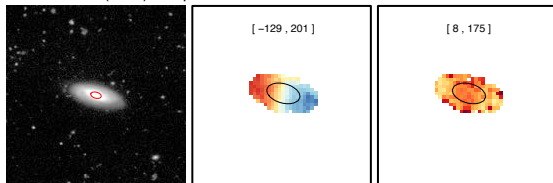

SAMI593117 (HSC): \*eSp

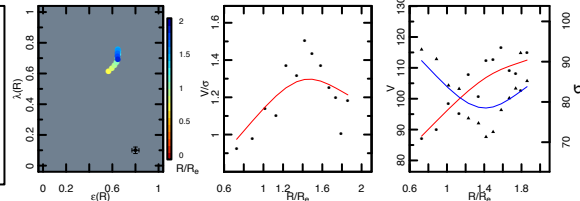

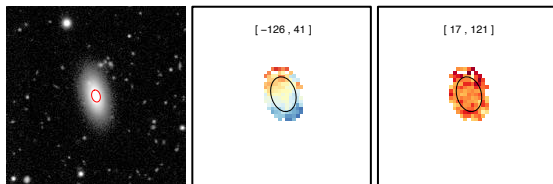

SAMI593642 (HSC): S0/eSp

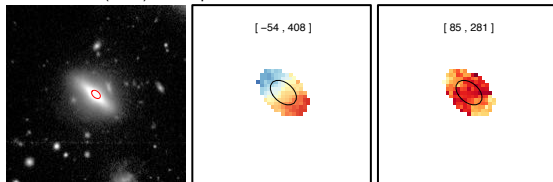

SAMI593813 (HSC): S0

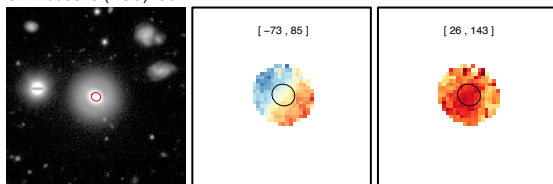

SAMI594053 (HSC): \*S0

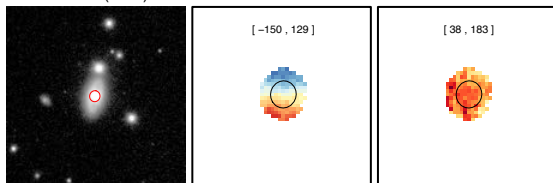

SAMI594834 (KiDS): eSp

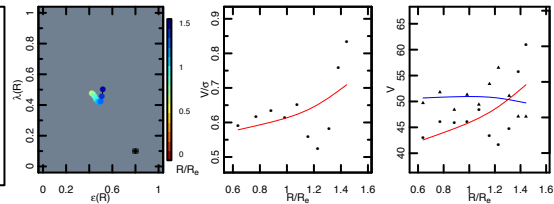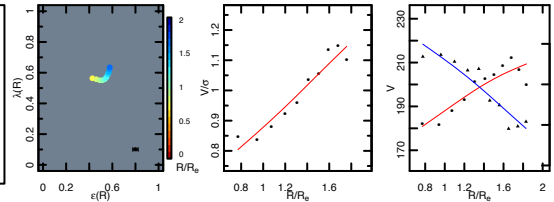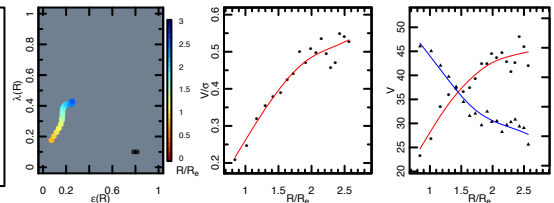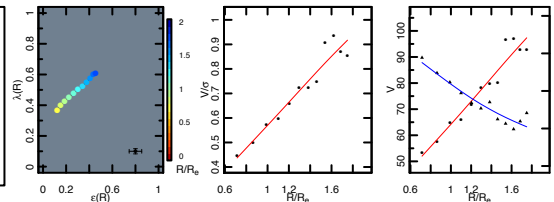

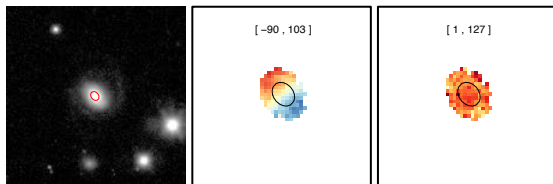

SAMI594906 (KiDS): ISp

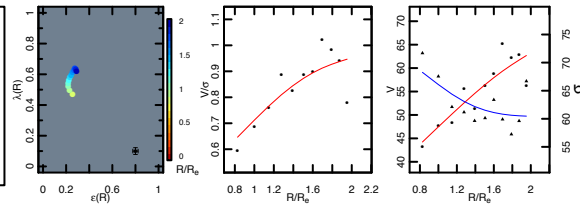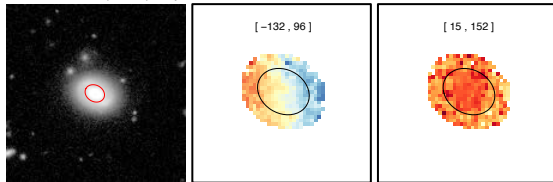

SAMI594990 (KiDS): \*S0

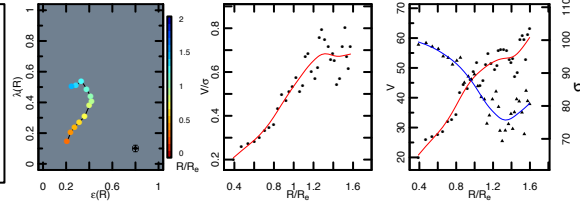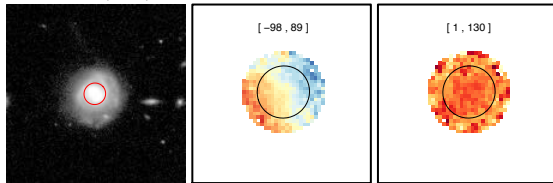

SAMI595060 (KiDS): eSp

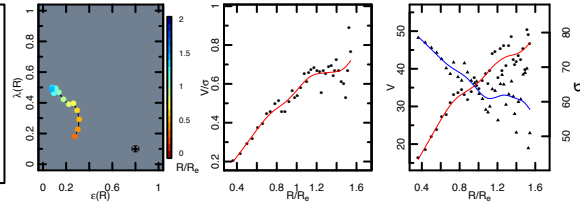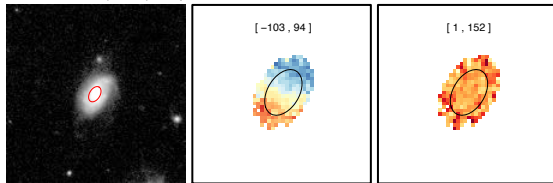

SAMI595088 (KiDS): ISp

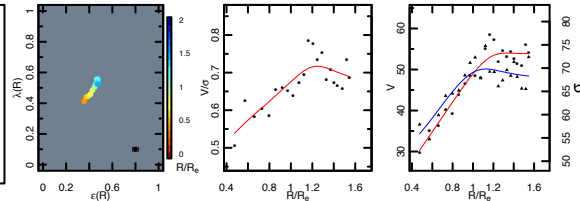

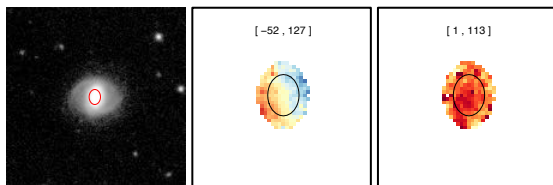

SAMI598999 (KiDS): eSp

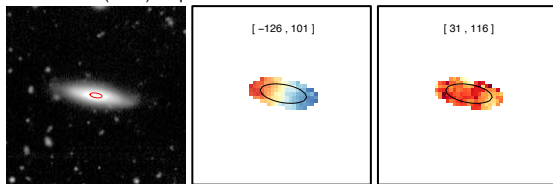

SAMI599846 (HSC): eSp/lSp

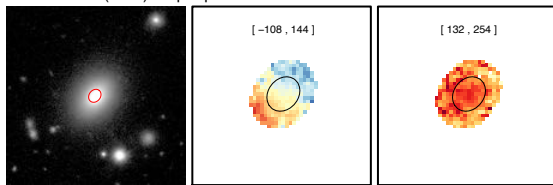

SAMI600743 (KiDS): \*S0

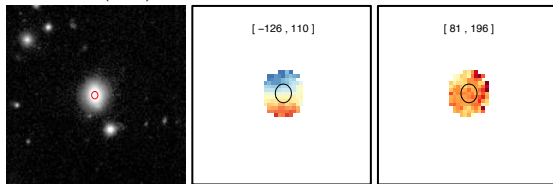

SAMI600882 (KiDS): \*S0

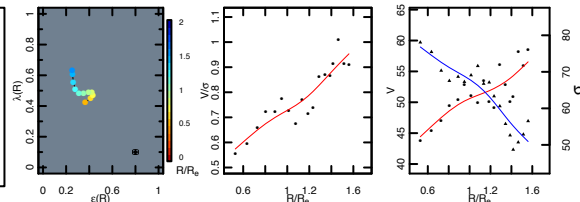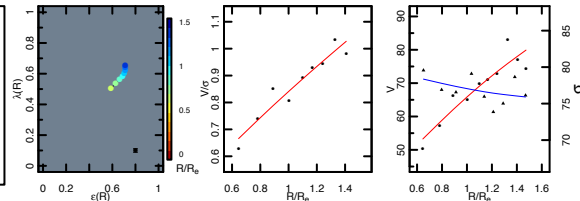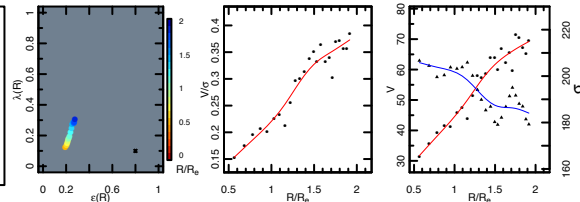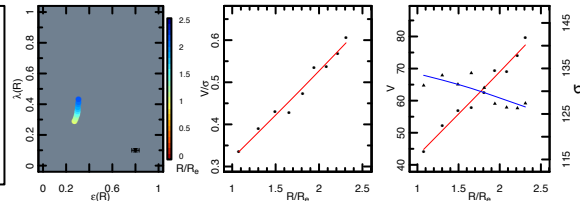

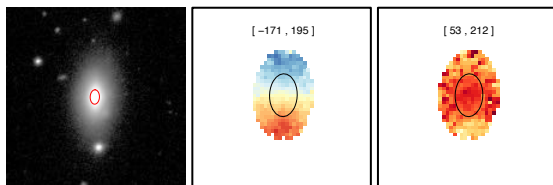

SAMI600915 (KiDS): S0

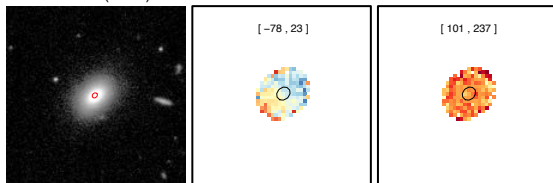

SAMI600973 (KiDS): \*E

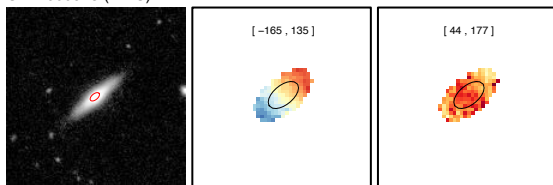

SAMI601102 (KiDS): \*S0

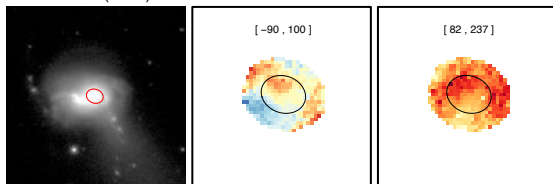

SAMI609396 (KiDS): \*ISp

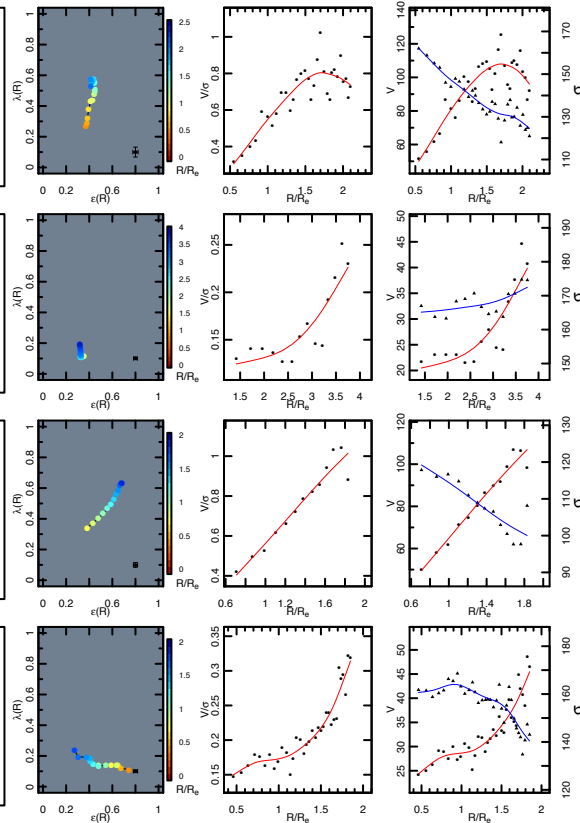



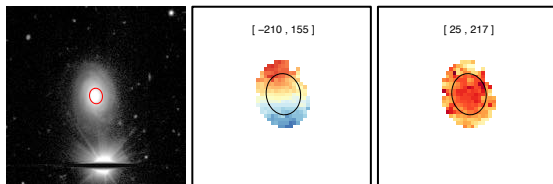

SAMI609948 (HSC): \*eSp

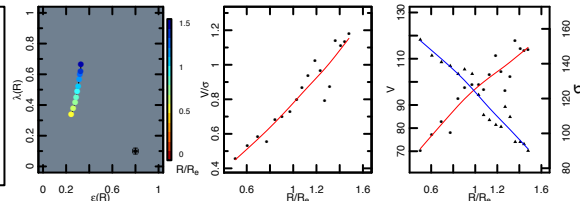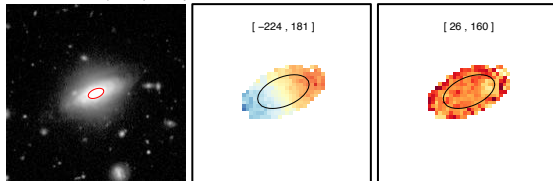

SAMI610054 (HSC): \*eSp

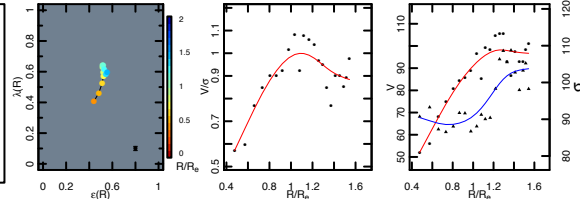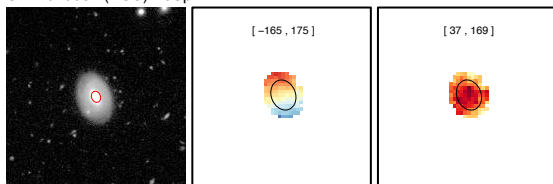

SAMI610396 (HSC): \*eSp

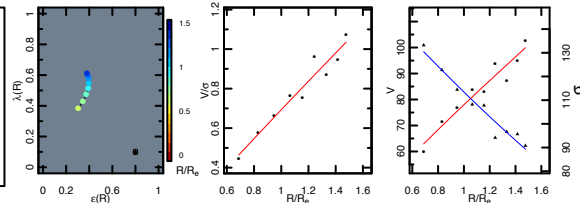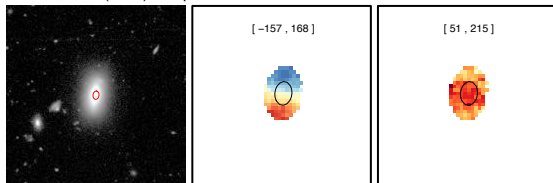

SAMI610404 (HSC): S0

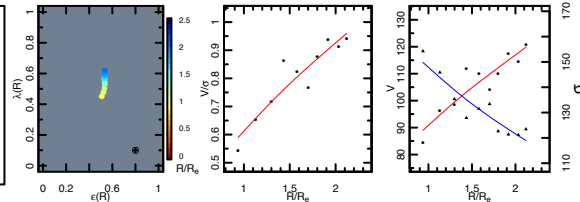

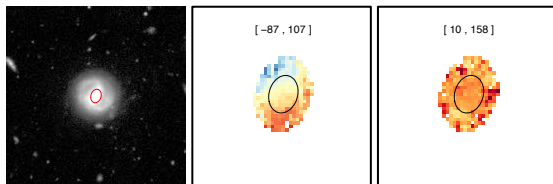

SAMI610474 (HSC): \*eSB

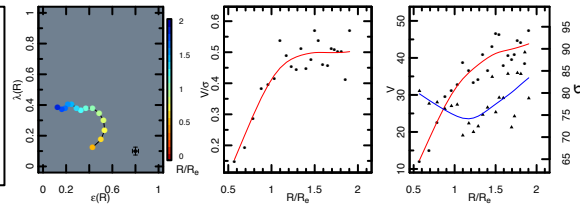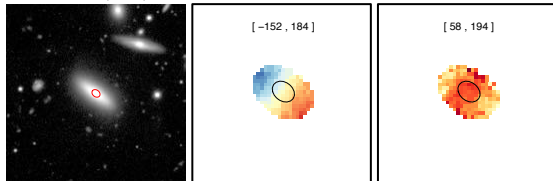

SAMI617989 (HSC): \*eSp

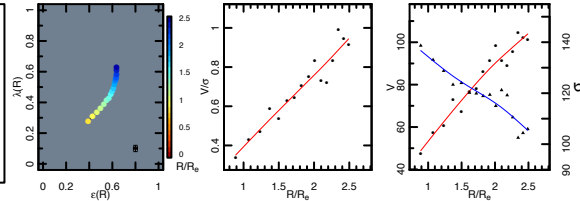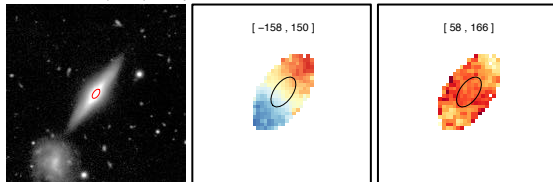

SAMI618108 (HSC): eSp

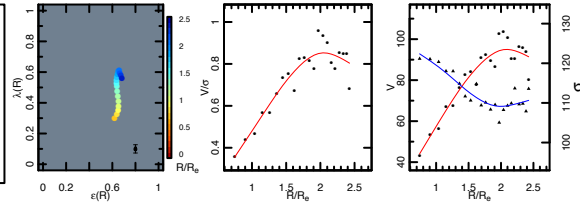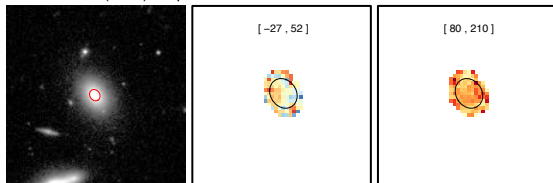

SAMI618142 (KiDS): \*E

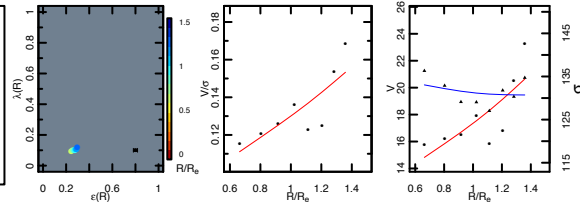

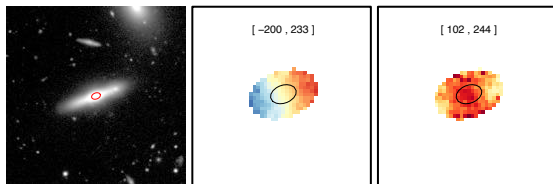

SAMI618143 (HSC): \*S0

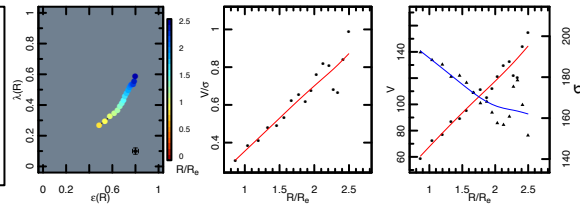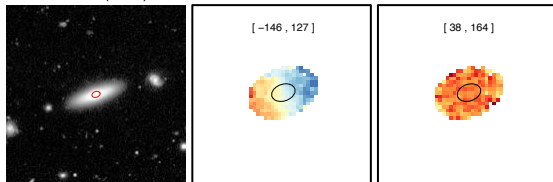

SAMI618144 (HSC): S0

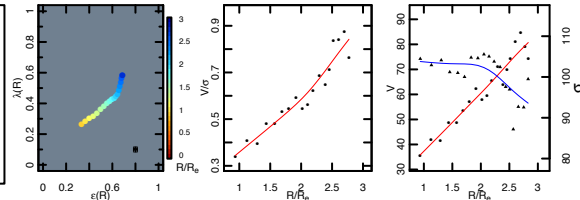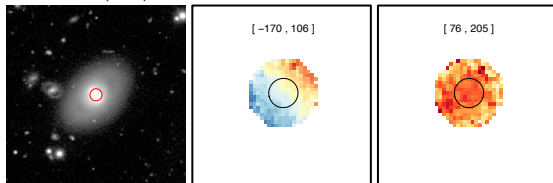

SAMI618151 (HSC): E

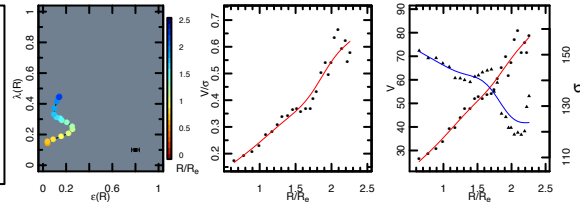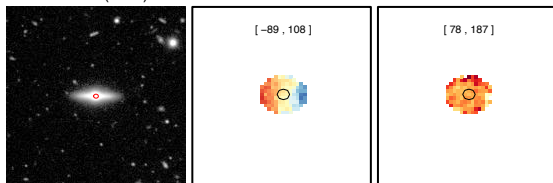

SAMI618904 (HSC): \*S0

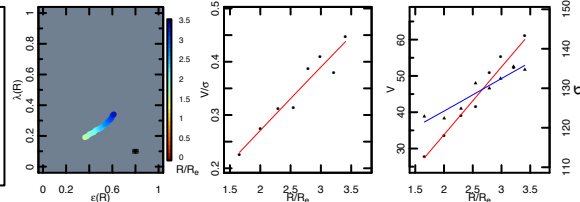

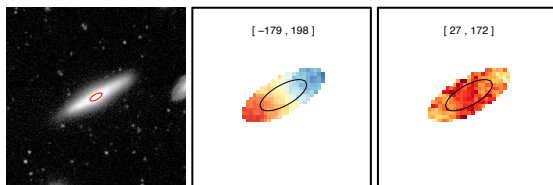

SAMI618906 (HSC): \*eSp

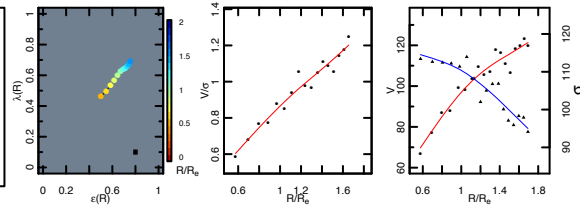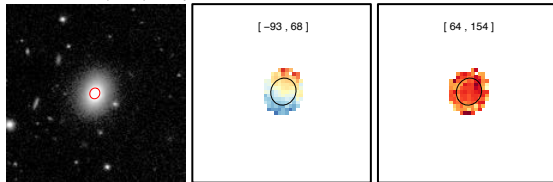

SAMI618912 (KiDS): \*E

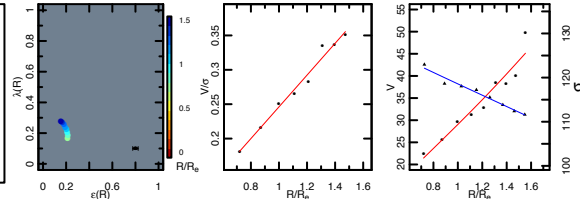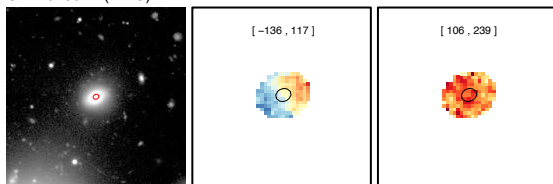

SAMI618930 (HSC): \*E

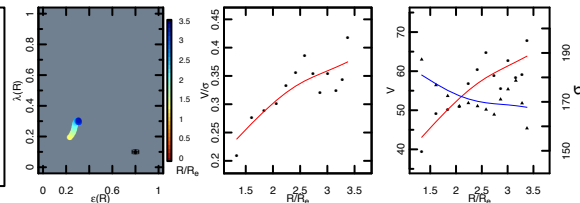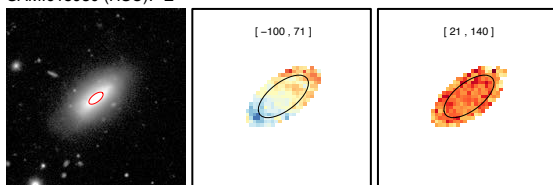

SAMI618935 (HSC): iSp

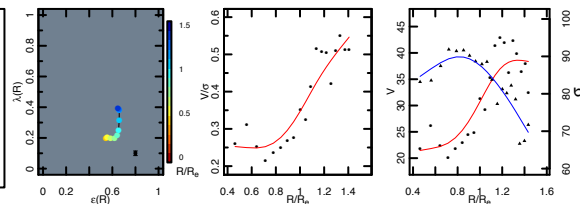

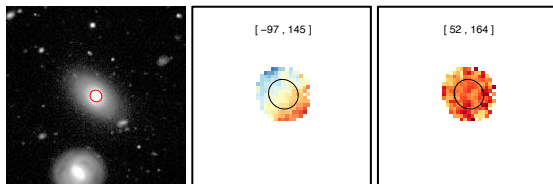

SAMI618937 (HSC): \*S0

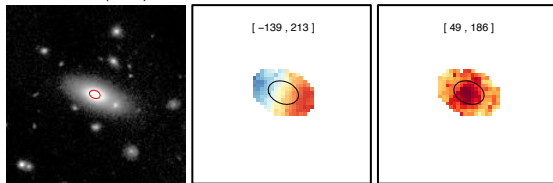

SAMI618938 (KiDS): S0

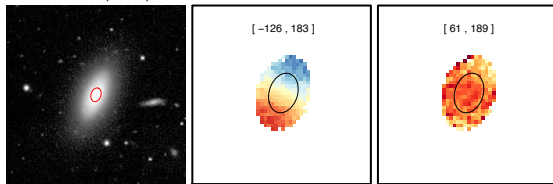

SAMI618941 (HSC): S0

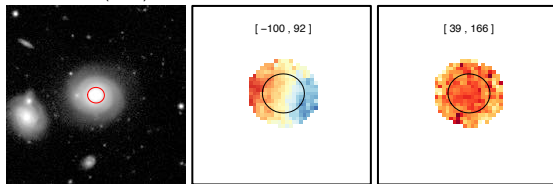

SAMI618942 (HSC): E

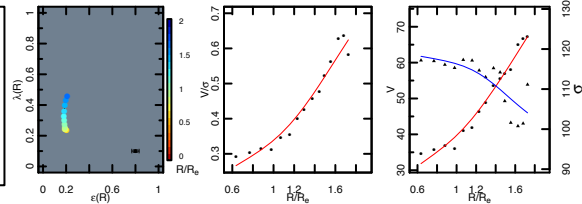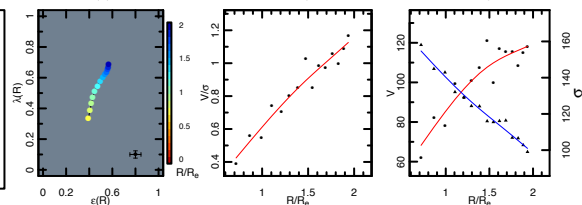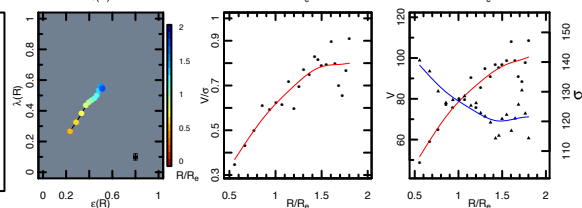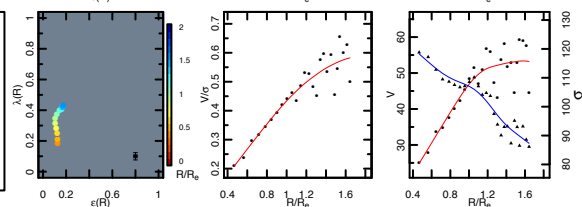

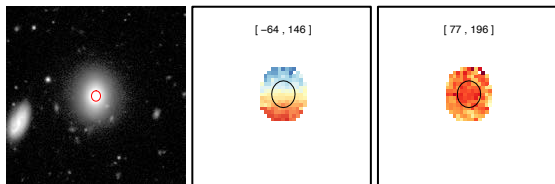

SAMI618947 (HSC): E/S0

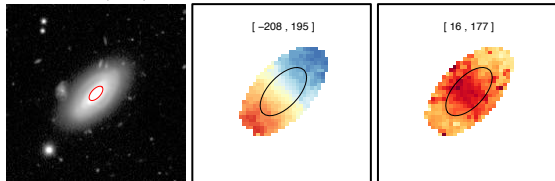

SAMI618952 (HSC): \*eSp

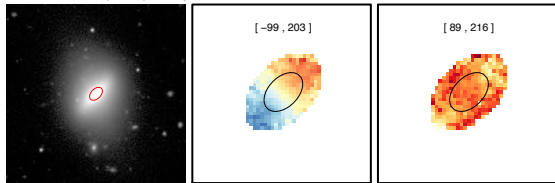

SAMI618976 (HSC): S0

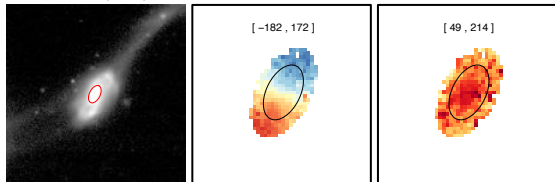

SAMI618992 (KiDS): \*Interacting

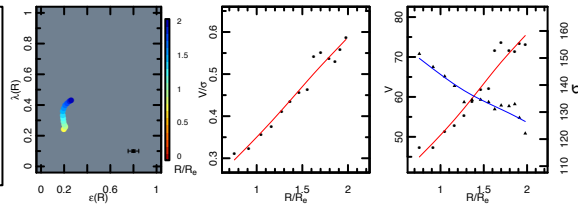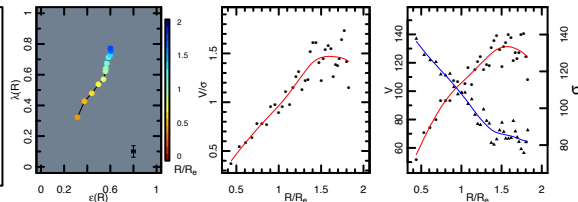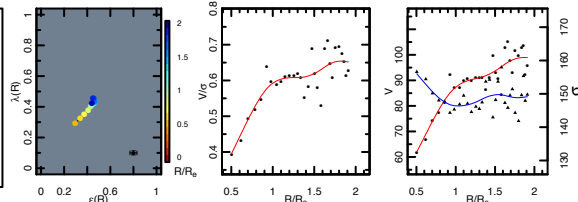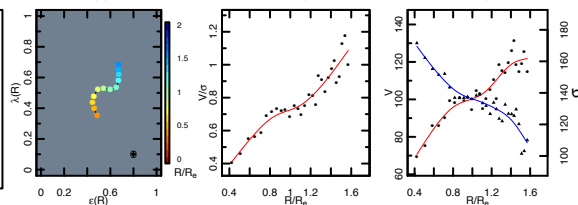

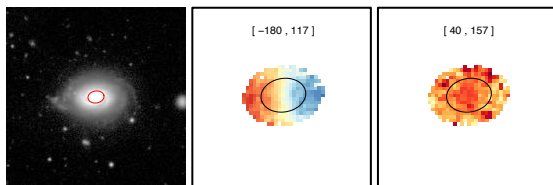

SAMI619095 (HSC): eSp/Sp

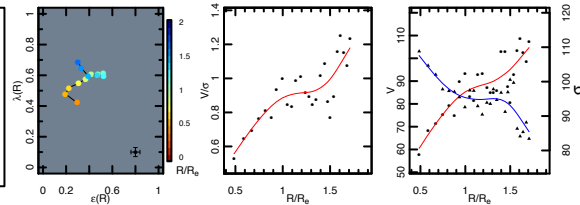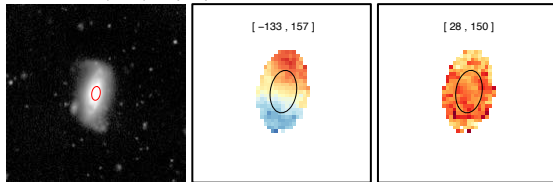

SAMI619097 (HSC): eSp

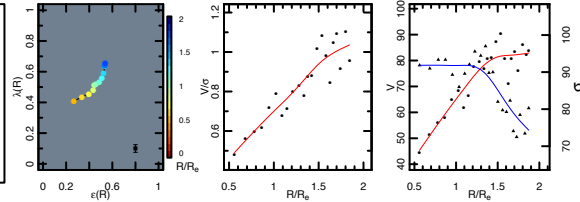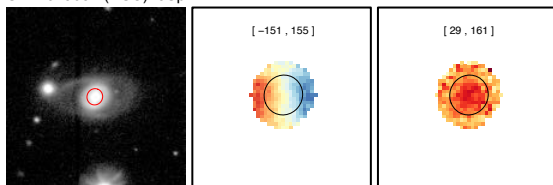

SAMI622596 (KiDS): eSp

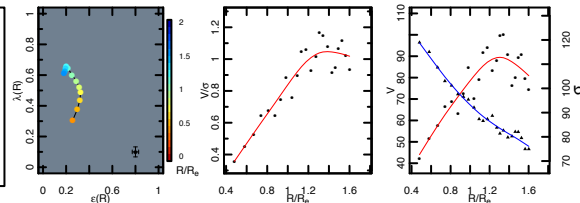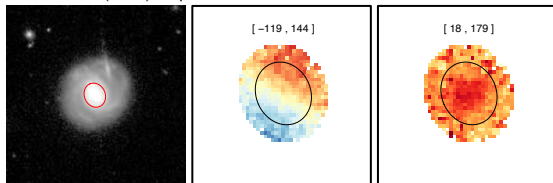

SAMI622694 (KiDS): eSp

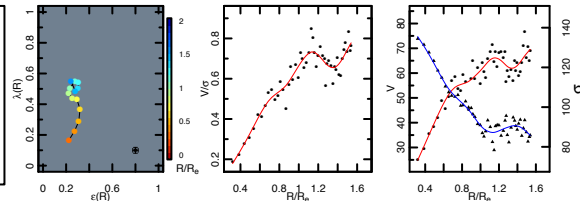

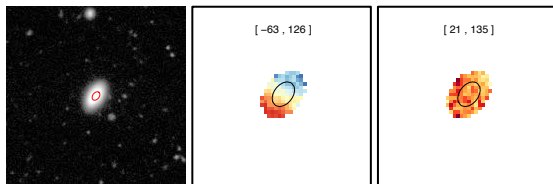

SAMI622770 (HSC): S0/eSp

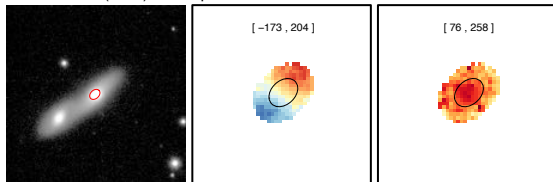

SAMI622787 (KiDS): S0

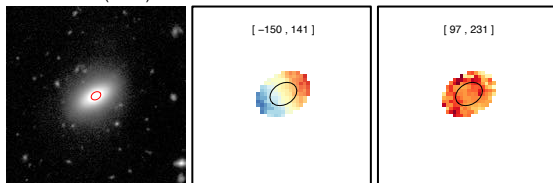

SAMI623043 (HSC): S0

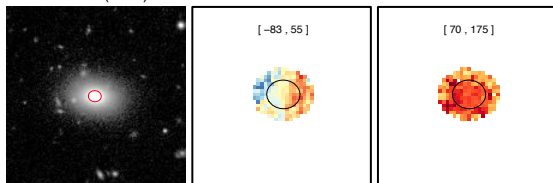

SAMI623143 (KiDS): S0/eSp

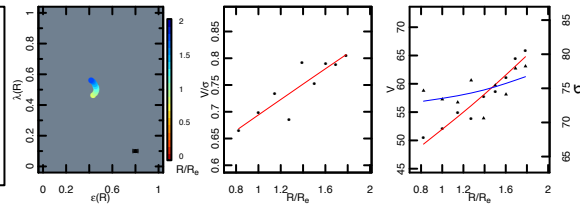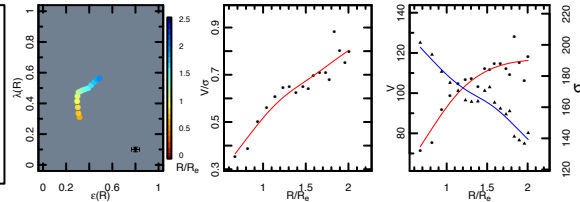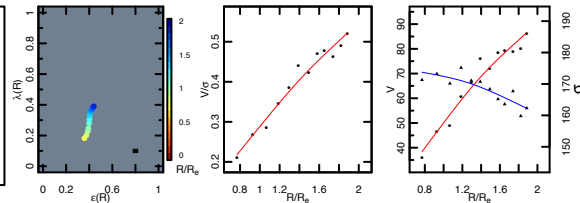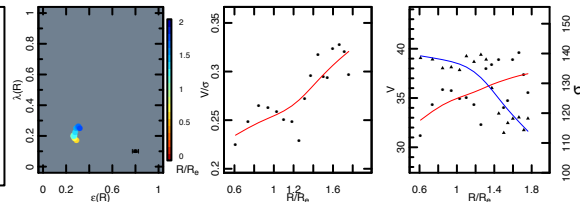



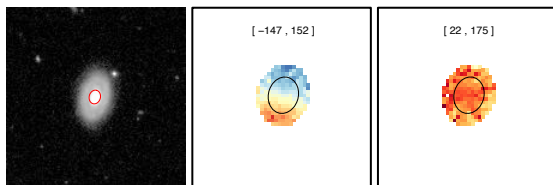

SAMI623161 (KiDS): eSp

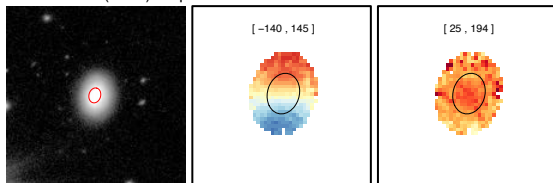

SAMI623272 (KiDS): eSp

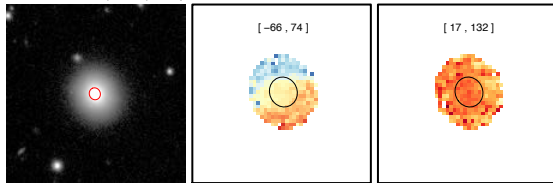

SAMI663440 (KiDS): S0

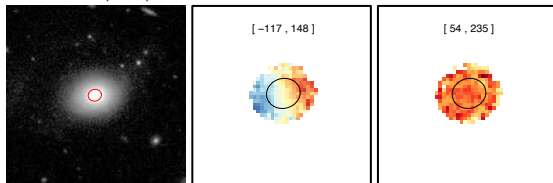

SAMI3628218 (KiDS): \*S0

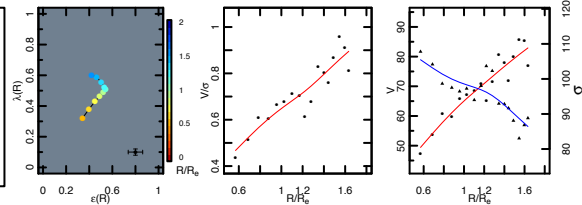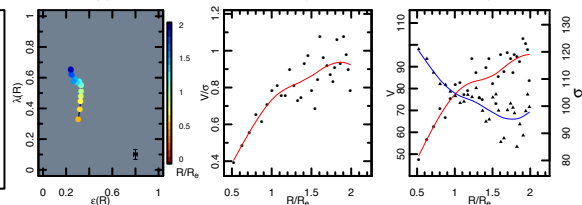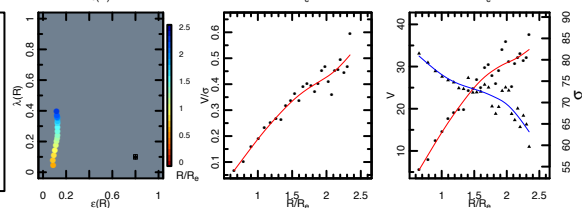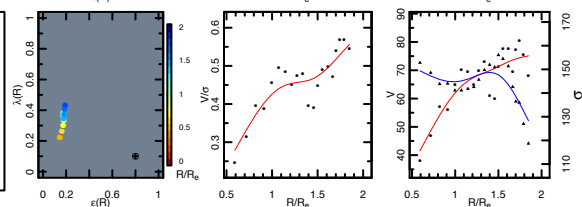

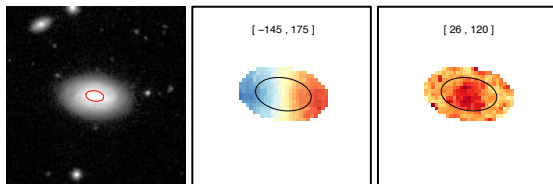

SAMI3630097 (KiDS): eSp

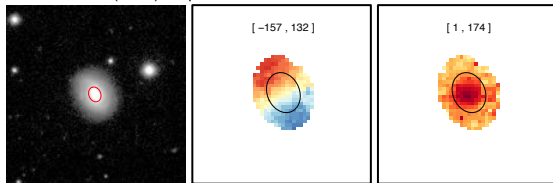

SAMI3630943 (KiDS): \*eSp

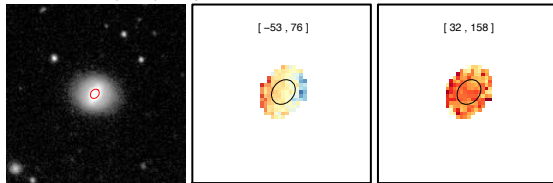

SAMI3631885 (KiDS): S0/eSp

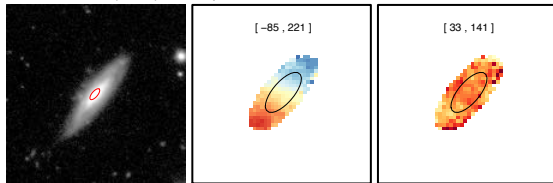

SAMI3894635 (KiDS): eSp

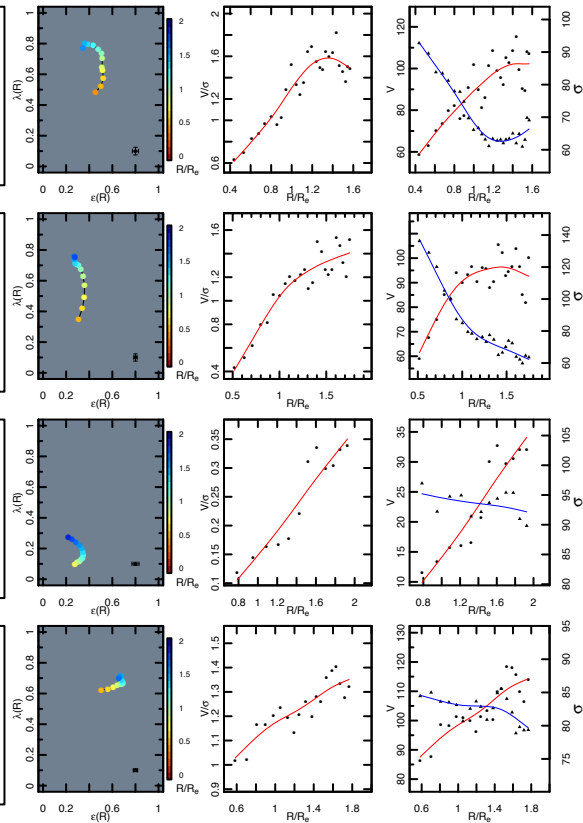

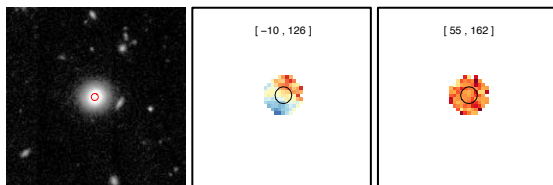

SAMI3895503 (KiDS): \*E

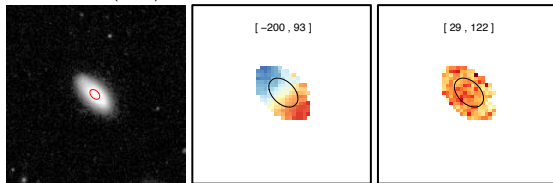

SAMI3895823 (KiDS): \*eSp

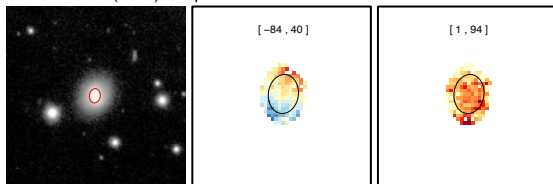

SAMI3896912 (KiDS): ISp

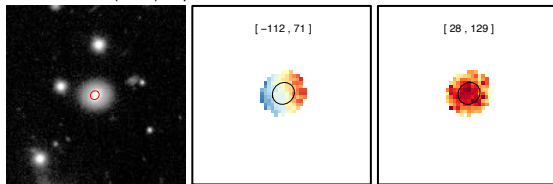

SAMI3897281 (KiDS): S0/eSp

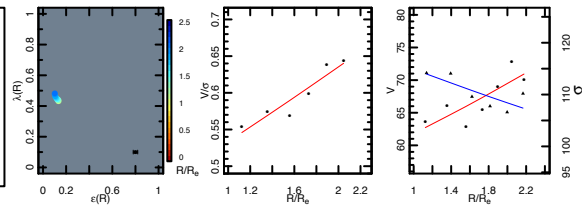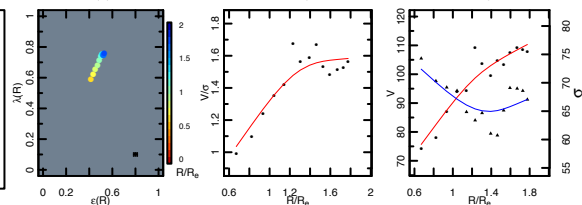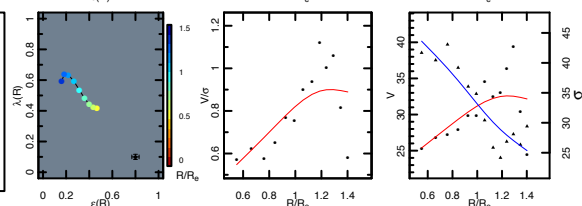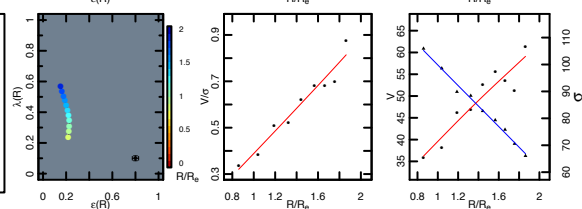

Supplement: Supplementary file 2 [file supplement_plots.pdf]
